# Supplementary material for: On the advanced integral equation theory description of dense Yukawa one-component plasma liquids
Source: arXiv:2006.11553 ancillary file (2020-07-20)
Supplement: Supplementary file 1 [file supplementary_material_full.pdf]

# On the advanced integral equation theory description of dense Yukawa one-component plasma liquids; Supplementary material

F. Lucco Castello and P. Tolias
*Space and Plasma Physics, Royal Institute of Technology, Stockholm, SE-100 44, Sweden*

Supplementary material for the manuscript entitled "On the advanced integral equation theory description of dense Yukawa one-component plasma liquids". Comparisons of structural and thermodynamic properties are carried out between the results of computer simulations (molecular dynamics, Langevin dynamics) and the results of different integral equation theory approaches (hypernetted chain approximation, isomorph-based empirically modified hypernetted-chain approximation, variational modified hypernetted-chain approximation, Rogers-Young approximation, Ballone-Pastore-Galli-Gazzillo approximation). A thermodynamic consistency test is also performed concerning the statistical and virial routes to the reduced excess inverse isothermal compressibility.

## Contents

**Tables 1a-1g**: Some key properties of the YOCP pair correlation function according to Langevin dynamics simulations and different integral equation theory approaches for $\kappa = 0$ and varying coupling parameters.
**Tables 2a-2g**: Some key properties of the YOCP pair correlation function according to Langevin dynamics simulations and different integral equation theory approaches for $\kappa = 1$ and varying coupling parameters.
**Tables 3a-3g**: Some key properties of the YOCP pair correlation function according to Langevin dynamics simulations and different integral equation theory approaches for $\kappa = 2$ and varying coupling parameters.
**Tables 4a-4d**: The YOCP reduced excess internal energy due to particle-particle interactions according to molecular dynamics simulations and different integral equation theory approaches for varying screening and coupling parameters.
**Tables 5a-5f**: The YOCP reduced excess inverse isothermal compressibility owing to the particle presence resulting from the statistical route and the virial route of different integral equation theory approaches for varying screening and coupling parameters.

**Table 1a.** Key properties of the pair correlation function resulting from Langevin dynamics simulations and five integral theory approaches: the hypernetted-chain approximation (HNC), isomorph-based empirically modified hypernetted-chain approximation (IEMHNC), variational modified hypernetted-chain approximation (VMHNC), Rogers-Young approximation (RY) and Ballone-Pastore-Galli-Gazzillo approximation (BPGG). The absolute relative deviation $\epsilon_{\mathrm{r}}$ between the theoretical and the simulation results is also reported. **Results for $\arg_r\{g(r) = 0.5\}$ in the case of $\kappa = 0$**. The LD results are adopted from Table 4 of *T. Ott and M. Bonitz, Contrib. Plasma Phys.* **55**, *243 (2015)*. Here $x = r/d$, where $d$ is the Wigner-Seitz radius.

| $\Gamma$ | $\Gamma/\Gamma_{\mathrm{m}}$ | $x_{\mathrm{cv}}^{\mathrm{LD}}$ | $x_{\mathrm{cv}}^{\mathrm{HNC}}$ | $\epsilon_{\mathrm{HNC}}(\%)$ | $x_{\mathrm{cv}}^{\mathrm{IEMHNC}}$ | $\epsilon_{\mathrm{IEMHNC}}(\%)$ | $x_{\mathrm{cv}}^{\mathrm{VMHNC}}$ | $\epsilon_{\mathrm{VMHNC}}(\%)$ | $x_{\mathrm{cv}}^{\mathrm{RY}}$ | $\epsilon_{\mathrm{RY}}(\%)$ | $x_{\mathrm{cv}}^{\mathrm{BPGG}}$ | $\epsilon_{\mathrm{BPGG}}(\%)$ |
|---|---|---|---|---|---|---|---|---|---|---|---|---|
| 15.0 | 0.09 | 1.179 | 1.150 | 2.460 | 1.165 | 1.187 | 1.176 | 0.254 | 1.169 | 0.848 | 1.150 | 2.460 |
| 20.0 | 0.12 | 1.218 | 1.187 | 2.545 | 1.207 | 0.903 | 1.217 | 0.082 | 1.206 | 0.985 | 1.187 | 2.545 |
| 25.0 | 0.15 | 1.246 | 1.214 | 2.568 | 1.237 | 0.722 | 1.247 | 0.080 | 1.234 | 0.963 | 1.214 | 2.568 |
| 30.0 | 0.17 | 1.272 | 1.235 | 2.909 | 1.262 | 0.786 | 1.271 | 0.079 | 1.257 | 1.179 | 1.235 | 2.909 |
| 35.0 | 0.20 | 1.291 | 1.253 | 2.943 | 1.282 | 0.697 | 1.291 | 0.000 | 1.275 | 1.239 | 1.253 | 2.943 |
| 40.0 | 0.23 | 1.307 | 1.268 | 2.984 | 1.299 | 0.612 | 1.307 | 0.000 | 1.290 | 1.301 | 1.268 | 2.984 |
| 45.0 | 0.26 | 1.320 | 1.282 | 2.879 | 1.314 | 0.455 | 1.322 | 0.152 | 1.304 | 1.212 | 1.282 | 2.879 |
| 50.0 | 0.29 | 1.333 | 1.293 | 3.001 | 1.327 | 0.450 | 1.335 | 0.150 | 1.316 | 1.275 | 1.293 | 3.001 |
| 55.0 | 0.32 | 1.346 | 1.304 | 3.120 | 1.338 | 0.594 | 1.346 | 0.000 | 1.326 | 1.486 | 1.304 | 3.120 |
| 60.0 | 0.35 | 1.355 | 1.313 | 3.100 | 1.349 | 0.443 | 1.356 | 0.074 | 1.336 | 1.402 | 1.313 | 3.100 |
| 65.0 | 0.38 | 1.365 | 1.322 | 3.150 | 1.359 | 0.440 | 1.366 | 0.073 | 1.345 | 1.465 | 1.322 | 3.150 |
| 70.0 | 0.41 | 1.374 | 1.330 | 3.202 | 1.367 | 0.509 | 1.374 | 0.000 | 1.353 | 1.528 | 1.330 | 3.202 |
| 75.0 | 0.44 | 1.381 | 1.337 | 3.186 | 1.376 | 0.362 | 1.382 | 0.072 | 1.360 | 1.521 | 1.337 | 3.186 |
| 80.0 | 0.47 | 1.387 | 1.344 | 3.100 | 1.383 | 0.288 | 1.390 | 0.216 | 1.367 | 1.442 | 1.344 | 3.100 |
| 85.0 | 0.49 | 1.394 | 1.350 | 3.156 | 1.390 | 0.287 | 1.396 | 0.143 | 1.374 | 1.435 | 1.350 | 3.156 |
| 90.0 | 0.52 | 1.400 | 1.356 | 3.143 | 1.397 | 0.214 | 1.403 | 0.214 | 1.380 | 1.429 | 1.356 | 3.143 |
| 95.0 | 0.55 | 1.406 | 1.362 | 3.129 | 1.403 | 0.213 | 1.409 | 0.213 | 1.385 | 1.494 | 1.362 | 3.129 |
| 100.0 | 0.58 | 1.413 | 1.367 | 3.255 | 1.409 | 0.283 | 1.414 | 0.071 | 1.391 | 1.557 | 1.367 | 3.255 |
| 105.0 | 0.61 | 1.419 | 1.372 | 3.312 | 1.415 | 0.282 | 1.420 | 0.070 | 1.396 | 1.621 | 1.372 | 3.312 |
| 110.0 | 0.64 | 1.422 | 1.376 | 3.235 | 1.420 | 0.141 | 1.425 | 0.211 | 1.400 | 1.547 | 1.377 | 3.165 |
| 115.0 | 0.67 | 1.429 | 1.381 | 3.359 | 1.425 | 0.280 | 1.429 | 0.000 | 1.405 | 1.679 | 1.381 | 3.359 |
| 120.0 | 0.70 | 1.432 | 1.385 | 3.282 | 1.430 | 0.140 | 1.434 | 0.140 | 1.409 | 1.606 | 1.385 | 3.282 |
| 125.0 | 0.73 | 1.435 | 1.389 | 3.206 | 1.434 | 0.070 | 1.438 | 0.209 | 1.413 | 1.533 | 1.389 | 3.206 |
| 130.0 | 0.76 | 1.442 | 1.393 | 3.398 | 1.439 | 0.208 | 1.442 | 0.000 | 1.417 | 1.734 | 1.393 | 3.398 |
| 135.0 | 0.79 | 1.445 | 1.397 | 3.322 | 1.443 | 0.138 | 1.446 | 0.069 | 1.421 | 1.661 | 1.397 | 3.322 |
| 140.0 | 0.81 | 1.448 | 1.401 | 3.246 | 1.447 | 0.069 | 1.450 | 0.138 | 1.425 | 1.588 | 1.401 | 3.246 |
| 145.0 | 0.84 | 1.451 | 1.404 | 3.239 | 1.451 | 0.000 | 1.454 | 0.207 | 1.428 | 1.585 | 1.404 | 3.239 |
| 150.0 | 0.87 | 1.454 | 1.407 | 3.232 | 1.455 | 0.069 | 1.457 | 0.206 | 1.431 | 1.582 | 1.407 | 3.232 |
| 155.0 | 0.90 | 1.461 | 1.411 | 3.422 | 1.458 | 0.205 | 1.461 | 0.000 | 1.435 | 1.780 | 1.411 | 3.422 |
| 160.0 | 0.93 | 1.464 | 1.414 | 3.415 | 1.462 | 0.137 | 1.464 | 0.000 | 1.438 | 1.776 | 1.414 | 3.415 |
| 165.0 | 0.96 | 1.467 | 1.417 | 3.408 | 1.465 | 0.136 | 1.467 | 0.000 | 1.441 | 1.772 | 1.417 | 3.408 |

**Table 1b.** Key properties of the pair correlation function resulting from Langevin dynamics simulations and five integral theory approaches: the hypernetted-chain approximation (HNC), isomorph-based empirically modified hypernetted-chain approximation (IEMHNC), variational modified hypernetted-chain approximation (VMHNC), Rogers-Young approximation (RY) and Ballone-Pastore-Galli-Gazzillo approximation (BPGG). The absolute relative deviation $\epsilon_{\mathrm{r}}$ between the theoretical and the simulation results is also reported. **Results for the magnitude of the first maximum in the case of $\boldsymbol{\kappa = 0}$**. The LD results are adopted from Table 4 of *T. Ott and M. Bonitz, Contrib. Plasma Phys.* **55**, *243 (2015).*

| $\Gamma$ | $\Gamma/\Gamma_{\mathrm{m}}$ | $g_{\mathrm{max1}}^{\mathrm{LD}}$ | $g_{\mathrm{max1}}^{\mathrm{HNC}}$ | $\epsilon_{\mathrm{HNC}}(\%)$ | $g_{\mathrm{max1}}^{\mathrm{IEMHNC}}$ | $\epsilon_{\mathrm{IEMHNC}}(\%)$ | $g_{\mathrm{max1}}^{\mathrm{VMHNC}}$ | $\epsilon_{\mathrm{VMHNC}}(\%)$ | $g_{\mathrm{max1}}^{\mathrm{RY}}$ | $\epsilon_{\mathrm{RY}}(\%)$ | $g_{\mathrm{max1}}^{\mathrm{BPGG}}$ | $\epsilon_{\mathrm{BPGG}}(\%)$ |
|---|---|---|---|---|---|---|---|---|---|---|---|---|
| 15.0 | 0.09 | 1.228 | 1.173 | 4.458 | 1.200 | 2.269 | 1.228 | 0.023 | 1.208 | 1.656 | 1.173 | 4.454 |
| 20.0 | 0.12 | 1.307 | 1.234 | 5.618 | 1.277 | 2.330 | 1.312 | 0.345 | 1.278 | 2.193 | 1.234 | 5.614 |
| 25.0 | 0.15 | 1.378 | 1.288 | 6.558 | 1.348 | 2.204 | 1.387 | 0.670 | 1.341 | 2.660 | 1.288 | 6.554 |
| 30.0 | 0.17 | 1.443 | 1.337 | 7.359 | 1.414 | 2.041 | 1.457 | 0.941 | 1.399 | 3.084 | 1.337 | 7.356 |
| 35.0 | 0.20 | 1.504 | 1.382 | 8.105 | 1.475 | 1.931 | 1.521 | 1.116 | 1.451 | 3.520 | 1.382 | 8.101 |
| 40.0 | 0.23 | 1.560 | 1.424 | 8.702 | 1.533 | 1.759 | 1.581 | 1.331 | 1.500 | 3.852 | 1.424 | 8.699 |
| 45.0 | 0.26 | 1.614 | 1.464 | 9.307 | 1.587 | 1.677 | 1.637 | 1.438 | 1.546 | 4.232 | 1.464 | 9.304 |
| 50.0 | 0.29 | 1.664 | 1.501 | 9.790 | 1.639 | 1.528 | 1.691 | 1.601 | 1.589 | 4.513 | 1.501 | 9.787 |
| 55.0 | 0.32 | 1.712 | 1.537 | 10.251 | 1.688 | 1.410 | 1.741 | 1.722 | 1.630 | 4.795 | 1.537 | 10.248 |
| 60.0 | 0.35 | 1.757 | 1.570 | 10.627 | 1.735 | 1.246 | 1.790 | 1.883 | 1.669 | 5.009 | 1.570 | 10.625 |
| 65.0 | 0.38 | 1.803 | 1.603 | 11.115 | 1.781 | 1.244 | 1.837 | 1.867 | 1.706 | 5.357 | 1.603 | 11.113 |
| 70.0 | 0.41 | 1.845 | 1.634 | 11.456 | 1.824 | 1.113 | 1.881 | 1.977 | 1.742 | 5.564 | 1.634 | 11.454 |
| 75.0 | 0.44 | 1.885 | 1.664 | 11.750 | 1.867 | 0.957 | 1.925 | 2.106 | 1.777 | 5.732 | 1.664 | 11.748 |
| 80.0 | 0.47 | 1.926 | 1.692 | 12.130 | 1.908 | 0.926 | 1.966 | 2.101 | 1.810 | 6.004 | 1.692 | 12.128 |
| 85.0 | 0.49 | 1.964 | 1.720 | 12.409 | 1.948 | 0.802 | 2.007 | 2.187 | 1.843 | 6.177 | 1.720 | 12.407 |
| 90.0 | 0.52 | 2.001 | 1.747 | 12.676 | 1.987 | 0.686 | 2.046 | 2.261 | 1.874 | 6.345 | 1.747 | 12.675 |
| 95.0 | 0.55 | 2.037 | 1.774 | 12.930 | 2.025 | 0.573 | 2.084 | 2.328 | 1.904 | 6.506 | 1.774 | 12.928 |
| 100.0 | 0.58 | 2.072 | 1.799 | 13.167 | 2.063 | 0.457 | 2.122 | 2.394 | 1.934 | 6.656 | 1.799 | 13.165 |
| 105.0 | 0.61 | 2.107 | 1.824 | 13.428 | 2.099 | 0.385 | 2.158 | 2.413 | 1.963 | 6.837 | 1.824 | 13.426 |
| 110.0 | 0.64 | 2.140 | 1.848 | 13.629 | 2.134 | 0.258 | 2.193 | 2.488 | 1.991 | 6.959 | 1.848 | 13.627 |
| 115.0 | 0.67 | 2.174 | 1.872 | 13.890 | 2.169 | 0.213 | 2.228 | 2.475 | 2.019 | 7.151 | 1.872 | 13.888 |
| 120.0 | 0.70 | 2.206 | 1.895 | 14.089 | 2.204 | 0.110 | 2.262 | 2.522 | 2.045 | 7.281 | 1.895 | 14.087 |
| 125.0 | 0.73 | 2.237 | 1.918 | 14.266 | 2.237 | 0.008 | 2.295 | 2.581 | 2.072 | 7.391 | 1.918 | 14.265 |
| 130.0 | 0.76 | 2.270 | 1.940 | 14.535 | 2.270 | 0.007 | 2.327 | 2.518 | 2.097 | 7.604 | 1.940 | 14.534 |
| 135.0 | 0.79 | 2.298 | 1.962 | 14.631 | 2.303 | 0.199 | 2.359 | 2.653 | 2.123 | 7.633 | 1.962 | 14.630 |
| 140.0 | 0.81 | 2.329 | 1.983 | 14.852 | 2.334 | 0.234 | 2.390 | 2.628 | 2.147 | 7.801 | 1.983 | 14.851 |
| 145.0 | 0.84 | 2.358 | 2.004 | 15.013 | 2.366 | 0.331 | 2.421 | 2.665 | 2.172 | 7.906 | 2.004 | 15.011 |
| 150.0 | 0.87 | 2.386 | 2.025 | 15.149 | 2.397 | 0.448 | 2.451 | 2.723 | 2.195 | 7.987 | 2.025 | 15.147 |
| 155.0 | 0.90 | 2.413 | 2.045 | 15.263 | 2.427 | 0.584 | 2.481 | 2.801 | 2.219 | 8.046 | 2.045 | 15.260 |
| 160.0 | 0.93 | 2.442 | 2.065 | 15.455 | 2.457 | 0.616 | 2.510 | 2.773 | 2.242 | 8.195 | 2.065 | 15.454 |
| 165.0 | 0.96 | 2.470 | 2.084 | 15.623 | 2.487 | 0.670 | 2.538 | 2.768 | 2.265 | 8.319 | 2.084 | 15.623 |

**Table 1c.** Key properties of the pair correlation function resulting from Langevin dynamics simulations and five integral theory approaches: the hypernetted-chain approximation (HNC), isomorph-based empirically modified hypernetted-chain approximation (IEMHNC), variational modified hypernetted-chain approximation (VMHNC), Rogers-Young approximation (RY) and Ballone-Pastore-Galli-Gazzillo approximation (BPGG). The absolute relative deviation $\epsilon_{\rm r}$ between the theoretical and the simulation results is also reported. **Results for the position of the first maximum in the case of $\boldsymbol{\kappa = 0}$**. The LD results are adopted from Table 4 of *T. Ott and M. Bonitz, Contrib. Plasma Phys.* **55**, *243 (2015).* Here $x = r/d$, where $d$ is the Wigner-Seitz radius.

| $\Gamma$ | $\Gamma/\Gamma_{\rm m}$ | $x_{\rm max1}^{\rm LD}$ | $x_{\rm max1}^{\rm HNC}$ | $\epsilon_{\rm HNC}(\%)$ | $x_{\rm max1}^{\rm IEMHNC}$ | $\epsilon_{\rm IEMHNC}(\%)$ | $x_{\rm max1}^{\rm VMHNC}$ | $\epsilon_{\rm VMHNC}(\%)$ | $x_{\rm max1}^{\rm RY}$ | $\epsilon_{\rm RY}(\%)$ | $x_{\rm max1}^{\rm BPGG}$ | $\epsilon_{\rm BPGG}(\%)$ |
|---|---|---|---|---|---|---|---|---|---|---|---|---|
| 15.0 | 0.09 | 1.666 | 1.663 | 0.180 | 1.678 | 0.720 | 1.644 | 1.321 | 1.646 | 1.200 | 1.663 | 0.180 |
| 20.0 | 0.12 | 1.665 | 1.657 | 0.480 | 1.672 | 0.420 | 1.647 | 1.081 | 1.644 | 1.261 | 1.657 | 0.480 |
| 25.0 | 0.15 | 1.668 | 1.655 | 0.779 | 1.670 | 0.120 | 1.652 | 0.959 | 1.646 | 1.319 | 1.655 | 0.779 |
| 30.0 | 0.17 | 1.671 | 1.655 | 0.958 | 1.670 | 0.060 | 1.658 | 0.778 | 1.648 | 1.376 | 1.655 | 0.958 |
| 35.0 | 0.20 | 1.674 | 1.657 | 1.016 | 1.671 | 0.179 | 1.664 | 0.597 | 1.651 | 1.374 | 1.657 | 1.016 |
| 40.0 | 0.23 | 1.678 | 1.658 | 1.192 | 1.673 | 0.298 | 1.669 | 0.536 | 1.654 | 1.430 | 1.658 | 1.192 |
| 45.0 | 0.26 | 1.681 | 1.660 | 1.249 | 1.676 | 0.297 | 1.674 | 0.416 | 1.657 | 1.428 | 1.660 | 1.249 |
| 50.0 | 0.29 | 1.685 | 1.662 | 1.365 | 1.678 | 0.415 | 1.678 | 0.415 | 1.660 | 1.484 | 1.662 | 1.365 |
| 55.0 | 0.32 | 1.688 | 1.664 | 1.422 | 1.681 | 0.415 | 1.683 | 0.296 | 1.663 | 1.481 | 1.664 | 1.422 |
| 60.0 | 0.35 | 1.690 | 1.666 | 1.420 | 1.683 | 0.414 | 1.687 | 0.178 | 1.665 | 1.479 | 1.666 | 1.420 |
| 65.0 | 0.38 | 1.693 | 1.668 | 1.477 | 1.686 | 0.413 | 1.690 | 0.177 | 1.668 | 1.477 | 1.668 | 1.477 |
| 70.0 | 0.41 | 1.696 | 1.669 | 1.592 | 1.688 | 0.472 | 1.694 | 0.118 | 1.670 | 1.533 | 1.670 | 1.533 |
| 75.0 | 0.44 | 1.698 | 1.671 | 1.590 | 1.690 | 0.471 | 1.697 | 0.059 | 1.672 | 1.531 | 1.671 | 1.590 |
| 80.0 | 0.47 | 1.701 | 1.673 | 1.646 | 1.693 | 0.470 | 1.700 | 0.059 | 1.674 | 1.587 | 1.673 | 1.646 |
| 85.0 | 0.49 | 1.703 | 1.675 | 1.644 | 1.695 | 0.470 | 1.703 | 0.000 | 1.676 | 1.585 | 1.675 | 1.644 |
| 90.0 | 0.52 | 1.705 | 1.676 | 1.701 | 1.697 | 0.469 | 1.705 | 0.000 | 1.678 | 1.584 | 1.676 | 1.701 |
| 95.0 | 0.55 | 1.707 | 1.678 | 1.699 | 1.699 | 0.469 | 1.708 | 0.059 | 1.680 | 1.582 | 1.678 | 1.699 |
| 100.0 | 0.58 | 1.709 | 1.679 | 1.755 | 1.701 | 0.468 | 1.710 | 0.059 | 1.682 | 1.580 | 1.679 | 1.755 |
| 105.0 | 0.61 | 1.710 | 1.681 | 1.696 | 1.703 | 0.409 | 1.713 | 0.175 | 1.684 | 1.520 | 1.681 | 1.696 |
| 110.0 | 0.64 | 1.712 | 1.682 | 1.752 | 1.705 | 0.409 | 1.715 | 0.175 | 1.685 | 1.577 | 1.682 | 1.752 |
| 115.0 | 0.67 | 1.714 | 1.683 | 1.809 | 1.707 | 0.408 | 1.717 | 0.175 | 1.687 | 1.575 | 1.683 | 1.809 |
| 120.0 | 0.70 | 1.715 | 1.685 | 1.749 | 1.708 | 0.408 | 1.719 | 0.233 | 1.689 | 1.516 | 1.685 | 1.749 |
| 125.0 | 0.73 | 1.717 | 1.686 | 1.805 | 1.710 | 0.408 | 1.721 | 0.233 | 1.690 | 1.573 | 1.686 | 1.805 |
| 130.0 | 0.76 | 1.719 | 1.687 | 1.862 | 1.712 | 0.407 | 1.722 | 0.175 | 1.691 | 1.629 | 1.687 | 1.862 |
| 135.0 | 0.79 | 1.720 | 1.688 | 1.860 | 1.713 | 0.407 | 1.724 | 0.233 | 1.693 | 1.570 | 1.688 | 1.860 |
| 140.0 | 0.81 | 1.721 | 1.690 | 1.801 | 1.715 | 0.349 | 1.726 | 0.291 | 1.694 | 1.569 | 1.690 | 1.801 |
| 145.0 | 0.84 | 1.723 | 1.691 | 1.857 | 1.716 | 0.406 | 1.728 | 0.290 | 1.695 | 1.625 | 1.691 | 1.857 |
| 150.0 | 0.87 | 1.724 | 1.692 | 1.856 | 1.718 | 0.348 | 1.729 | 0.290 | 1.697 | 1.566 | 1.692 | 1.856 |
| 155.0 | 0.90 | 1.725 | 1.693 | 1.855 | 1.719 | 0.348 | 1.731 | 0.348 | 1.698 | 1.565 | 1.693 | 1.855 |
| 160.0 | 0.93 | 1.727 | 1.694 | 1.911 | 1.721 | 0.347 | 1.732 | 0.290 | 1.699 | 1.621 | 1.694 | 1.911 |
| 165.0 | 0.96 | 1.728 | 1.695 | 1.910 | 1.722 | 0.347 | 1.733 | 0.289 | 1.700 | 1.620 | 1.695 | 1.910 |

**Table 1d.** Key properties of the pair correlation function resulting from Langevin dynamics simulations and five integral theory approaches: the hypernetted-chain approximation (HNC), isomorph-based empirically modified hypernetted-chain approximation (IEMHNC), variational modified hypernetted-chain approximation (VMHNC), Rogers-Young approximation (RY) and Ballone-Pastore-Galli-Gazzillo approximation (BPGG). The absolute relative deviation $\epsilon_{\mathrm{r}}$ between the theoretical and the simulation results is also reported. **Results for the magnitude of the first minimum in the case of $\boldsymbol{\kappa = 0}$**. The LD results are adopted from Table 4 of *T. Ott and M. Bonitz, Contrib. Plasma Phys.* **55**, *243 (2015).*

| $\Gamma$ | $\Gamma/\Gamma_{\mathrm{m}}$ | $g_{\mathrm{min1}}^{\mathrm{LD}}$ | $g_{\mathrm{min1}}^{\mathrm{HNC}}$ | $\epsilon_{\mathrm{HNC}}(\%)$ | $g_{\mathrm{min1}}^{\mathrm{IEMHNC}}$ | $\epsilon_{\mathrm{IEMHNC}}(\%)$ | $g_{\mathrm{min1}}^{\mathrm{VMHNC}}$ | $\epsilon_{\mathrm{VMHNC}}(\%)$ | $g_{\mathrm{min1}}^{\mathrm{RY}}$ | $\epsilon_{\mathrm{RY}}(\%)$ | $g_{\mathrm{min1}}^{\mathrm{BPGG}}$ | $\epsilon_{\mathrm{BPGG}}(\%)$ |
|---|---|---|---|---|---|---|---|---|---|---|---|---|
| 15.0 | 0.09 | 0.952 | 0.971 | 1.956 | 0.959 | 0.743 | 0.959 | 0.689 | 0.961 | 0.975 | 0.971 | 1.955 |
| 20.0 | 0.12 | 0.925 | 0.953 | 3.038 | 0.935 | 1.092 | 0.932 | 0.782 | 0.940 | 1.588 | 0.953 | 3.037 |
| 25.0 | 0.15 | 0.899 | 0.936 | 4.107 | 0.912 | 1.397 | 0.907 | 0.858 | 0.919 | 2.240 | 0.936 | 4.106 |
| 30.0 | 0.17 | 0.876 | 0.920 | 4.976 | 0.889 | 1.521 | 0.883 | 0.787 | 0.900 | 2.747 | 0.920 | 4.975 |
| 35.0 | 0.20 | 0.853 | 0.904 | 6.008 | 0.869 | 1.837 | 0.861 | 0.924 | 0.882 | 3.457 | 0.904 | 6.007 |
| 40.0 | 0.23 | 0.833 | 0.890 | 6.831 | 0.850 | 1.987 | 0.841 | 0.906 | 0.866 | 3.998 | 0.890 | 6.830 |
| 45.0 | 0.26 | 0.814 | 0.877 | 7.678 | 0.832 | 2.192 | 0.822 | 0.949 | 0.851 | 4.590 | 0.876 | 7.678 |
| 50.0 | 0.29 | 0.796 | 0.864 | 8.538 | 0.815 | 2.434 | 0.804 | 1.032 | 0.838 | 5.218 | 0.864 | 8.538 |
| 55.0 | 0.32 | 0.780 | 0.852 | 9.258 | 0.800 | 2.565 | 0.788 | 1.006 | 0.825 | 5.728 | 0.852 | 9.258 |
| 60.0 | 0.35 | 0.765 | 0.841 | 9.957 | 0.786 | 2.691 | 0.772 | 0.977 | 0.813 | 6.232 | 0.841 | 9.958 |
| 65.0 | 0.38 | 0.750 | 0.831 | 10.770 | 0.772 | 2.935 | 0.758 | 1.063 | 0.801 | 6.857 | 0.831 | 10.770 |
| 70.0 | 0.41 | 0.737 | 0.821 | 11.391 | 0.759 | 3.008 | 0.744 | 0.982 | 0.791 | 7.307 | 0.821 | 11.391 |
| 75.0 | 0.44 | 0.724 | 0.812 | 12.106 | 0.747 | 3.173 | 0.731 | 0.991 | 0.781 | 7.855 | 0.812 | 12.106 |
| 80.0 | 0.47 | 0.711 | 0.803 | 12.913 | 0.735 | 3.426 | 0.719 | 1.086 | 0.771 | 8.498 | 0.803 | 12.914 |
| 85.0 | 0.49 | 0.700 | 0.794 | 13.487 | 0.724 | 3.466 | 0.707 | 0.972 | 0.762 | 8.921 | 0.794 | 13.488 |
| 90.0 | 0.52 | 0.689 | 0.786 | 14.135 | 0.714 | 3.576 | 0.695 | 0.925 | 0.754 | 9.420 | 0.786 | 14.136 |
| 95.0 | 0.55 | 0.678 | 0.779 | 14.857 | 0.703 | 3.751 | 0.684 | 0.942 | 0.746 | 9.993 | 0.779 | 14.858 |
| 100.0 | 0.58 | 0.668 | 0.771 | 15.478 | 0.694 | 3.835 | 0.674 | 0.868 | 0.738 | 10.473 | 0.771 | 15.479 |
| 105.0 | 0.61 | 0.658 | 0.764 | 16.163 | 0.684 | 3.975 | 0.664 | 0.847 | 0.730 | 11.016 | 0.764 | 16.165 |
| 110.0 | 0.64 | 0.648 | 0.758 | 16.912 | 0.675 | 4.169 | 0.654 | 0.877 | 0.723 | 11.622 | 0.758 | 16.914 |
| 115.0 | 0.67 | 0.639 | 0.751 | 17.539 | 0.666 | 4.253 | 0.644 | 0.799 | 0.716 | 12.115 | 0.751 | 17.541 |
| 120.0 | 0.70 | 0.630 | 0.745 | 18.222 | 0.658 | 4.384 | 0.635 | 0.763 | 0.710 | 12.662 | 0.745 | 18.224 |
| 125.0 | 0.73 | 0.621 | 0.739 | 18.960 | 0.649 | 4.561 | 0.626 | 0.770 | 0.703 | 13.263 | 0.739 | 18.962 |
| 130.0 | 0.76 | 0.613 | 0.733 | 19.557 | 0.641 | 4.612 | 0.617 | 0.652 | 0.697 | 13.731 | 0.733 | 19.560 |
| 135.0 | 0.79 | 0.605 | 0.727 | 20.202 | 0.633 | 4.701 | 0.608 | 0.570 | 0.691 | 14.245 | 0.727 | 20.205 |
| 140.0 | 0.81 | 0.596 | 0.722 | 21.096 | 0.626 | 5.005 | 0.600 | 0.688 | 0.685 | 14.998 | 0.722 | 21.099 |
| 145.0 | 0.84 | 0.588 | 0.716 | 21.838 | 0.618 | 5.173 | 0.592 | 0.674 | 0.680 | 15.607 | 0.716 | 21.841 |
| 150.0 | 0.87 | 0.581 | 0.711 | 22.418 | 0.611 | 5.197 | 0.584 | 0.519 | 0.674 | 16.062 | 0.711 | 22.421 |
| 155.0 | 0.90 | 0.574 | 0.706 | 23.037 | 0.604 | 5.253 | 0.576 | 0.390 | 0.669 | 16.555 | 0.706 | 23.040 |
| 160.0 | 0.93 | 0.567 | 0.701 | 23.694 | 0.597 | 5.340 | 0.569 | 0.288 | 0.664 | 17.087 | 0.701 | 23.698 |
| 165.0 | 0.96 | 0.560 | 0.697 | 24.392 | 0.591 | 5.459 | 0.561 | 0.212 | 0.659 | 17.657 | 0.697 | 24.397 |

**Table 1e.** Key properties of the pair correlation function resulting from Langevin dynamics simulations and five integral theory approaches: the hypernetted-chain approximation (HNC), isomorph-based empirically modified hypernetted-chain approximation (IEMHNC), variational modified hypernetted-chain approximation (VMHNC), Rogers-Young approximation (RY) and Ballone-Pastore-Galli-Gazzillo approximation (BPGG). The absolute relative deviation $\epsilon_{\mathrm{r}}$ between the theoretical and the simulation results is also reported. **Results for the position of the first minimum in the case of $\boldsymbol{\kappa = 0}$**. The LD results are adopted from Table 4 of *T. Ott and M. Bonitz, Contrib. Plasma Phys.* **55***, 243 (2015).* Here $x = r/d$, where $d$ is the Wigner-Seitz radius.

| $\Gamma$ | $\Gamma/\Gamma_{\mathrm{m}}$ | $x_{\mathrm{min1}}^{\mathrm{LD}}$ | $x_{\mathrm{min1}}^{\mathrm{HNC}}$ | $\epsilon_{\mathrm{HNC}}(\%)$ | $x_{\mathrm{min1}}^{\mathrm{IEMHNC}}$ | $\epsilon_{\mathrm{IEMHNC}}(\%)$ | $x_{\mathrm{min1}}^{\mathrm{VMHNC}}$ | $\epsilon_{\mathrm{VMHNC}}(\%)$ | $x_{\mathrm{min1}}^{\mathrm{RY}}$ | $\epsilon_{\mathrm{RY}}(\%)$ | $x_{\mathrm{min1}}^{\mathrm{BPGG}}$ | $\epsilon_{\mathrm{BPGG}}(\%)$ |
|---|---|---|---|---|---|---|---|---|---|---|---|---|
| 15.0 | 0.09 | 2.489 | 2.540 | 2.049 | 2.538 | 1.969 | 2.467 | 0.884 | 2.502 | 0.522 | 2.540 | 2.049 |
| 20.0 | 0.12 | 2.472 | 2.514 | 1.699 | 2.510 | 1.537 | 2.445 | 1.092 | 2.487 | 0.607 | 2.514 | 1.699 |
| 25.0 | 0.15 | 2.467 | 2.502 | 1.419 | 2.494 | 1.094 | 2.439 | 1.135 | 2.481 | 0.567 | 2.502 | 1.419 |
| 30.0 | 0.17 | 2.463 | 2.496 | 1.340 | 2.485 | 0.893 | 2.437 | 1.056 | 2.478 | 0.609 | 2.496 | 1.340 |
| 35.0 | 0.20 | 2.461 | 2.492 | 1.260 | 2.480 | 0.772 | 2.435 | 1.056 | 2.478 | 0.691 | 2.492 | 1.260 |
| 40.0 | 0.23 | 2.461 | 2.490 | 1.178 | 2.476 | 0.610 | 2.433 | 1.138 | 2.477 | 0.650 | 2.490 | 1.178 |
| 45.0 | 0.26 | 2.459 | 2.489 | 1.220 | 2.473 | 0.569 | 2.431 | 1.139 | 2.477 | 0.732 | 2.489 | 1.220 |
| 50.0 | 0.29 | 2.459 | 2.488 | 1.179 | 2.471 | 0.488 | 2.429 | 1.220 | 2.477 | 0.732 | 2.488 | 1.179 |
| 55.0 | 0.32 | 2.456 | 2.487 | 1.262 | 2.468 | 0.489 | 2.426 | 1.221 | 2.476 | 0.814 | 2.487 | 1.262 |
| 60.0 | 0.35 | 2.455 | 2.486 | 1.263 | 2.466 | 0.448 | 2.424 | 1.263 | 2.476 | 0.855 | 2.487 | 1.303 |
| 65.0 | 0.38 | 2.454 | 2.486 | 1.304 | 2.464 | 0.407 | 2.421 | 1.345 | 2.475 | 0.856 | 2.486 | 1.304 |
| 70.0 | 0.41 | 2.453 | 2.485 | 1.305 | 2.462 | 0.367 | 2.418 | 1.427 | 2.474 | 0.856 | 2.485 | 1.305 |
| 75.0 | 0.44 | 2.451 | 2.484 | 1.346 | 2.459 | 0.326 | 2.414 | 1.510 | 2.473 | 0.898 | 2.484 | 1.346 |
| 80.0 | 0.47 | 2.449 | 2.484 | 1.429 | 2.457 | 0.327 | 2.411 | 1.552 | 2.472 | 0.939 | 2.484 | 1.429 |
| 85.0 | 0.49 | 2.448 | 2.483 | 1.430 | 2.455 | 0.286 | 2.408 | 1.634 | 2.471 | 0.940 | 2.483 | 1.430 |
| 90.0 | 0.52 | 2.446 | 2.482 | 1.472 | 2.453 | 0.286 | 2.405 | 1.676 | 2.470 | 0.981 | 2.482 | 1.472 |
| 95.0 | 0.55 | 2.443 | 2.481 | 1.555 | 2.450 | 0.287 | 2.402 | 1.678 | 2.468 | 1.023 | 2.481 | 1.555 |
| 100.0 | 0.58 | 2.441 | 2.480 | 1.598 | 2.448 | 0.287 | 2.399 | 1.721 | 2.467 | 1.065 | 2.480 | 1.598 |
| 105.0 | 0.61 | 2.439 | 2.479 | 1.640 | 2.446 | 0.287 | 2.396 | 1.763 | 2.465 | 1.066 | 2.479 | 1.640 |
| 110.0 | 0.64 | 2.439 | 2.478 | 1.599 | 2.444 | 0.205 | 2.393 | 1.886 | 2.464 | 1.025 | 2.478 | 1.599 |
| 115.0 | 0.67 | 2.437 | 2.476 | 1.600 | 2.442 | 0.205 | 2.390 | 1.929 | 2.462 | 1.026 | 2.476 | 1.600 |
| 120.0 | 0.70 | 2.435 | 2.475 | 1.643 | 2.440 | 0.205 | 2.387 | 1.971 | 2.461 | 1.068 | 2.475 | 1.643 |
| 125.0 | 0.73 | 2.434 | 2.474 | 1.643 | 2.438 | 0.164 | 2.384 | 2.054 | 2.460 | 1.068 | 2.474 | 1.643 |
| 130.0 | 0.76 | 2.432 | 2.473 | 1.686 | 2.436 | 0.164 | 2.381 | 2.097 | 2.458 | 1.069 | 2.473 | 1.686 |
| 135.0 | 0.79 | 2.431 | 2.472 | 1.687 | 2.434 | 0.123 | 2.379 | 2.139 | 2.457 | 1.070 | 2.472 | 1.687 |
| 140.0 | 0.81 | 2.428 | 2.471 | 1.771 | 2.432 | 0.165 | 2.376 | 2.142 | 2.455 | 1.112 | 2.471 | 1.771 |
| 145.0 | 0.84 | 2.428 | 2.469 | 1.689 | 2.430 | 0.082 | 2.373 | 2.265 | 2.454 | 1.071 | 2.469 | 1.689 |
| 150.0 | 0.87 | 2.426 | 2.468 | 1.731 | 2.429 | 0.124 | 2.371 | 2.267 | 2.452 | 1.072 | 2.468 | 1.731 |
| 155.0 | 0.90 | 2.425 | 2.467 | 1.732 | 2.427 | 0.082 | 2.368 | 2.351 | 2.451 | 1.072 | 2.467 | 1.732 |
| 160.0 | 0.93 | 2.424 | 2.466 | 1.733 | 2.425 | 0.041 | 2.366 | 2.393 | 2.449 | 1.031 | 2.466 | 1.733 |
| 165.0 | 0.96 | 2.423 | 2.465 | 1.733 | 2.424 | 0.041 | 2.364 | 2.435 | 2.448 | 1.032 | 2.465 | 1.733 |

**Table 1f.** Key properties of the pair correlation function resulting from Langevin dynamics simulations and five integral theory approaches: the hypernetted-chain approximation (HNC), isomorph-based empirically modified hypernetted-chain approximation (IEMHNC), variational modified hypernetted-chain approximation (VMHNC), Rogers-Young approximation (RY) and Ballone-Pastore-Galli-Gazzillo approximation (BPGG). The absolute relative deviation $\epsilon_{\mathrm{r}}$ between the theoretical and the simulation results is reported. **Results for the magnitude of the second maximum in the case of $\boldsymbol{\kappa = 0}$**. The LD results are adopted from Table 4 of *T. Ott and M. Bonitz, Contrib. Plasma Phys.* **55**, *243 (2015).*

| $\Gamma$ | $\Gamma/\Gamma_{\mathrm{m}}$ | $g_{\mathrm{max2}}^{\mathrm{LD}}$ | $g_{\mathrm{max2}}^{\mathrm{HNC}}$ | $\epsilon_{\mathrm{HNC}}(\%)$ | $g_{\mathrm{max2}}^{\mathrm{IEMHNC}}$ | $\epsilon_{\mathrm{IEMHNC}}(\%)$ | $g_{\mathrm{max2}}^{\mathrm{VMHNC}}$ | $\epsilon_{\mathrm{VMHNC}}(\%)$ | $g_{\mathrm{max2}}^{\mathrm{RY}}$ | $\epsilon_{\mathrm{RY}}(\%)$ | $g_{\mathrm{max2}}^{\mathrm{BPGG}}$ | $\epsilon_{\mathrm{BPGG}}(\%)$ |
|---|---|---|---|---|---|---|---|---|---|---|---|---|
| 15.0 | 0.09 | 1.012 | 1.006 | 0.594 | 1.010 | 0.189 | 1.010 | 0.196 | 1.009 | 0.314 | 1.006 | 0.594 |
| 20.0 | 0.12 | 1.023 | 1.012 | 1.106 | 1.019 | 0.369 | 1.020 | 0.276 | 1.017 | 0.613 | 1.012 | 1.106 |
| 25.0 | 0.15 | 1.035 | 1.018 | 1.609 | 1.030 | 0.493 | 1.032 | 0.284 | 1.026 | 0.899 | 1.018 | 1.609 |
| 30.0 | 0.17 | 1.047 | 1.026 | 2.047 | 1.042 | 0.523 | 1.045 | 0.206 | 1.035 | 1.124 | 1.026 | 2.047 |
| 35.0 | 0.20 | 1.060 | 1.033 | 2.536 | 1.054 | 0.597 | 1.058 | 0.186 | 1.045 | 1.411 | 1.033 | 2.536 |
| 40.0 | 0.23 | 1.073 | 1.041 | 2.997 | 1.066 | 0.645 | 1.071 | 0.156 | 1.055 | 1.682 | 1.041 | 2.997 |
| 45.0 | 0.26 | 1.085 | 1.049 | 3.351 | 1.079 | 0.590 | 1.085 | 0.043 | 1.065 | 1.856 | 1.049 | 3.351 |
| 50.0 | 0.29 | 1.098 | 1.056 | 3.783 | 1.091 | 0.627 | 1.098 | 0.042 | 1.075 | 2.121 | 1.056 | 3.783 |
| 55.0 | 0.32 | 1.110 | 1.064 | 4.121 | 1.104 | 0.580 | 1.110 | 0.024 | 1.084 | 2.301 | 1.064 | 4.121 |
| 60.0 | 0.35 | 1.122 | 1.072 | 4.456 | 1.116 | 0.542 | 1.123 | 0.060 | 1.094 | 2.489 | 1.072 | 4.457 |
| 65.0 | 0.38 | 1.133 | 1.080 | 4.707 | 1.128 | 0.429 | 1.135 | 0.153 | 1.104 | 2.600 | 1.080 | 4.708 |
| 70.0 | 0.41 | 1.145 | 1.087 | 5.043 | 1.140 | 0.419 | 1.146 | 0.126 | 1.113 | 2.808 | 1.087 | 5.045 |
| 75.0 | 0.44 | 1.156 | 1.095 | 5.299 | 1.152 | 0.338 | 1.158 | 0.154 | 1.122 | 2.941 | 1.095 | 5.301 |
| 80.0 | 0.47 | 1.166 | 1.102 | 5.478 | 1.164 | 0.188 | 1.169 | 0.236 | 1.131 | 3.004 | 1.102 | 5.480 |
| 85.0 | 0.49 | 1.176 | 1.109 | 5.662 | 1.175 | 0.056 | 1.179 | 0.286 | 1.140 | 3.079 | 1.109 | 5.664 |
| 90.0 | 0.52 | 1.186 | 1.117 | 5.853 | 1.187 | 0.057 | 1.190 | 0.305 | 1.148 | 3.167 | 1.117 | 5.855 |
| 95.0 | 0.55 | 1.196 | 1.124 | 6.048 | 1.198 | 0.152 | 1.200 | 0.296 | 1.157 | 3.268 | 1.124 | 6.051 |
| 100.0 | 0.58 | 1.205 | 1.131 | 6.172 | 1.209 | 0.311 | 1.209 | 0.342 | 1.165 | 3.300 | 1.131 | 6.175 |
| 105.0 | 0.61 | 1.213 | 1.137 | 6.226 | 1.219 | 0.535 | 1.218 | 0.443 | 1.173 | 3.266 | 1.137 | 6.229 |
| 110.0 | 0.64 | 1.222 | 1.144 | 6.364 | 1.230 | 0.658 | 1.227 | 0.435 | 1.181 | 3.323 | 1.144 | 6.367 |
| 115.0 | 0.67 | 1.231 | 1.151 | 6.509 | 1.240 | 0.761 | 1.236 | 0.403 | 1.189 | 3.393 | 1.151 | 6.512 |
| 120.0 | 0.70 | 1.238 | 1.157 | 6.509 | 1.251 | 1.011 | 1.244 | 0.509 | 1.197 | 3.318 | 1.157 | 6.512 |
| 125.0 | 0.73 | 1.246 | 1.164 | 6.592 | 1.260 | 1.159 | 1.252 | 0.512 | 1.204 | 3.333 | 1.164 | 6.596 |
| 130.0 | 0.76 | 1.253 | 1.170 | 6.608 | 1.270 | 1.371 | 1.260 | 0.572 | 1.212 | 3.282 | 1.170 | 6.612 |
| 135.0 | 0.79 | 1.260 | 1.176 | 6.632 | 1.280 | 1.565 | 1.268 | 0.611 | 1.219 | 3.243 | 1.176 | 6.636 |
| 140.0 | 0.81 | 1.267 | 1.183 | 6.662 | 1.289 | 1.741 | 1.275 | 0.630 | 1.226 | 3.216 | 1.183 | 6.667 |
| 145.0 | 0.84 | 1.273 | 1.189 | 6.627 | 1.298 | 1.980 | 1.282 | 0.708 | 1.233 | 3.123 | 1.189 | 6.631 |
| 150.0 | 0.87 | 1.279 | 1.195 | 6.599 | 1.307 | 2.202 | 1.289 | 0.768 | 1.240 | 3.041 | 1.195 | 6.604 |
| 155.0 | 0.90 | 1.285 | 1.200 | 6.579 | 1.316 | 2.407 | 1.295 | 0.809 | 1.247 | 2.970 | 1.200 | 6.584 |
| 160.0 | 0.93 | 1.291 | 1.206 | 6.566 | 1.324 | 2.594 | 1.302 | 0.833 | 1.253 | 2.909 | 1.206 | 6.571 |
| 165.0 | 0.96 | 1.297 | 1.212 | 6.559 | 1.333 | 2.766 | 1.308 | 0.840 | 1.260 | 2.858 | 1.212 | 6.565 |

**Table 1g.** Key properties of the pair correlation function resulting from Langevin dynamics simulations and five integral theory approaches: the hypernetted-chain approximation (HNC), isomorph-based empirically modified hypernetted-chain approximation (IEMHNC), variational modified hypernetted-chain approximation (VMHNC), Rogers-Young approximation (RY) and Ballone-Pastore-Galli-Gazzillo approximation (BPGG). The absolute relative deviation $\epsilon_{\mathrm{r}}$ between the theoretical and the simulation results is also reported. **Results for the position of the second maximum in the case of $\boldsymbol{\kappa = 0}$**. The LD results are adopted from Table 4 of *T. Ott and M. Bonitz, Contrib. Plasma Phys.* **55**, *243 (2015)*. Here $x = r/d$, where $d$ is the Wigner-Seitz radius.

| $\Gamma$ | $\Gamma/\Gamma_{\mathrm{m}}$ | $x_{\mathrm{max2}}^{\mathrm{LD}}$ | $x_{\mathrm{max2}}^{\mathrm{HNC}}$ | $\epsilon_{\mathrm{HNC}}(\%)$ | $x_{\mathrm{max2}}^{\mathrm{IEMHNC}}$ | $\epsilon_{\mathrm{IEMHNC}}(\%)$ | $x_{\mathrm{max2}}^{\mathrm{VMHNC}}$ | $\epsilon_{\mathrm{VMHNC}}(\%)$ | $x_{\mathrm{max2}}^{\mathrm{RY}}$ | $\epsilon_{\mathrm{RY}}(\%)$ | $x_{\mathrm{max2}}^{\mathrm{BPGG}}$ | $\epsilon_{\mathrm{BPGG}}(\%)$ |
|---|---|---|---|---|---|---|---|---|---|---|---|---|
| 15.0 | 0.09 | 3.298 | 3.402 | 3.153 | 3.384 | 2.608 | 3.292 | 0.182 | 3.339 | 1.243 | 3.402 | 3.153 |
| 20.0 | 0.12 | 3.278 | 3.350 | 2.196 | 3.332 | 1.647 | 3.258 | 0.610 | 3.302 | 0.732 | 3.351 | 2.227 |
| 25.0 | 0.15 | 3.259 | 3.322 | 1.933 | 3.300 | 1.258 | 3.244 | 0.460 | 3.282 | 0.706 | 3.322 | 1.933 |
| 30.0 | 0.17 | 3.248 | 3.304 | 1.724 | 3.280 | 0.985 | 3.239 | 0.277 | 3.270 | 0.677 | 3.304 | 1.724 |
| 35.0 | 0.20 | 3.244 | 3.292 | 1.480 | 3.267 | 0.709 | 3.237 | 0.216 | 3.262 | 0.555 | 3.292 | 1.480 |
| 40.0 | 0.23 | 3.240 | 3.283 | 1.327 | 3.259 | 0.586 | 3.237 | 0.093 | 3.257 | 0.525 | 3.284 | 1.358 |
| 45.0 | 0.26 | 3.238 | 3.277 | 1.204 | 3.253 | 0.463 | 3.238 | 0.000 | 3.253 | 0.463 | 3.277 | 1.204 |
| 50.0 | 0.29 | 3.236 | 3.272 | 1.112 | 3.249 | 0.402 | 3.239 | 0.093 | 3.251 | 0.464 | 3.272 | 1.112 |
| 55.0 | 0.32 | 3.235 | 3.268 | 1.020 | 3.247 | 0.371 | 3.242 | 0.216 | 3.249 | 0.433 | 3.268 | 1.020 |
| 60.0 | 0.35 | 3.233 | 3.265 | 0.990 | 3.245 | 0.371 | 3.244 | 0.340 | 3.247 | 0.433 | 3.265 | 0.990 |
| 65.0 | 0.38 | 3.234 | 3.263 | 0.897 | 3.244 | 0.309 | 3.247 | 0.402 | 3.246 | 0.371 | 3.263 | 0.897 |
| 70.0 | 0.41 | 3.231 | 3.261 | 0.929 | 3.243 | 0.371 | 3.249 | 0.557 | 3.246 | 0.464 | 3.261 | 0.929 |
| 75.0 | 0.44 | 3.232 | 3.259 | 0.835 | 3.243 | 0.340 | 3.252 | 0.619 | 3.245 | 0.402 | 3.259 | 0.835 |
| 80.0 | 0.47 | 3.232 | 3.258 | 0.804 | 3.243 | 0.340 | 3.255 | 0.712 | 3.245 | 0.402 | 3.258 | 0.804 |
| 85.0 | 0.49 | 3.233 | 3.257 | 0.742 | 3.243 | 0.309 | 3.257 | 0.742 | 3.245 | 0.371 | 3.257 | 0.742 |
| 90.0 | 0.52 | 3.234 | 3.256 | 0.680 | 3.244 | 0.309 | 3.260 | 0.804 | 3.245 | 0.340 | 3.256 | 0.680 |
| 95.0 | 0.55 | 3.232 | 3.255 | 0.712 | 3.244 | 0.371 | 3.262 | 0.928 | 3.245 | 0.402 | 3.255 | 0.712 |
| 100.0 | 0.58 | 3.232 | 3.255 | 0.712 | 3.245 | 0.402 | 3.265 | 1.021 | 3.246 | 0.433 | 3.255 | 0.712 |
| 105.0 | 0.61 | 3.233 | 3.254 | 0.650 | 3.246 | 0.402 | 3.267 | 1.052 | 3.246 | 0.402 | 3.254 | 0.650 |
| 110.0 | 0.64 | 3.233 | 3.254 | 0.650 | 3.246 | 0.402 | 3.270 | 1.144 | 3.246 | 0.402 | 3.254 | 0.650 |
| 115.0 | 0.67 | 3.233 | 3.254 | 0.650 | 3.247 | 0.433 | 3.272 | 1.206 | 3.247 | 0.433 | 3.254 | 0.650 |
| 120.0 | 0.70 | 3.234 | 3.254 | 0.618 | 3.248 | 0.433 | 3.275 | 1.268 | 3.247 | 0.402 | 3.254 | 0.618 |
| 125.0 | 0.73 | 3.233 | 3.254 | 0.650 | 3.249 | 0.495 | 3.277 | 1.361 | 3.248 | 0.464 | 3.254 | 0.650 |
| 130.0 | 0.76 | 3.233 | 3.254 | 0.650 | 3.250 | 0.526 | 3.279 | 1.423 | 3.248 | 0.464 | 3.254 | 0.650 |
| 135.0 | 0.79 | 3.235 | 3.254 | 0.587 | 3.251 | 0.495 | 3.281 | 1.422 | 3.249 | 0.433 | 3.254 | 0.587 |
| 140.0 | 0.81 | 3.234 | 3.254 | 0.618 | 3.252 | 0.557 | 3.283 | 1.515 | 3.250 | 0.495 | 3.254 | 0.618 |
| 145.0 | 0.84 | 3.235 | 3.254 | 0.587 | 3.253 | 0.556 | 3.285 | 1.546 | 3.250 | 0.464 | 3.254 | 0.587 |
| 150.0 | 0.87 | 3.235 | 3.254 | 0.587 | 3.254 | 0.587 | 3.287 | 1.607 | 3.251 | 0.495 | 3.254 | 0.587 |
| 155.0 | 0.90 | 3.235 | 3.255 | 0.618 | 3.255 | 0.618 | 3.289 | 1.669 | 3.251 | 0.495 | 3.254 | 0.587 |
| 160.0 | 0.93 | 3.235 | 3.255 | 0.618 | 3.256 | 0.649 | 3.291 | 1.731 | 3.252 | 0.526 | 3.255 | 0.618 |
| 165.0 | 0.96 | 3.234 | 3.255 | 0.649 | 3.257 | 0.711 | 3.293 | 1.824 | 3.253 | 0.588 | 3.255 | 0.649 |

**Table 2a.** Key properties of the pair correlation function resulting from Langevin dynamics simulations and five integral theory approaches: the hypernetted-chain approximation (HNC), isomorph-based empirically modified hypernetted-chain approximation (IEMHNC), variational modified hypernetted-chain approximation (VMHNC), Rogers-Young approximation (RY) and Ballone-Pastore-Galli-Gazzillo approximation (BPGG). The absolute relative deviation $\epsilon_{\mathrm{r}}$ between the theoretical and the simulation results is also reported. **Results for $\arg_r\{g(r) = 0.5\}$ in the case of $\kappa = 1$**. The LD results are adopted from Table 5 of *T. Ott and M. Bonitz, Contrib. Plasma Phys.* **55**, *243 (2015)*. Here $x = r/d$, where $d$ is the Wigner-Seitz radius.

| $\Gamma$ | $\Gamma/\Gamma_{\mathrm{m}}$ | $x_{\mathrm{cv}}^{\mathrm{LD}}$ | $x_{\mathrm{cv}}^{\mathrm{HNC}}$ | $\epsilon_{\mathrm{HNC}}(\%)$ | $x_{\mathrm{cv}}^{\mathrm{IEMHNC}}$ | $\epsilon_{\mathrm{IEMHNC}}(\%)$ | $x_{\mathrm{cv}}^{\mathrm{VMHNC}}$ | $\epsilon_{\mathrm{VMHNC}}(\%)$ | $x_{\mathrm{cv}}^{\mathrm{RY}}$ | $\epsilon_{\mathrm{RY}}(\%)$ | $x_{\mathrm{cv}}^{\mathrm{BPGG}}$ | $\epsilon_{\mathrm{BPGG}}(\%)$ |
|---|---|---|---|---|---|---|---|---|---|---|---|---|
| 10.0 | 0.05 | 1.076 | 1.054 | 2.045 | 1.057 | 1.766 | 1.070 | 0.558 | 1.070 | 0.558 | 1.060 | 1.487 |
| 15.0 | 0.07 | 1.139 | 1.113 | 2.283 | 1.124 | 1.317 | 1.134 | 0.439 | 1.131 | 0.702 | 1.119 | 1.756 |
| 20.0 | 0.09 | 1.177 | 1.152 | 2.124 | 1.168 | 0.765 | 1.177 | 0.000 | 1.172 | 0.425 | 1.158 | 1.614 |
| 25.0 | 0.11 | 1.211 | 1.181 | 2.477 | 1.200 | 0.908 | 1.209 | 0.165 | 1.202 | 0.743 | 1.187 | 1.982 |
| 30.0 | 0.14 | 1.237 | 1.204 | 2.668 | 1.226 | 0.889 | 1.234 | 0.243 | 1.225 | 0.970 | 1.210 | 2.183 |
| 35.0 | 0.16 | 1.254 | 1.223 | 2.472 | 1.247 | 0.558 | 1.255 | 0.080 | 1.244 | 0.797 | 1.229 | 1.994 |
| 40.0 | 0.18 | 1.275 | 1.239 | 2.824 | 1.265 | 0.784 | 1.273 | 0.157 | 1.261 | 1.098 | 1.245 | 2.353 |
| 45.0 | 0.21 | 1.288 | 1.253 | 2.717 | 1.281 | 0.543 | 1.288 | 0.000 | 1.275 | 1.009 | 1.259 | 2.252 |
| 50.0 | 0.23 | 1.301 | 1.265 | 2.767 | 1.295 | 0.461 | 1.302 | 0.077 | 1.287 | 1.076 | 1.271 | 2.306 |
| 55.0 | 0.25 | 1.313 | 1.276 | 2.818 | 1.307 | 0.457 | 1.314 | 0.076 | 1.299 | 1.066 | 1.282 | 2.361 |
| 60.0 | 0.28 | 1.326 | 1.286 | 3.017 | 1.318 | 0.603 | 1.325 | 0.075 | 1.309 | 1.282 | 1.292 | 2.564 |
| 65.0 | 0.30 | 1.334 | 1.295 | 2.924 | 1.328 | 0.450 | 1.335 | 0.075 | 1.318 | 1.199 | 1.301 | 2.474 |
| 70.0 | 0.32 | 1.343 | 1.303 | 2.978 | 1.337 | 0.447 | 1.344 | 0.074 | 1.326 | 1.266 | 1.309 | 2.532 |
| 75.0 | 0.34 | 1.351 | 1.311 | 2.961 | 1.346 | 0.370 | 1.352 | 0.074 | 1.334 | 1.258 | 1.316 | 2.591 |
| 80.0 | 0.37 | 1.360 | 1.318 | 3.088 | 1.354 | 0.441 | 1.360 | 0.000 | 1.341 | 1.397 | 1.323 | 2.721 |
| 85.0 | 0.39 | 1.364 | 1.324 | 2.933 | 1.361 | 0.220 | 1.367 | 0.220 | 1.348 | 1.173 | 1.330 | 2.493 |
| 90.0 | 0.41 | 1.373 | 1.330 | 3.132 | 1.368 | 0.364 | 1.373 | 0.000 | 1.354 | 1.384 | 1.336 | 2.695 |
| 95.0 | 0.44 | 1.377 | 1.336 | 2.977 | 1.374 | 0.218 | 1.380 | 0.218 | 1.360 | 1.235 | 1.342 | 2.542 |
| 100.0 | 0.46 | 1.385 | 1.342 | 3.105 | 1.381 | 0.289 | 1.386 | 0.072 | 1.365 | 1.444 | 1.347 | 2.744 |
| 105.0 | 0.48 | 1.390 | 1.347 | 3.094 | 1.386 | 0.288 | 1.391 | 0.072 | 1.371 | 1.367 | 1.352 | 2.734 |
| 110.0 | 0.51 | 1.394 | 1.352 | 3.013 | 1.392 | 0.143 | 1.397 | 0.215 | 1.376 | 1.291 | 1.357 | 2.654 |
| 115.0 | 0.53 | 1.402 | 1.356 | 3.281 | 1.397 | 0.357 | 1.402 | 0.000 | 1.380 | 1.569 | 1.362 | 2.853 |
| 120.0 | 0.55 | 1.407 | 1.361 | 3.269 | 1.402 | 0.355 | 1.406 | 0.071 | 1.385 | 1.564 | 1.366 | 2.914 |
| 125.0 | 0.57 | 1.411 | 1.365 | 3.260 | 1.407 | 0.283 | 1.411 | 0.000 | 1.389 | 1.559 | 1.370 | 2.906 |
| 130.0 | 0.60 | 1.415 | 1.369 | 3.251 | 1.411 | 0.283 | 1.415 | 0.000 | 1.393 | 1.555 | 1.374 | 2.898 |
| 135.0 | 0.62 | 1.419 | 1.373 | 3.242 | 1.416 | 0.211 | 1.419 | 0.000 | 1.397 | 1.550 | 1.378 | 2.889 |
| 140.0 | 0.64 | 1.424 | 1.377 | 3.301 | 1.420 | 0.281 | 1.423 | 0.070 | 1.401 | 1.615 | 1.382 | 2.949 |
| 145.0 | 0.67 | 1.428 | 1.381 | 3.291 | 1.424 | 0.280 | 1.427 | 0.070 | 1.404 | 1.681 | 1.385 | 3.011 |
| 150.0 | 0.69 | 1.428 | 1.384 | 3.081 | 1.428 | 0.000 | 1.431 | 0.210 | 1.408 | 1.401 | 1.389 | 2.731 |
| 155.0 | 0.71 | 1.432 | 1.387 | 3.142 | 1.431 | 0.070 | 1.434 | 0.140 | 1.411 | 1.466 | 1.392 | 2.793 |
| 160.0 | 0.74 | 1.436 | 1.391 | 3.134 | 1.435 | 0.070 | 1.438 | 0.139 | 1.415 | 1.462 | 1.395 | 2.855 |
| 165.0 | 0.76 | 1.441 | 1.394 | 3.262 | 1.438 | 0.208 | 1.441 | 0.000 | 1.418 | 1.596 | 1.398 | 2.984 |
| 170.0 | 0.78 | 1.445 | 1.397 | 3.322 | 1.442 | 0.208 | 1.444 | 0.069 | 1.421 | 1.661 | 1.401 | 3.045 |
| 175.0 | 0.80 | 1.445 | 1.400 | 3.114 | 1.445 | 0.000 | 1.447 | 0.138 | 1.424 | 1.453 | 1.404 | 2.837 |
| 180.0 | 0.83 | 1.449 | 1.402 | 3.244 | 1.448 | 0.069 | 1.450 | 0.069 | 1.426 | 1.587 | 1.407 | 2.899 |
| 185.0 | 0.85 | 1.453 | 1.405 | 3.304 | 1.451 | 0.138 | 1.453 | 0.000 | 1.429 | 1.652 | 1.409 | 3.028 |
| 190.0 | 0.87 | 1.453 | 1.408 | 3.097 | 1.454 | 0.069 | 1.456 | 0.206 | 1.432 | 1.445 | 1.412 | 2.822 |
| 195.0 | 0.90 | 1.458 | 1.410 | 3.292 | 1.457 | 0.069 | 1.459 | 0.069 | 1.434 | 1.646 | 1.415 | 2.949 |
| 200.0 | 0.92 | 1.462 | 1.413 | 3.352 | 1.460 | 0.137 | 1.461 | 0.068 | 1.437 | 1.710 | 1.417 | 3.078 |

**Table 2b.** Key properties of the pair correlation function resulting from Langevin dynamics simulations and five integral theory approaches: the hypernetted-chain approximation (HNC), isomorph-based empirically modified hypernetted-chain approximation (IEMHNC), variational modified hypernetted-chain approximation (VMHNC), Rogers-Young approximation (RY) and Ballone-Pastore-Galli-Gazzillo approximation (BPGG). The absolute relative deviation $\epsilon_{\mathrm{r}}$ between the theoretical and the simulation results is also reported. **Results for the magnitude of the first maximum in the case of $\boldsymbol{\kappa = 1}$**. The LD results are adopted from Table 5 of *T. Ott and M. Bonitz, Contrib. Plasma Phys.* **55**, *243 (2015).*

| $\Gamma$ | $\Gamma/\Gamma_{\mathrm{m}}$ | $g_{\mathrm{max1}}^{\mathrm{LD}}$ | $g_{\mathrm{max1}}^{\mathrm{HNC}}$ | $\epsilon_{\mathrm{HNC}}(\%)$ | $g_{\mathrm{max1}}^{\mathrm{IEMHNC}}$ | $\epsilon_{\mathrm{IEMHNC}}(\%)$ | $g_{\mathrm{max1}}^{\mathrm{VMHNC}}$ | $\epsilon_{\mathrm{VMHNC}}(\%)$ | $g_{\mathrm{max1}}^{\mathrm{RY}}$ | $\epsilon_{\mathrm{RY}}(\%)$ | $g_{\mathrm{max1}}^{\mathrm{BPGG}}$ | $\epsilon_{\mathrm{BPGG}}(\%)$ |
|---|---|---|---|---|---|---|---|---|---|---|---|---|
| 10.0 | 0.05 | 1.101 | 1.079 | 1.989 | 1.084 | 1.575 | 1.097 | 0.353 | 1.096 | 0.456 | 1.084 | 1.547 |
| 15.0 | 0.07 | 1.175 | 1.137 | 3.198 | 1.154 | 1.805 | 1.174 | 0.059 | 1.166 | 0.799 | 1.144 | 2.614 |
| 20.0 | 0.09 | 1.243 | 1.190 | 4.248 | 1.217 | 2.074 | 1.245 | 0.172 | 1.228 | 1.237 | 1.198 | 3.581 |
| 25.0 | 0.11 | 1.304 | 1.238 | 5.058 | 1.278 | 2.029 | 1.310 | 0.463 | 1.283 | 1.593 | 1.247 | 4.338 |
| 30.0 | 0.14 | 1.360 | 1.282 | 5.745 | 1.335 | 1.872 | 1.370 | 0.734 | 1.334 | 1.925 | 1.292 | 4.991 |
| 35.0 | 0.16 | 1.413 | 1.322 | 6.412 | 1.388 | 1.754 | 1.426 | 0.907 | 1.380 | 2.304 | 1.333 | 5.634 |
| 40.0 | 0.18 | 1.462 | 1.360 | 6.960 | 1.439 | 1.582 | 1.478 | 1.110 | 1.424 | 2.607 | 1.372 | 6.168 |
| 45.0 | 0.21 | 1.509 | 1.396 | 7.502 | 1.487 | 1.469 | 1.528 | 1.240 | 1.465 | 2.936 | 1.408 | 6.699 |
| 50.0 | 0.23 | 1.553 | 1.429 | 7.957 | 1.532 | 1.323 | 1.575 | 1.396 | 1.503 | 3.202 | 1.442 | 7.147 |
| 55.0 | 0.25 | 1.595 | 1.461 | 8.378 | 1.576 | 1.190 | 1.619 | 1.535 | 1.540 | 3.451 | 1.474 | 7.563 |
| 60.0 | 0.28 | 1.636 | 1.492 | 8.810 | 1.618 | 1.114 | 1.662 | 1.611 | 1.575 | 3.730 | 1.505 | 7.993 |
| 65.0 | 0.30 | 1.675 | 1.521 | 9.190 | 1.658 | 1.019 | 1.704 | 1.703 | 1.609 | 3.968 | 1.535 | 8.371 |
| 70.0 | 0.32 | 1.711 | 1.549 | 9.461 | 1.697 | 0.837 | 1.743 | 1.880 | 1.641 | 4.102 | 1.563 | 8.640 |
| 75.0 | 0.34 | 1.749 | 1.576 | 9.882 | 1.734 | 0.849 | 1.781 | 1.855 | 1.672 | 4.408 | 1.590 | 9.063 |
| 80.0 | 0.37 | 1.783 | 1.602 | 10.137 | 1.770 | 0.702 | 1.818 | 1.990 | 1.702 | 4.545 | 1.617 | 9.318 |
| 85.0 | 0.39 | 1.817 | 1.628 | 10.428 | 1.806 | 0.617 | 1.854 | 2.058 | 1.731 | 4.729 | 1.642 | 9.610 |
| 90.0 | 0.41 | 1.850 | 1.652 | 10.702 | 1.840 | 0.533 | 1.889 | 2.122 | 1.759 | 4.903 | 1.667 | 9.886 |
| 95.0 | 0.44 | 1.882 | 1.676 | 10.956 | 1.874 | 0.444 | 1.923 | 2.188 | 1.787 | 5.063 | 1.691 | 10.141 |
| 100.0 | 0.46 | 1.914 | 1.699 | 11.236 | 1.906 | 0.400 | 1.956 | 2.205 | 1.813 | 5.256 | 1.714 | 10.423 |
| 105.0 | 0.48 | 1.944 | 1.721 | 11.447 | 1.938 | 0.293 | 1.988 | 2.285 | 1.839 | 5.380 | 1.737 | 10.636 |
| 110.0 | 0.51 | 1.974 | 1.743 | 11.679 | 1.970 | 0.223 | 2.020 | 2.324 | 1.865 | 5.533 | 1.759 | 10.870 |
| 115.0 | 0.53 | 2.003 | 1.765 | 11.886 | 2.000 | 0.138 | 2.051 | 2.378 | 1.890 | 5.664 | 1.781 | 11.080 |
| 120.0 | 0.55 | 2.031 | 1.786 | 12.068 | 2.030 | 0.035 | 2.081 | 2.448 | 1.914 | 5.772 | 1.802 | 11.264 |
| 125.0 | 0.57 | 2.058 | 1.806 | 12.225 | 2.060 | 0.087 | 2.110 | 2.536 | 1.937 | 5.857 | 1.823 | 11.423 |
| 130.0 | 0.60 | 2.088 | 1.826 | 12.524 | 2.089 | 0.037 | 2.139 | 2.445 | 1.961 | 6.098 | 1.843 | 11.725 |
| 135.0 | 0.62 | 2.114 | 1.846 | 12.669 | 2.117 | 0.154 | 2.167 | 2.525 | 1.983 | 6.177 | 1.863 | 11.871 |
| 140.0 | 0.64 | 2.141 | 1.865 | 12.868 | 2.145 | 0.200 | 2.195 | 2.531 | 2.006 | 6.318 | 1.883 | 12.073 |
| 145.0 | 0.67 | 2.166 | 1.884 | 12.999 | 2.173 | 0.316 | 2.222 | 2.608 | 2.028 | 6.389 | 1.902 | 12.206 |
| 150.0 | 0.69 | 2.191 | 1.903 | 13.142 | 2.200 | 0.410 | 2.249 | 2.626 | 2.049 | 6.476 | 1.920 | 12.352 |
| 155.0 | 0.71 | 2.217 | 1.921 | 13.336 | 2.227 | 0.439 | 2.276 | 2.648 | 2.070 | 6.619 | 1.939 | 12.549 |
| 160.0 | 0.74 | 2.242 | 1.939 | 13.501 | 2.253 | 0.495 | 2.302 | 2.662 | 2.091 | 6.733 | 1.957 | 12.716 |
| 165.0 | 0.76 | 2.266 | 1.957 | 13.637 | 2.279 | 0.577 | 2.327 | 2.702 | 2.111 | 6.819 | 1.975 | 12.854 |
| 170.0 | 0.78 | 2.289 | 1.974 | 13.744 | 2.305 | 0.687 | 2.352 | 2.770 | 2.132 | 6.877 | 1.992 | 12.963 |
| 175.0 | 0.80 | 2.314 | 1.992 | 13.936 | 2.330 | 0.692 | 2.377 | 2.731 | 2.151 | 7.027 | 2.010 | 13.158 |
| 180.0 | 0.83 | 2.337 | 2.008 | 14.060 | 2.355 | 0.769 | 2.402 | 2.766 | 2.171 | 7.107 | 2.027 | 13.285 |
| 185.0 | 0.85 | 2.359 | 2.025 | 14.157 | 2.380 | 0.875 | 2.426 | 2.829 | 2.190 | 7.158 | 2.043 | 13.383 |
| 190.0 | 0.87 | 2.383 | 2.041 | 14.333 | 2.404 | 0.881 | 2.450 | 2.791 | 2.209 | 7.297 | 2.060 | 13.562 |
| 195.0 | 0.90 | 2.404 | 2.058 | 14.408 | 2.428 | 1.000 | 2.473 | 2.869 | 2.228 | 7.329 | 2.076 | 13.639 |
| 200.0 | 0.92 | 2.427 | 2.074 | 14.562 | 2.452 | 1.022 | 2.496 | 2.849 | 2.246 | 7.447 | 2.092 | 13.796 |

**Table 2c.** Key properties of the pair correlation function resulting from Langevin dynamics simulations and five integral theory approaches: the hypernetted-chain approximation (HNC), isomorph-based empirically modified hypernetted-chain approximation (IEMHNC), variational modified hypernetted-chain approximation (VMHNC), Rogers-Young approximation (RY) and Ballone-Pastore-Galli-Gazzillo approximation (BPGG). The absolute relative deviation $\epsilon_{\mathrm{r}}$ between the theoretical and the simulation results is also reported. **Results for the position of the first maximum in the case of $\boldsymbol{\kappa = 1}$**. The LD results are adopted from Table 5 of *T. Ott and M. Bonitz, Contrib. Plasma Phys.* **55***, 243 (2015).* Here $x = r/d$, where $d$ is the Wigner-Seitz radius.

| $\Gamma$ | $\Gamma/\Gamma_{\mathrm{m}}$ | $x^{\mathrm{LD}}_{\mathrm{max1}}$ | $x^{\mathrm{HNC}}_{\mathrm{max1}}$ | $\epsilon_{\mathrm{HNC}}(\%)$ | $x^{\mathrm{IEMHNC}}_{\mathrm{max1}}$ | $\epsilon_{\mathrm{IEMHNC}}(\%)$ | $x^{\mathrm{VMHNC}}_{\mathrm{max1}}$ | $\epsilon_{\mathrm{VMHNC}}(\%)$ | $x^{\mathrm{RY}}_{\mathrm{max1}}$ | $\epsilon_{\mathrm{RY}}(\%)$ | $x^{\mathrm{BPGG}}_{\mathrm{max1}}$ | $\epsilon_{\mathrm{BPGG}}(\%)$ |
|---|---|---|---|---|---|---|---|---|---|---|---|---|
| 10.0 | 0.05 | 1.660 | 1.666 | 0.361 | 1.664 | 0.241 | 1.635 | 1.506 | 1.646 | 0.843 | 1.671 | 0.663 |
| 15.0 | 0.07 | 1.648 | 1.643 | 0.303 | 1.659 | 0.667 | 1.624 | 1.456 | 1.631 | 1.032 | 1.650 | 0.121 |
| 20.0 | 0.09 | 1.648 | 1.637 | 0.667 | 1.657 | 0.546 | 1.627 | 1.274 | 1.631 | 1.032 | 1.645 | 0.182 |
| 25.0 | 0.11 | 1.650 | 1.636 | 0.848 | 1.656 | 0.364 | 1.632 | 1.091 | 1.633 | 1.030 | 1.644 | 0.364 |
| 30.0 | 0.14 | 1.655 | 1.637 | 1.088 | 1.656 | 0.060 | 1.638 | 1.027 | 1.636 | 1.148 | 1.645 | 0.604 |
| 35.0 | 0.16 | 1.659 | 1.639 | 1.206 | 1.658 | 0.060 | 1.644 | 0.904 | 1.639 | 1.206 | 1.647 | 0.723 |
| 40.0 | 0.18 | 1.662 | 1.641 | 1.264 | 1.660 | 0.120 | 1.650 | 0.722 | 1.642 | 1.203 | 1.649 | 0.782 |
| 45.0 | 0.21 | 1.666 | 1.643 | 1.381 | 1.662 | 0.240 | 1.655 | 0.660 | 1.645 | 1.261 | 1.651 | 0.900 |
| 50.0 | 0.23 | 1.669 | 1.646 | 1.378 | 1.665 | 0.240 | 1.660 | 0.539 | 1.648 | 1.258 | 1.653 | 0.959 |
| 55.0 | 0.25 | 1.673 | 1.648 | 1.494 | 1.667 | 0.359 | 1.664 | 0.538 | 1.651 | 1.315 | 1.655 | 1.076 |
| 60.0 | 0.28 | 1.676 | 1.650 | 1.551 | 1.669 | 0.418 | 1.668 | 0.477 | 1.654 | 1.313 | 1.657 | 1.134 |
| 65.0 | 0.30 | 1.679 | 1.652 | 1.608 | 1.672 | 0.417 | 1.672 | 0.417 | 1.656 | 1.370 | 1.659 | 1.191 |
| 70.0 | 0.32 | 1.681 | 1.654 | 1.606 | 1.674 | 0.416 | 1.676 | 0.297 | 1.659 | 1.309 | 1.661 | 1.190 |
| 75.0 | 0.34 | 1.684 | 1.656 | 1.663 | 1.677 | 0.416 | 1.679 | 0.297 | 1.661 | 1.366 | 1.662 | 1.306 |
| 80.0 | 0.37 | 1.687 | 1.658 | 1.719 | 1.679 | 0.474 | 1.682 | 0.296 | 1.663 | 1.423 | 1.664 | 1.363 |
| 85.0 | 0.39 | 1.689 | 1.660 | 1.717 | 1.681 | 0.474 | 1.685 | 0.237 | 1.665 | 1.421 | 1.666 | 1.362 |
| 90.0 | 0.41 | 1.691 | 1.662 | 1.715 | 1.683 | 0.473 | 1.688 | 0.177 | 1.667 | 1.419 | 1.667 | 1.419 |
| 95.0 | 0.44 | 1.693 | 1.663 | 1.772 | 1.685 | 0.473 | 1.691 | 0.118 | 1.669 | 1.418 | 1.669 | 1.418 |
| 100.0 | 0.46 | 1.695 | 1.665 | 1.770 | 1.687 | 0.472 | 1.694 | 0.059 | 1.671 | 1.416 | 1.671 | 1.416 |
| 105.0 | 0.48 | 1.697 | 1.667 | 1.768 | 1.689 | 0.471 | 1.696 | 0.059 | 1.673 | 1.414 | 1.672 | 1.473 |
| 110.0 | 0.51 | 1.699 | 1.668 | 1.825 | 1.691 | 0.471 | 1.698 | 0.059 | 1.675 | 1.413 | 1.673 | 1.530 |
| 115.0 | 0.53 | 1.701 | 1.670 | 1.822 | 1.693 | 0.470 | 1.701 | 0.000 | 1.676 | 1.470 | 1.675 | 1.529 |
| 120.0 | 0.55 | 1.702 | 1.671 | 1.821 | 1.695 | 0.411 | 1.703 | 0.059 | 1.678 | 1.410 | 1.676 | 1.528 |
| 125.0 | 0.57 | 1.704 | 1.672 | 1.878 | 1.696 | 0.469 | 1.705 | 0.059 | 1.680 | 1.408 | 1.677 | 1.585 |
| 130.0 | 0.60 | 1.706 | 1.674 | 1.876 | 1.698 | 0.469 | 1.707 | 0.059 | 1.681 | 1.465 | 1.679 | 1.583 |
| 135.0 | 0.62 | 1.707 | 1.675 | 1.875 | 1.700 | 0.410 | 1.709 | 0.117 | 1.682 | 1.465 | 1.680 | 1.582 |
| 140.0 | 0.64 | 1.709 | 1.676 | 1.931 | 1.701 | 0.468 | 1.710 | 0.059 | 1.684 | 1.463 | 1.681 | 1.638 |
| 145.0 | 0.67 | 1.710 | 1.677 | 1.930 | 1.703 | 0.409 | 1.712 | 0.117 | 1.685 | 1.462 | 1.682 | 1.637 |
| 150.0 | 0.69 | 1.712 | 1.679 | 1.928 | 1.704 | 0.467 | 1.714 | 0.117 | 1.686 | 1.519 | 1.683 | 1.694 |
| 155.0 | 0.71 | 1.713 | 1.680 | 1.926 | 1.706 | 0.409 | 1.715 | 0.117 | 1.688 | 1.459 | 1.684 | 1.693 |
| 160.0 | 0.74 | 1.715 | 1.681 | 1.983 | 1.707 | 0.466 | 1.717 | 0.117 | 1.689 | 1.516 | 1.685 | 1.749 |
| 165.0 | 0.76 | 1.715 | 1.682 | 1.924 | 1.709 | 0.350 | 1.718 | 0.175 | 1.690 | 1.458 | 1.686 | 1.691 |
| 170.0 | 0.78 | 1.717 | 1.683 | 1.980 | 1.710 | 0.408 | 1.720 | 0.175 | 1.691 | 1.514 | 1.687 | 1.747 |
| 175.0 | 0.80 | 1.718 | 1.684 | 1.979 | 1.711 | 0.407 | 1.721 | 0.175 | 1.692 | 1.513 | 1.688 | 1.746 |
| 180.0 | 0.83 | 1.719 | 1.685 | 1.978 | 1.713 | 0.349 | 1.723 | 0.233 | 1.693 | 1.513 | 1.689 | 1.745 |
| 185.0 | 0.85 | 1.720 | 1.686 | 1.977 | 1.714 | 0.349 | 1.724 | 0.233 | 1.694 | 1.512 | 1.690 | 1.744 |
| 190.0 | 0.87 | 1.721 | 1.687 | 1.976 | 1.715 | 0.349 | 1.725 | 0.232 | 1.695 | 1.511 | 1.691 | 1.743 |
| 195.0 | 0.90 | 1.722 | 1.688 | 1.974 | 1.716 | 0.348 | 1.727 | 0.290 | 1.696 | 1.510 | 1.692 | 1.742 |
| 200.0 | 0.92 | 1.723 | 1.689 | 1.973 | 1.717 | 0.348 | 1.728 | 0.290 | 1.697 | 1.509 | 1.693 | 1.741 |

**Table 2d.** Key properties of the pair correlation function resulting from Langevin dynamics simulations and five integral theory approaches: the hypernetted-chain approximation (HNC), isomorph-based empirically modified hypernetted-chain approximation (IEMHNC), variational modified hypernetted-chain approximation (VMHNC), Rogers-Young approximation (RY) and Ballone-Pastore-Galli-Gazzillo approximation (BPGG). The absolute relative deviation $\epsilon_{\mathrm{r}}$ between the theoretical and the simulation results is also reported. **Results for the magnitude of the first minimum in the case of $\boldsymbol{\kappa=1}$**. The LD results are adopted from Table 5 of *T. Ott and M. Bonitz, Contrib. Plasma Phys.* **55**, *243 (2015).*

| $\Gamma$ | $\Gamma/\Gamma_{\mathrm{m}}$ | $g_{\mathrm{min1}}^{\mathrm{LD}}$ | $g_{\mathrm{min1}}^{\mathrm{HNC}}$ | $\epsilon_{\mathrm{HNC}}(\%)$ | $g_{\mathrm{min1}}^{\mathrm{IEMHNC}}$ | $\epsilon_{\mathrm{IEMHNC}}(\%)$ | $g_{\mathrm{min1}}^{\mathrm{VMHNC}}$ | $\epsilon_{\mathrm{VMHNC}}(\%)$ | $g_{\mathrm{min1}}^{\mathrm{RY}}$ | $\epsilon_{\mathrm{RY}}(\%)$ | $g_{\mathrm{min1}}^{\mathrm{BPGG}}$ | $\epsilon_{\mathrm{BPGG}}(\%)$ |
|---|---|---|---|---|---|---|---|---|---|---|---|---|
| 10.0 | 0.05 | 0.987 | 0.992 | 0.525 | 0.991 | 0.429 | 0.990 | 0.271 | 0.989 | 0.201 | 0.991 | 0.407 |
| 15.0 | 0.07 | 0.969 | 0.980 | 1.162 | 0.973 | 0.447 | 0.973 | 0.421 | 0.973 | 0.416 | 0.978 | 0.934 |
| 20.0 | 0.09 | 0.948 | 0.967 | 1.965 | 0.955 | 0.707 | 0.953 | 0.578 | 0.956 | 0.797 | 0.964 | 1.636 |
| 25.0 | 0.11 | 0.927 | 0.953 | 2.768 | 0.936 | 0.937 | 0.933 | 0.643 | 0.938 | 1.217 | 0.949 | 2.352 |
| 30.0 | 0.14 | 0.907 | 0.939 | 3.525 | 0.917 | 1.096 | 0.913 | 0.660 | 0.922 | 1.632 | 0.935 | 3.035 |
| 35.0 | 0.16 | 0.887 | 0.926 | 4.375 | 0.899 | 1.349 | 0.894 | 0.789 | 0.906 | 2.176 | 0.921 | 3.821 |
| 40.0 | 0.18 | 0.869 | 0.913 | 5.095 | 0.882 | 1.493 | 0.876 | 0.817 | 0.892 | 2.624 | 0.908 | 4.487 |
| 45.0 | 0.21 | 0.853 | 0.901 | 5.672 | 0.866 | 1.523 | 0.859 | 0.737 | 0.878 | 2.959 | 0.896 | 5.018 |
| 50.0 | 0.23 | 0.836 | 0.890 | 6.474 | 0.851 | 1.792 | 0.843 | 0.895 | 0.866 | 3.534 | 0.884 | 5.779 |
| 55.0 | 0.25 | 0.822 | 0.879 | 6.991 | 0.837 | 1.809 | 0.829 | 0.802 | 0.854 | 3.849 | 0.873 | 6.261 |
| 60.0 | 0.28 | 0.807 | 0.869 | 7.728 | 0.824 | 2.052 | 0.815 | 0.933 | 0.842 | 4.392 | 0.863 | 6.965 |
| 65.0 | 0.30 | 0.794 | 0.860 | 8.285 | 0.811 | 2.139 | 0.801 | 0.907 | 0.832 | 4.771 | 0.854 | 7.494 |
| 70.0 | 0.32 | 0.781 | 0.851 | 8.921 | 0.799 | 2.313 | 0.789 | 0.967 | 0.822 | 5.236 | 0.844 | 8.104 |
| 75.0 | 0.34 | 0.769 | 0.842 | 9.493 | 0.788 | 2.435 | 0.776 | 0.974 | 0.812 | 5.648 | 0.836 | 8.653 |
| 80.0 | 0.37 | 0.758 | 0.834 | 9.991 | 0.777 | 2.495 | 0.765 | 0.921 | 0.803 | 5.994 | 0.827 | 9.131 |
| 85.0 | 0.39 | 0.747 | 0.826 | 10.553 | 0.767 | 2.621 | 0.754 | 0.930 | 0.795 | 6.407 | 0.819 | 9.674 |
| 90.0 | 0.41 | 0.736 | 0.818 | 11.178 | 0.757 | 2.809 | 0.743 | 1.000 | 0.787 | 6.886 | 0.812 | 10.280 |
| 95.0 | 0.44 | 0.726 | 0.811 | 11.711 | 0.747 | 2.915 | 0.733 | 0.988 | 0.779 | 7.279 | 0.804 | 10.797 |
| 100.0 | 0.46 | 0.716 | 0.804 | 12.300 | 0.738 | 3.073 | 0.723 | 1.027 | 0.771 | 7.729 | 0.797 | 11.369 |
| 105.0 | 0.48 | 0.707 | 0.797 | 12.783 | 0.729 | 3.137 | 0.714 | 0.972 | 0.764 | 8.081 | 0.791 | 11.838 |
| 110.0 | 0.51 | 0.698 | 0.791 | 13.315 | 0.721 | 3.245 | 0.705 | 0.960 | 0.757 | 8.481 | 0.784 | 12.355 |
| 115.0 | 0.53 | 0.689 | 0.785 | 13.894 | 0.712 | 3.395 | 0.696 | 0.989 | 0.751 | 8.929 | 0.778 | 12.920 |
| 120.0 | 0.55 | 0.681 | 0.779 | 14.351 | 0.704 | 3.437 | 0.687 | 0.909 | 0.744 | 9.263 | 0.772 | 13.365 |
| 125.0 | 0.57 | 0.672 | 0.773 | 15.020 | 0.697 | 3.668 | 0.679 | 1.015 | 0.738 | 9.800 | 0.766 | 14.019 |
| 130.0 | 0.60 | 0.664 | 0.767 | 15.561 | 0.689 | 3.783 | 0.671 | 1.005 | 0.732 | 10.216 | 0.761 | 14.548 |
| 135.0 | 0.62 | 0.657 | 0.762 | 15.965 | 0.682 | 3.774 | 0.663 | 0.874 | 0.726 | 10.504 | 0.755 | 14.940 |
| 140.0 | 0.64 | 0.649 | 0.757 | 16.583 | 0.675 | 3.955 | 0.655 | 0.927 | 0.720 | 10.996 | 0.750 | 15.545 |
| 145.0 | 0.67 | 0.642 | 0.752 | 17.057 | 0.668 | 4.007 | 0.647 | 0.853 | 0.715 | 11.353 | 0.745 | 16.008 |
| 150.0 | 0.69 | 0.634 | 0.747 | 17.750 | 0.661 | 4.252 | 0.640 | 1.009 | 0.710 | 11.919 | 0.740 | 16.688 |
| 155.0 | 0.71 | 0.627 | 0.742 | 18.294 | 0.654 | 4.362 | 0.633 | 0.944 | 0.704 | 12.344 | 0.735 | 17.220 |
| 160.0 | 0.74 | 0.620 | 0.737 | 18.870 | 0.648 | 4.500 | 0.626 | 0.948 | 0.699 | 12.801 | 0.730 | 17.784 |
| 165.0 | 0.76 | 0.614 | 0.732 | 19.286 | 0.642 | 4.495 | 0.619 | 0.812 | 0.694 | 13.106 | 0.726 | 18.189 |
| 170.0 | 0.78 | 0.608 | 0.728 | 19.728 | 0.635 | 4.513 | 0.612 | 0.697 | 0.690 | 13.438 | 0.721 | 18.621 |
| 175.0 | 0.80 | 0.601 | 0.724 | 20.398 | 0.629 | 4.727 | 0.606 | 0.769 | 0.685 | 13.986 | 0.717 | 19.278 |
| 180.0 | 0.83 | 0.595 | 0.719 | 20.898 | 0.624 | 4.791 | 0.599 | 0.695 | 0.681 | 14.373 | 0.713 | 19.767 |
| 185.0 | 0.85 | 0.588 | 0.715 | 21.631 | 0.618 | 5.056 | 0.593 | 0.811 | 0.676 | 14.982 | 0.708 | 20.486 |
| 190.0 | 0.87 | 0.582 | 0.711 | 22.188 | 0.612 | 5.166 | 0.587 | 0.776 | 0.672 | 15.425 | 0.704 | 21.032 |
| 195.0 | 0.90 | 0.577 | 0.707 | 22.559 | 0.607 | 5.115 | 0.580 | 0.584 | 0.668 | 15.693 | 0.700 | 21.393 |
| 200.0 | 0.92 | 0.571 | 0.703 | 23.168 | 0.601 | 5.266 | 0.574 | 0.585 | 0.663 | 16.186 | 0.697 | 21.989 |

**Table 2e.** Key properties of the pair correlation function resulting from Langevin dynamics simulations and five integral theory approaches: the hypernetted-chain approximation (HNC), isomorph-based empirically modified hypernetted-chain approximation (IEMHNC), variational modified hypernetted-chain approximation (VMHNC), Rogers-Young approximation (RY) and Ballone-Pastore-Galli-Gazzillo approximation (BPGG). The absolute relative deviation $\epsilon_{\mathrm{r}}$ between the theoretical and the simulation results is also reported. **Results for the position of the first minimum in the case of $\boldsymbol{\kappa = 1}$**. The LD results are adopted from Table 5 of *T. Ott and M. Bonitz, Contrib. Plasma Phys.* **55**, *243 (2015)*. Here $x = r/d$, where $d$ is the Wigner-Seitz radius.

| $\Gamma$ | $\Gamma/\Gamma_{\mathrm{m}}$ | $x_{\mathrm{min1}}^{\mathrm{LD}}$ | $x_{\mathrm{min1}}^{\mathrm{HNC}}$ | $\epsilon_{\mathrm{HNC}}(\%)$ | $x_{\mathrm{min1}}^{\mathrm{IEMHNC}}$ | $\epsilon_{\mathrm{IEMHNC}}(\%)$ | $x_{\mathrm{min1}}^{\mathrm{VMHNC}}$ | $\epsilon_{\mathrm{VMHNC}}(\%)$ | $x_{\mathrm{min1}}^{\mathrm{RY}}$ | $\epsilon_{\mathrm{RY}}(\%)$ | $x_{\mathrm{min1}}^{\mathrm{BPGG}}$ | $\epsilon_{\mathrm{BPGG}}(\%)$ |
|---|---|---|---|---|---|---|---|---|---|---|---|---|
| 10.0 | 0.05 | 2.520 | 2.594 | 2.937 | 2.576 | 2.222 | 2.529 | 0.357 | 2.541 | 0.833 | 2.600 | 3.175 |
| 15.0 | 0.07 | 2.482 | 2.523 | 1.652 | 2.526 | 1.773 | 2.470 | 0.483 | 2.489 | 0.282 | 2.533 | 2.055 |
| 20.0 | 0.09 | 2.464 | 2.495 | 1.258 | 2.505 | 1.664 | 2.435 | 1.177 | 2.473 | 0.365 | 2.507 | 1.745 |
| 25.0 | 0.11 | 2.457 | 2.483 | 1.058 | 2.489 | 1.302 | 2.427 | 1.221 | 2.467 | 0.407 | 2.496 | 1.587 |
| 30.0 | 0.14 | 2.454 | 2.477 | 0.937 | 2.479 | 1.019 | 2.425 | 1.182 | 2.466 | 0.489 | 2.489 | 1.426 |
| 35.0 | 0.16 | 2.452 | 2.474 | 0.897 | 2.473 | 0.856 | 2.425 | 1.101 | 2.466 | 0.571 | 2.486 | 1.387 |
| 40.0 | 0.18 | 2.452 | 2.473 | 0.856 | 2.469 | 0.693 | 2.425 | 1.101 | 2.466 | 0.571 | 2.485 | 1.346 |
| 45.0 | 0.21 | 2.454 | 2.472 | 0.733 | 2.467 | 0.530 | 2.425 | 1.182 | 2.467 | 0.530 | 2.484 | 1.222 |
| 50.0 | 0.23 | 2.452 | 2.472 | 0.816 | 2.465 | 0.530 | 2.425 | 1.101 | 2.468 | 0.653 | 2.483 | 1.264 |
| 55.0 | 0.25 | 2.452 | 2.472 | 0.816 | 2.464 | 0.489 | 2.424 | 1.142 | 2.468 | 0.653 | 2.483 | 1.264 |
| 60.0 | 0.28 | 2.452 | 2.473 | 0.856 | 2.462 | 0.408 | 2.423 | 1.183 | 2.469 | 0.693 | 2.483 | 1.264 |
| 65.0 | 0.30 | 2.452 | 2.473 | 0.856 | 2.461 | 0.367 | 2.422 | 1.223 | 2.469 | 0.693 | 2.483 | 1.264 |
| 70.0 | 0.32 | 2.451 | 2.473 | 0.898 | 2.460 | 0.367 | 2.420 | 1.265 | 2.469 | 0.734 | 2.482 | 1.265 |
| 75.0 | 0.34 | 2.450 | 2.473 | 0.939 | 2.458 | 0.327 | 2.418 | 1.306 | 2.469 | 0.776 | 2.482 | 1.306 |
| 80.0 | 0.37 | 2.449 | 2.473 | 0.980 | 2.457 | 0.327 | 2.417 | 1.307 | 2.469 | 0.817 | 2.482 | 1.347 |
| 85.0 | 0.39 | 2.448 | 2.473 | 1.021 | 2.456 | 0.327 | 2.415 | 1.348 | 2.468 | 0.817 | 2.481 | 1.348 |
| 90.0 | 0.41 | 2.447 | 2.473 | 1.063 | 2.454 | 0.286 | 2.412 | 1.430 | 2.468 | 0.858 | 2.481 | 1.389 |
| 95.0 | 0.44 | 2.446 | 2.473 | 1.104 | 2.453 | 0.286 | 2.410 | 1.472 | 2.467 | 0.859 | 2.480 | 1.390 |
| 100.0 | 0.46 | 2.445 | 2.473 | 1.145 | 2.451 | 0.245 | 2.408 | 1.513 | 2.466 | 0.859 | 2.480 | 1.431 |
| 105.0 | 0.48 | 2.443 | 2.472 | 1.187 | 2.450 | 0.287 | 2.406 | 1.515 | 2.465 | 0.901 | 2.479 | 1.474 |
| 110.0 | 0.51 | 2.442 | 2.472 | 1.229 | 2.448 | 0.246 | 2.403 | 1.597 | 2.464 | 0.901 | 2.478 | 1.474 |
| 115.0 | 0.53 | 2.442 | 2.471 | 1.188 | 2.446 | 0.164 | 2.401 | 1.679 | 2.463 | 0.860 | 2.478 | 1.474 |
| 120.0 | 0.55 | 2.440 | 2.471 | 1.270 | 2.445 | 0.205 | 2.399 | 1.680 | 2.463 | 0.943 | 2.477 | 1.516 |
| 125.0 | 0.57 | 2.438 | 2.470 | 1.313 | 2.443 | 0.205 | 2.397 | 1.682 | 2.462 | 0.984 | 2.476 | 1.559 |
| 130.0 | 0.60 | 2.437 | 2.469 | 1.313 | 2.442 | 0.205 | 2.394 | 1.764 | 2.460 | 0.944 | 2.475 | 1.559 |
| 135.0 | 0.62 | 2.437 | 2.469 | 1.313 | 2.440 | 0.123 | 2.392 | 1.847 | 2.459 | 0.903 | 2.474 | 1.518 |
| 140.0 | 0.64 | 2.436 | 2.468 | 1.314 | 2.439 | 0.123 | 2.390 | 1.888 | 2.458 | 0.903 | 2.473 | 1.519 |
| 145.0 | 0.67 | 2.434 | 2.467 | 1.356 | 2.437 | 0.123 | 2.388 | 1.890 | 2.457 | 0.945 | 2.472 | 1.561 |
| 150.0 | 0.69 | 2.432 | 2.466 | 1.398 | 2.436 | 0.164 | 2.386 | 1.891 | 2.456 | 0.987 | 2.472 | 1.645 |
| 155.0 | 0.71 | 2.432 | 2.466 | 1.398 | 2.434 | 0.082 | 2.383 | 2.015 | 2.455 | 0.946 | 2.471 | 1.604 |
| 160.0 | 0.74 | 2.430 | 2.465 | 1.440 | 2.433 | 0.123 | 2.381 | 2.016 | 2.454 | 0.988 | 2.470 | 1.646 |
| 165.0 | 0.76 | 2.429 | 2.464 | 1.441 | 2.431 | 0.082 | 2.379 | 2.058 | 2.453 | 0.988 | 2.469 | 1.647 |
| 170.0 | 0.78 | 2.428 | 2.463 | 1.442 | 2.430 | 0.082 | 2.377 | 2.100 | 2.452 | 0.988 | 2.468 | 1.647 |
| 175.0 | 0.80 | 2.427 | 2.462 | 1.442 | 2.428 | 0.041 | 2.375 | 2.143 | 2.451 | 0.989 | 2.467 | 1.648 |
| 180.0 | 0.83 | 2.426 | 2.462 | 1.484 | 2.427 | 0.041 | 2.373 | 2.185 | 2.450 | 0.989 | 2.466 | 1.649 |
| 185.0 | 0.85 | 2.425 | 2.461 | 1.485 | 2.426 | 0.041 | 2.371 | 2.227 | 2.448 | 0.948 | 2.465 | 1.649 |
| 190.0 | 0.87 | 2.424 | 2.460 | 1.485 | 2.425 | 0.041 | 2.369 | 2.269 | 2.447 | 0.949 | 2.464 | 1.650 |
| 195.0 | 0.90 | 2.423 | 2.459 | 1.486 | 2.423 | 0.000 | 2.367 | 2.311 | 2.446 | 0.949 | 2.463 | 1.651 |
| 200.0 | 0.92 | 2.422 | 2.458 | 1.486 | 2.422 | 0.000 | 2.366 | 2.312 | 2.445 | 0.950 | 2.462 | 1.652 |

**Table 2f.** Key properties of the pair correlation function resulting from Langevin dynamics simulations and five integral theory approaches: the hypernetted-chain approximation (HNC), isomorph-based empirically modified hypernetted-chain approximation (IEMHNC), variational modified hypernetted-chain approximation (VMHNC), Rogers-Young approximation (RY) and Ballone-Pastore-Galli-Gazzillo approximation (BPGG). The absolute relative deviation $\epsilon_{\mathrm{r}}$ between the theoretical and the simulation results is also reported. **Results for the magnitude of the second maximum in the case of $\boldsymbol{\kappa = 1}$**. The LD results are adopted from Table 5 of *T. Ott and M. Bonitz, Contrib. Plasma Phys.* **55**, *243 (2015)*.

| $\Gamma$ | $\Gamma/\Gamma_{\mathrm{m}}$ | $g_{\max 2}^{\mathrm{LD}}$ | $g_{\max 2}^{\mathrm{HNC}}$ | $\epsilon_{\mathrm{HNC}}(\%)$ | $g_{\max 2}^{\mathrm{IEMHNC}}$ | $\epsilon_{\mathrm{IEMHNC}}(\%)$ | $g_{\max 2}^{\mathrm{VMHNC}}$ | $\epsilon_{\mathrm{VMHNC}}(\%)$ | $g_{\max 2}^{\mathrm{RY}}$ | $\epsilon_{\mathrm{RY}}(\%)$ | $g_{\max 2}^{\mathrm{BPGG}}$ | $\epsilon_{\mathrm{BPGG}}(\%)$ |
|---|---|---|---|---|---|---|---|---|---|---|---|---|
| 10.0 | 0.05 | 1.002 | 1.001 | 0.110 | 1.001 | 0.093 | 1.001 | 0.069 | 1.001 | 0.052 | 1.001 | 0.088 |
| 15.0 | 0.07 | 1.007 | 1.003 | 0.362 | 1.005 | 0.152 | 1.005 | 0.169 | 1.005 | 0.172 | 1.004 | 0.301 |
| 20.0 | 0.09 | 1.014 | 1.007 | 0.680 | 1.012 | 0.245 | 1.012 | 0.230 | 1.011 | 0.320 | 1.008 | 0.574 |
| 25.0 | 0.11 | 1.022 | 1.012 | 1.004 | 1.019 | 0.309 | 1.020 | 0.229 | 1.017 | 0.460 | 1.013 | 0.852 |
| 30.0 | 0.14 | 1.031 | 1.017 | 1.361 | 1.027 | 0.372 | 1.029 | 0.222 | 1.024 | 0.633 | 1.019 | 1.167 |
| 35.0 | 0.16 | 1.041 | 1.023 | 1.770 | 1.036 | 0.466 | 1.038 | 0.250 | 1.032 | 0.864 | 1.025 | 1.537 |
| 40.0 | 0.18 | 1.050 | 1.028 | 2.053 | 1.046 | 0.424 | 1.048 | 0.147 | 1.040 | 0.976 | 1.031 | 1.786 |
| 45.0 | 0.21 | 1.060 | 1.034 | 2.409 | 1.055 | 0.453 | 1.059 | 0.123 | 1.048 | 1.170 | 1.038 | 2.112 |
| 50.0 | 0.23 | 1.070 | 1.041 | 2.749 | 1.065 | 0.468 | 1.069 | 0.093 | 1.055 | 1.357 | 1.044 | 2.425 |
| 55.0 | 0.25 | 1.080 | 1.047 | 3.079 | 1.075 | 0.477 | 1.079 | 0.067 | 1.063 | 1.540 | 1.051 | 2.731 |
| 60.0 | 0.28 | 1.090 | 1.053 | 3.400 | 1.085 | 0.485 | 1.089 | 0.050 | 1.071 | 1.723 | 1.057 | 3.031 |
| 65.0 | 0.30 | 1.100 | 1.059 | 3.716 | 1.095 | 0.495 | 1.100 | 0.045 | 1.079 | 1.908 | 1.063 | 3.329 |
| 70.0 | 0.32 | 1.109 | 1.065 | 3.943 | 1.104 | 0.420 | 1.109 | 0.035 | 1.087 | 2.008 | 1.070 | 3.539 |
| 75.0 | 0.34 | 1.118 | 1.071 | 4.168 | 1.114 | 0.352 | 1.119 | 0.097 | 1.094 | 2.113 | 1.076 | 3.750 |
| 80.0 | 0.37 | 1.127 | 1.077 | 4.394 | 1.124 | 0.292 | 1.129 | 0.140 | 1.102 | 2.225 | 1.082 | 3.964 |
| 85.0 | 0.39 | 1.137 | 1.084 | 4.705 | 1.133 | 0.330 | 1.138 | 0.076 | 1.109 | 2.429 | 1.089 | 4.264 |
| 90.0 | 0.41 | 1.145 | 1.089 | 4.849 | 1.143 | 0.201 | 1.147 | 0.169 | 1.117 | 2.469 | 1.095 | 4.398 |
| 95.0 | 0.44 | 1.153 | 1.095 | 4.997 | 1.152 | 0.084 | 1.156 | 0.242 | 1.124 | 2.516 | 1.101 | 4.537 |
| 100.0 | 0.46 | 1.162 | 1.101 | 5.229 | 1.161 | 0.064 | 1.164 | 0.208 | 1.131 | 2.655 | 1.107 | 4.763 |
| 105.0 | 0.48 | 1.170 | 1.107 | 5.383 | 1.170 | 0.031 | 1.173 | 0.243 | 1.138 | 2.719 | 1.113 | 4.910 |
| 110.0 | 0.51 | 1.178 | 1.113 | 5.540 | 1.179 | 0.115 | 1.181 | 0.258 | 1.145 | 2.790 | 1.118 | 5.062 |
| 115.0 | 0.53 | 1.185 | 1.118 | 5.621 | 1.188 | 0.272 | 1.189 | 0.340 | 1.152 | 2.787 | 1.124 | 5.138 |
| 120.0 | 0.55 | 1.193 | 1.124 | 5.786 | 1.197 | 0.332 | 1.197 | 0.320 | 1.159 | 2.874 | 1.130 | 5.299 |
| 125.0 | 0.57 | 1.200 | 1.129 | 5.876 | 1.206 | 0.466 | 1.204 | 0.367 | 1.165 | 2.887 | 1.135 | 5.385 |
| 130.0 | 0.60 | 1.207 | 1.135 | 5.970 | 1.214 | 0.587 | 1.212 | 0.397 | 1.172 | 2.909 | 1.141 | 5.477 |
| 135.0 | 0.62 | 1.214 | 1.140 | 6.069 | 1.222 | 0.697 | 1.219 | 0.410 | 1.178 | 2.939 | 1.146 | 5.573 |
| 140.0 | 0.64 | 1.220 | 1.146 | 6.095 | 1.231 | 0.877 | 1.226 | 0.490 | 1.185 | 2.897 | 1.152 | 5.597 |
| 145.0 | 0.67 | 1.227 | 1.151 | 6.202 | 1.239 | 0.964 | 1.233 | 0.472 | 1.191 | 2.942 | 1.157 | 5.703 |
| 150.0 | 0.69 | 1.233 | 1.156 | 6.238 | 1.247 | 1.122 | 1.239 | 0.508 | 1.197 | 2.916 | 1.162 | 5.738 |
| 155.0 | 0.71 | 1.239 | 1.161 | 6.278 | 1.255 | 1.267 | 1.246 | 0.556 | 1.203 | 2.898 | 1.167 | 5.778 |
| 160.0 | 0.74 | 1.246 | 1.166 | 6.399 | 1.262 | 1.321 | 1.252 | 0.496 | 1.209 | 2.966 | 1.173 | 5.898 |
| 165.0 | 0.76 | 1.251 | 1.171 | 6.373 | 1.270 | 1.525 | 1.258 | 0.584 | 1.215 | 2.884 | 1.178 | 5.872 |
| 170.0 | 0.78 | 1.256 | 1.176 | 6.353 | 1.278 | 1.718 | 1.264 | 0.659 | 1.221 | 2.811 | 1.183 | 5.852 |
| 175.0 | 0.80 | 1.262 | 1.181 | 6.411 | 1.285 | 1.820 | 1.270 | 0.640 | 1.226 | 2.822 | 1.187 | 5.912 |
| 180.0 | 0.83 | 1.267 | 1.186 | 6.400 | 1.292 | 1.991 | 1.276 | 0.689 | 1.232 | 2.764 | 1.192 | 5.901 |
| 185.0 | 0.85 | 1.272 | 1.191 | 6.394 | 1.299 | 2.151 | 1.281 | 0.726 | 1.237 | 2.712 | 1.197 | 5.896 |
| 190.0 | 0.87 | 1.277 | 1.195 | 6.393 | 1.306 | 2.301 | 1.287 | 0.753 | 1.243 | 2.667 | 1.202 | 5.895 |
| 195.0 | 0.90 | 1.281 | 1.200 | 6.323 | 1.313 | 2.520 | 1.292 | 0.846 | 1.248 | 2.554 | 1.206 | 5.826 |
| 200.0 | 0.92 | 1.286 | 1.205 | 6.330 | 1.320 | 2.649 | 1.297 | 0.849 | 1.254 | 2.522 | 1.211 | 5.835 |

**Table 2g.** Key properties of the pair correlation function resulting from Langevin dynamics simulations and five integral theory approaches: the hypernetted-chain approximation (HNC), isomorph-based empirically modified hypernetted-chain approximation (IEMHNC), variational modified hypernetted-chain approximation (VMHNC), Rogers-Young approximation (RY) and Ballone-Pastore-Galli-Gazzillo approximation (BPGG). The absolute relative deviation $\epsilon_{\mathrm{r}}$ between the theoretical and the simulation results is also reported. **Results for the position of the second maximum in the case of $\boldsymbol{\kappa = 1}$**. The LD results are adopted from Table 5 of *T. Ott and M. Bonitz, Contrib. Plasma Phys.* **55**, *243 (2015)*. Here $x = r/d$, where $d$ is the Wigner-Seitz radius.

| $\Gamma$ | $\Gamma/\Gamma_{\mathrm{m}}$ | $x_{\mathrm{max2}}^{\mathrm{LD}}$ | $x_{\mathrm{max2}}^{\mathrm{HNC}}$ | $\epsilon_{\mathrm{HNC}}(\%)$ | $x_{\mathrm{max2}}^{\mathrm{IEMHNC}}$ | $\epsilon_{\mathrm{IEMHNC}}(\%)$ | $x_{\mathrm{max2}}^{\mathrm{VMHNC}}$ | $\epsilon_{\mathrm{VMHNC}}(\%)$ | $x_{\mathrm{max2}}^{\mathrm{RY}}$ | $\epsilon_{\mathrm{RY}}(\%)$ | $x_{\mathrm{max2}}^{\mathrm{BPGG}}$ | $\epsilon_{\mathrm{BPGG}}(\%)$ |
|---|---|---|---|---|---|---|---|---|---|---|---|---|
| 10.0 | 0.05 | 1.660 | 1.666 | 0.361 | 1.664 | 0.241 | 1.635 | 1.506 | 1.646 | 0.843 | 1.671 | 0.663 |
| 15.0 | 0.07 | 1.648 | 1.643 | 0.303 | 1.659 | 0.667 | 1.624 | 1.456 | 1.631 | 1.032 | 1.650 | 0.121 |
| 20.0 | 0.09 | 1.648 | 1.637 | 0.667 | 1.657 | 0.546 | 1.627 | 1.274 | 1.631 | 1.032 | 1.645 | 0.182 |
| 25.0 | 0.11 | 1.650 | 1.636 | 0.848 | 1.656 | 0.364 | 1.632 | 1.091 | 1.633 | 1.030 | 1.644 | 0.364 |
| 30.0 | 0.14 | 1.655 | 1.637 | 1.088 | 1.656 | 0.060 | 1.638 | 1.027 | 1.636 | 1.148 | 1.645 | 0.604 |
| 35.0 | 0.16 | 1.659 | 1.639 | 1.206 | 1.658 | 0.060 | 1.644 | 0.904 | 1.639 | 1.206 | 1.647 | 0.723 |
| 40.0 | 0.18 | 1.662 | 1.641 | 1.264 | 1.660 | 0.120 | 1.650 | 0.722 | 1.642 | 1.203 | 1.649 | 0.782 |
| 45.0 | 0.21 | 1.666 | 1.643 | 1.381 | 1.662 | 0.240 | 1.655 | 0.660 | 1.645 | 1.261 | 1.651 | 0.900 |
| 50.0 | 0.23 | 1.669 | 1.646 | 1.378 | 1.665 | 0.240 | 1.660 | 0.539 | 1.648 | 1.258 | 1.653 | 0.959 |
| 55.0 | 0.25 | 1.673 | 1.648 | 1.494 | 1.667 | 0.359 | 1.664 | 0.538 | 1.651 | 1.315 | 1.655 | 1.076 |
| 60.0 | 0.28 | 1.676 | 1.650 | 1.551 | 1.669 | 0.418 | 1.668 | 0.477 | 1.654 | 1.313 | 1.657 | 1.134 |
| 65.0 | 0.30 | 1.679 | 1.652 | 1.608 | 1.672 | 0.417 | 1.672 | 0.417 | 1.656 | 1.370 | 1.659 | 1.191 |
| 70.0 | 0.32 | 1.681 | 1.654 | 1.606 | 1.674 | 0.416 | 1.676 | 0.297 | 1.659 | 1.309 | 1.661 | 1.190 |
| 75.0 | 0.34 | 1.684 | 1.656 | 1.663 | 1.677 | 0.416 | 1.679 | 0.297 | 1.661 | 1.366 | 1.662 | 1.306 |
| 80.0 | 0.37 | 1.687 | 1.658 | 1.719 | 1.679 | 0.474 | 1.682 | 0.296 | 1.663 | 1.423 | 1.664 | 1.363 |
| 85.0 | 0.39 | 1.689 | 1.660 | 1.717 | 1.681 | 0.474 | 1.685 | 0.237 | 1.665 | 1.421 | 1.666 | 1.362 |
| 90.0 | 0.41 | 1.691 | 1.662 | 1.715 | 1.683 | 0.473 | 1.688 | 0.177 | 1.667 | 1.419 | 1.667 | 1.419 |
| 95.0 | 0.44 | 1.693 | 1.663 | 1.772 | 1.685 | 0.473 | 1.691 | 0.118 | 1.669 | 1.418 | 1.669 | 1.418 |
| 100.0 | 0.46 | 1.695 | 1.665 | 1.770 | 1.687 | 0.472 | 1.694 | 0.059 | 1.671 | 1.416 | 1.671 | 1.416 |
| 105.0 | 0.48 | 1.697 | 1.667 | 1.768 | 1.689 | 0.471 | 1.696 | 0.059 | 1.673 | 1.414 | 1.672 | 1.473 |
| 110.0 | 0.51 | 1.699 | 1.668 | 1.825 | 1.691 | 0.471 | 1.698 | 0.059 | 1.675 | 1.413 | 1.673 | 1.530 |
| 115.0 | 0.53 | 1.701 | 1.670 | 1.822 | 1.693 | 0.470 | 1.701 | 0.000 | 1.676 | 1.470 | 1.675 | 1.529 |
| 120.0 | 0.55 | 1.702 | 1.671 | 1.821 | 1.695 | 0.411 | 1.703 | 0.059 | 1.678 | 1.410 | 1.676 | 1.528 |
| 125.0 | 0.57 | 1.704 | 1.672 | 1.878 | 1.696 | 0.469 | 1.705 | 0.059 | 1.680 | 1.408 | 1.677 | 1.585 |
| 130.0 | 0.60 | 1.706 | 1.674 | 1.876 | 1.698 | 0.469 | 1.707 | 0.059 | 1.681 | 1.465 | 1.679 | 1.583 |
| 135.0 | 0.62 | 1.707 | 1.675 | 1.875 | 1.700 | 0.410 | 1.709 | 0.117 | 1.682 | 1.465 | 1.680 | 1.582 |
| 140.0 | 0.64 | 1.709 | 1.676 | 1.931 | 1.701 | 0.468 | 1.710 | 0.059 | 1.684 | 1.463 | 1.681 | 1.638 |
| 145.0 | 0.67 | 1.710 | 1.677 | 1.930 | 1.703 | 0.409 | 1.712 | 0.117 | 1.685 | 1.462 | 1.682 | 1.637 |
| 150.0 | 0.69 | 1.712 | 1.679 | 1.928 | 1.704 | 0.467 | 1.714 | 0.117 | 1.686 | 1.519 | 1.683 | 1.694 |
| 155.0 | 0.71 | 1.713 | 1.680 | 1.926 | 1.706 | 0.409 | 1.715 | 0.117 | 1.688 | 1.459 | 1.684 | 1.693 |
| 160.0 | 0.74 | 1.715 | 1.681 | 1.983 | 1.707 | 0.466 | 1.717 | 0.117 | 1.689 | 1.516 | 1.685 | 1.749 |
| 165.0 | 0.76 | 1.715 | 1.682 | 1.924 | 1.709 | 0.350 | 1.718 | 0.175 | 1.690 | 1.458 | 1.686 | 1.691 |
| 170.0 | 0.78 | 1.717 | 1.683 | 1.980 | 1.710 | 0.408 | 1.720 | 0.175 | 1.691 | 1.514 | 1.687 | 1.747 |
| 175.0 | 0.80 | 1.718 | 1.684 | 1.979 | 1.711 | 0.407 | 1.721 | 0.175 | 1.692 | 1.513 | 1.688 | 1.746 |
| 180.0 | 0.83 | 1.719 | 1.685 | 1.978 | 1.713 | 0.349 | 1.723 | 0.233 | 1.693 | 1.513 | 1.689 | 1.745 |
| 185.0 | 0.85 | 1.720 | 1.686 | 1.977 | 1.714 | 0.349 | 1.724 | 0.233 | 1.694 | 1.512 | 1.690 | 1.744 |
| 190.0 | 0.87 | 1.721 | 1.687 | 1.976 | 1.715 | 0.349 | 1.725 | 0.232 | 1.695 | 1.511 | 1.691 | 1.743 |
| 195.0 | 0.90 | 1.722 | 1.688 | 1.974 | 1.716 | 0.348 | 1.727 | 0.290 | 1.696 | 1.510 | 1.692 | 1.742 |
| 200.0 | 0.92 | 1.723 | 1.689 | 1.973 | 1.717 | 0.348 | 1.728 | 0.290 | 1.697 | 1.509 | 1.693 | 1.741 |

**Table 3a.** Key properties of the pair correlation function resulting from Langevin dynamics simulations and five integral theory approaches: the hypernetted-chain approximation (HNC), isomorph-based empirically modified hypernetted-chain approximation (IEMHNC), variational modified hypernetted-chain approximation (VMHNC), Rogers-Young approximation (RY) and Ballone-Pastore-Galli-Gazzillo approximation (BPGG). The absolute relative deviation $\epsilon_{\mathrm{r}}$ between the theoretical and the simulation results is also reported. **Results for $\arg_r\{g(r)=0.5\}$ in the case of $\kappa=2$**. The LD results are adopted from Table 6 of *T. Ott and M. Bonitz, Contrib. Plasma Phys.* **55**, *243 (2015)*. Here $x=r/d$, where $d$ is the Wigner-Seitz radius.

| $\Gamma$ | $\Gamma/\Gamma_{\mathrm{m}}$ | $x_{\mathrm{cv}}^{\mathrm{LD}}$ | $x_{\mathrm{cv}}^{\mathrm{HNC}}$ | $\epsilon_{\mathrm{HNC}}(\%)$ | $x_{\mathrm{cv}}^{\mathrm{IEMHNC}}$ | $\epsilon_{\mathrm{IEMHNC}}(\%)$ | $x_{\mathrm{cv}}^{\mathrm{VMHNC}}$ | $\epsilon_{\mathrm{VMHNC}}(\%)$ | $x_{\mathrm{cv}}^{\mathrm{RY}}$ | $\epsilon_{\mathrm{RY}}(\%)$ | $x_{\mathrm{cv}}^{\mathrm{BPGG}}$ | $\epsilon_{\mathrm{BPGG}}(\%)$ |
|---|---|---|---|---|---|---|---|---|---|---|---|---|
| 30.0 | 0.14 | 1.135 | 1.113 | 1.938 | 1.123 | 1.057 | 1.133 | 0.176 | 1.133 | 0.176 | 1.126 | 0.793 |
| 40.0 | 0.18 | 1.176 | 1.153 | 1.956 | 1.167 | 0.765 | 1.176 | 0.000 | 1.175 | 0.085 | 1.167 | 0.765 |
| 50.0 | 0.23 | 1.209 | 1.182 | 2.233 | 1.200 | 0.744 | 1.208 | 0.083 | 1.206 | 0.248 | 1.197 | 0.993 |
| 60.0 | 0.28 | 1.234 | 1.205 | 2.350 | 1.226 | 0.648 | 1.234 | 0.000 | 1.230 | 0.324 | 1.221 | 1.053 |
| 70.0 | 0.32 | 1.254 | 1.225 | 2.313 | 1.247 | 0.558 | 1.255 | 0.080 | 1.250 | 0.319 | 1.240 | 1.116 |
| 80.0 | 0.37 | 1.272 | 1.241 | 2.437 | 1.266 | 0.472 | 1.273 | 0.079 | 1.267 | 0.393 | 1.257 | 1.179 |
| 90.0 | 0.41 | 1.288 | 1.255 | 2.562 | 1.281 | 0.543 | 1.288 | 0.000 | 1.281 | 0.543 | 1.271 | 1.320 |
| 100.0 | 0.46 | 1.301 | 1.268 | 2.537 | 1.295 | 0.461 | 1.302 | 0.077 | 1.294 | 0.538 | 1.284 | 1.307 |
| 110.0 | 0.51 | 1.313 | 1.279 | 2.589 | 1.308 | 0.381 | 1.314 | 0.076 | 1.305 | 0.609 | 1.295 | 1.371 |
| 120.0 | 0.55 | 1.324 | 1.289 | 2.644 | 1.319 | 0.378 | 1.325 | 0.076 | 1.315 | 0.680 | 1.306 | 1.360 |
| 130.0 | 0.60 | 1.333 | 1.298 | 2.626 | 1.329 | 0.300 | 1.335 | 0.150 | 1.324 | 0.675 | 1.315 | 1.350 |
| 140.0 | 0.64 | 1.342 | 1.307 | 2.608 | 1.338 | 0.298 | 1.344 | 0.149 | 1.333 | 0.671 | 1.323 | 1.416 |
| 150.0 | 0.69 | 1.351 | 1.315 | 2.665 | 1.347 | 0.296 | 1.353 | 0.148 | 1.341 | 0.740 | 1.331 | 1.480 |
| 160.0 | 0.74 | 1.358 | 1.322 | 2.651 | 1.355 | 0.221 | 1.360 | 0.147 | 1.348 | 0.736 | 1.338 | 1.473 |
| 170.0 | 0.78 | 1.366 | 1.329 | 2.709 | 1.362 | 0.293 | 1.368 | 0.146 | 1.354 | 0.878 | 1.345 | 1.537 |
| 180.0 | 0.83 | 1.373 | 1.335 | 2.768 | 1.369 | 0.291 | 1.375 | 0.146 | 1.361 | 0.874 | 1.351 | 1.602 |
| 190.0 | 0.87 | 1.378 | 1.341 | 2.685 | 1.376 | 0.145 | 1.381 | 0.218 | 1.367 | 0.798 | 1.357 | 1.524 |
| 200.0 | 0.92 | 1.384 | 1.346 | 2.746 | 1.382 | 0.145 | 1.387 | 0.217 | 1.372 | 0.867 | 1.363 | 1.517 |
| 210.0 | 0.97 | 1.389 | 1.352 | 2.664 | 1.388 | 0.072 | 1.393 | 0.288 | 1.377 | 0.864 | 1.368 | 1.512 |
| 220.0 | 1.01 | 1.396 | 1.357 | 2.794 | 1.393 | 0.215 | 1.398 | 0.143 | 1.382 | 1.003 | 1.373 | 1.648 |
| 230.0 | 1.06 | 1.400 | 1.361 | 2.786 | 1.398 | 0.143 | 1.403 | 0.214 | 1.387 | 0.929 | 1.377 | 1.643 |
| 240.0 | 1.10 | 1.405 | 1.366 | 2.776 | 1.403 | 0.142 | 1.408 | 0.214 | 1.391 | 0.996 | 1.382 | 1.637 |
| 250.0 | 1.15 | 1.409 | 1.370 | 2.768 | 1.408 | 0.071 | 1.413 | 0.284 | 1.396 | 0.923 | 1.386 | 1.632 |
| 260.0 | 1.20 | 1.414 | 1.374 | 2.829 | 1.413 | 0.071 | 1.417 | 0.212 | 1.400 | 0.990 | 1.390 | 1.697 |
| 270.0 | 1.24 | 1.418 | 1.378 | 2.821 | 1.417 | 0.071 | 1.421 | 0.212 | 1.404 | 0.987 | 1.394 | 1.693 |
| 280.0 | 1.29 | 1.423 | 1.382 | 2.881 | 1.421 | 0.141 | 1.425 | 0.141 | 1.407 | 1.124 | 1.398 | 1.757 |
| 290.0 | 1.33 | 1.427 | 1.386 | 2.873 | 1.425 | 0.140 | 1.429 | 0.140 | 1.411 | 1.121 | 1.401 | 1.822 |
| 300.0 | 1.38 | 1.429 | 1.389 | 2.799 | 1.429 | 0.000 | 1.433 | 0.280 | 1.415 | 0.980 | 1.405 | 1.679 |
| 310.0 | 1.43 | 1.434 | 1.393 | 2.859 | 1.433 | 0.070 | 1.436 | 0.139 | 1.418 | 1.116 | 1.408 | 1.813 |
| 320.0 | 1.47 | 1.436 | 1.396 | 2.786 | 1.436 | 0.000 | 1.440 | 0.279 | 1.421 | 1.045 | 1.411 | 1.741 |
| 330.0 | 1.52 | 1.441 | 1.399 | 2.915 | 1.440 | 0.069 | 1.443 | 0.139 | 1.424 | 1.180 | 1.415 | 1.804 |
| 340.0 | 1.56 | 1.443 | 1.402 | 2.841 | 1.443 | 0.000 | 1.446 | 0.208 | 1.427 | 1.109 | 1.418 | 1.733 |
| 350.0 | 1.61 | 1.447 | 1.405 | 2.903 | 1.447 | 0.000 | 1.450 | 0.207 | 1.430 | 1.175 | 1.420 | 1.866 |
| 360.0 | 1.66 | 1.450 | 1.408 | 2.897 | 1.450 | 0.000 | 1.453 | 0.207 | 1.433 | 1.172 | 1.423 | 1.862 |
| 370.0 | 1.70 | 1.452 | 1.411 | 2.824 | 1.453 | 0.069 | 1.456 | 0.275 | 1.436 | 1.102 | 1.426 | 1.791 |
| 380.0 | 1.75 | 1.456 | 1.414 | 2.885 | 1.456 | 0.000 | 1.458 | 0.137 | 1.438 | 1.236 | 1.429 | 1.854 |
| 390.0 | 1.79 | 1.459 | 1.416 | 2.947 | 1.459 | 0.000 | 1.461 | 0.137 | 1.441 | 1.234 | 1.431 | 1.919 |
| 400.0 | 1.84 | 1.461 | 1.419 | 2.875 | 1.461 | 0.000 | 1.464 | 0.205 | 1.443 | 1.232 | 1.434 | 1.848 |

**Table 3b.** Key properties of the pair correlation function resulting from Langevin dynamics simulations and five integral theory approaches: the hypernetted-chain approximation (HNC), isomorph-based empirically modified hypernetted-chain approximation (IEMHNC), variational modified hypernetted-chain approximation (VMHNC), Rogers-Young approximation (RY) and Ballone-Pastore-Galli-Gazzillo approximation (BPGG). The absolute relative deviation $\epsilon_{\mathrm{r}}$ between the theoretical and the simulation results is also reported. **Results for the magnitude of the first maximum in the case of $\boldsymbol{\kappa = 2}$**. The LD results are adopted from Table 6 of *T. Ott and M. Bonitz, Contrib. Plasma Phys.* **55**, *243 (2015)*.

| $\Gamma$ | $\Gamma/\Gamma_{\mathrm{m}}$ | $g_{\mathrm{max1}}^{\mathrm{LD}}$ | $g_{\mathrm{max1}}^{\mathrm{HNC}}$ | $\epsilon_{\mathrm{HNC}}(\%)$ | $g_{\mathrm{max1}}^{\mathrm{IEMHNC}}$ | $\epsilon_{\mathrm{IEMHNC}}(\%)$ | $g_{\mathrm{max1}}^{\mathrm{VMHNC}}$ | $\epsilon_{\mathrm{VMHNC}}(\%)$ | $g_{\mathrm{max1}}^{\mathrm{RY}}$ | $\epsilon_{\mathrm{RY}}(\%)$ | $g_{\mathrm{max1}}^{\mathrm{BPGG}}$ | $\epsilon_{\mathrm{BPGG}}(\%)$ |
|---|---|---|---|---|---|---|---|---|---|---|---|---|
| 30.0 | 0.14 | 1.202 | 1.169 | 2.711 | 1.180 | 1.808 | 1.206 | 0.316 | 1.201 | 0.116 | 1.185 | 1.430 |
| 40.0 | 0.18 | 1.270 | 1.225 | 3.508 | 1.244 | 2.015 | 1.277 | 0.570 | 1.267 | 0.230 | 1.245 | 1.930 |
| 50.0 | 0.23 | 1.331 | 1.276 | 4.148 | 1.306 | 1.911 | 1.342 | 0.846 | 1.326 | 0.345 | 1.300 | 2.337 |
| 60.0 | 0.28 | 1.388 | 1.322 | 4.777 | 1.363 | 1.772 | 1.402 | 1.022 | 1.380 | 0.570 | 1.349 | 2.778 |
| 70.0 | 0.32 | 1.440 | 1.364 | 5.271 | 1.418 | 1.537 | 1.458 | 1.250 | 1.429 | 0.746 | 1.395 | 3.117 |
| 80.0 | 0.37 | 1.490 | 1.404 | 5.797 | 1.469 | 1.393 | 1.510 | 1.368 | 1.475 | 1.023 | 1.438 | 3.516 |
| 90.0 | 0.41 | 1.536 | 1.441 | 6.201 | 1.518 | 1.179 | 1.560 | 1.556 | 1.517 | 1.223 | 1.477 | 3.810 |
| 100.0 | 0.46 | 1.582 | 1.476 | 6.710 | 1.564 | 1.130 | 1.607 | 1.578 | 1.557 | 1.572 | 1.515 | 4.229 |
| 110.0 | 0.51 | 1.624 | 1.509 | 7.068 | 1.608 | 0.969 | 1.652 | 1.716 | 1.595 | 1.794 | 1.551 | 4.507 |
| 120.0 | 0.55 | 1.664 | 1.541 | 7.389 | 1.651 | 0.808 | 1.695 | 1.857 | 1.631 | 1.998 | 1.585 | 4.757 |
| 130.0 | 0.60 | 1.702 | 1.572 | 7.665 | 1.691 | 0.634 | 1.736 | 2.014 | 1.665 | 2.173 | 1.617 | 4.971 |
| 140.0 | 0.64 | 1.741 | 1.601 | 8.050 | 1.730 | 0.609 | 1.776 | 2.019 | 1.698 | 2.477 | 1.649 | 5.305 |
| 150.0 | 0.69 | 1.777 | 1.629 | 8.324 | 1.768 | 0.490 | 1.815 | 2.121 | 1.729 | 2.674 | 1.679 | 5.531 |
| 160.0 | 0.74 | 1.812 | 1.656 | 8.589 | 1.805 | 0.385 | 1.852 | 2.208 | 1.760 | 2.871 | 1.708 | 5.754 |
| 170.0 | 0.78 | 1.847 | 1.683 | 8.892 | 1.841 | 0.342 | 1.888 | 2.232 | 1.789 | 3.114 | 1.736 | 6.021 |
| 180.0 | 0.83 | 1.879 | 1.708 | 9.081 | 1.875 | 0.192 | 1.923 | 2.363 | 1.818 | 3.242 | 1.763 | 6.174 |
| 190.0 | 0.87 | 1.912 | 1.733 | 9.350 | 1.909 | 0.147 | 1.958 | 2.388 | 1.846 | 3.458 | 1.789 | 6.414 |
| 200.0 | 0.92 | 1.944 | 1.757 | 9.597 | 1.942 | 0.093 | 1.991 | 2.420 | 1.873 | 3.656 | 1.815 | 6.635 |
| 210.0 | 0.97 | 1.974 | 1.781 | 9.777 | 1.974 | 0.022 | 2.024 | 2.515 | 1.899 | 3.784 | 1.840 | 6.788 |
| 220.0 | 1.01 | 2.004 | 1.804 | 9.981 | 2.006 | 0.099 | 2.055 | 2.569 | 1.925 | 3.940 | 1.864 | 6.969 |
| 230.0 | 1.06 | 2.034 | 1.826 | 10.204 | 2.037 | 0.142 | 2.087 | 2.587 | 1.950 | 4.120 | 1.888 | 7.174 |
| 240.0 | 1.10 | 2.062 | 1.848 | 10.359 | 2.067 | 0.251 | 2.117 | 2.672 | 1.975 | 4.227 | 1.911 | 7.309 |
| 250.0 | 1.15 | 2.091 | 1.870 | 10.576 | 2.097 | 0.282 | 2.147 | 2.676 | 1.999 | 4.402 | 1.934 | 7.510 |
| 260.0 | 1.20 | 2.119 | 1.891 | 10.765 | 2.126 | 0.334 | 2.176 | 2.701 | 2.023 | 4.549 | 1.956 | 7.684 |
| 270.0 | 1.24 | 2.145 | 1.911 | 10.886 | 2.155 | 0.454 | 2.205 | 2.796 | 2.046 | 4.625 | 1.978 | 7.789 |
| 280.0 | 1.29 | 2.173 | 1.932 | 11.104 | 2.183 | 0.457 | 2.233 | 2.770 | 2.069 | 4.805 | 1.999 | 7.996 |
| 290.0 | 1.33 | 2.198 | 1.952 | 11.212 | 2.211 | 0.577 | 2.261 | 2.863 | 2.091 | 4.870 | 2.020 | 8.091 |
| 300.0 | 1.38 | 2.225 | 1.971 | 11.414 | 2.238 | 0.584 | 2.288 | 2.840 | 2.113 | 5.034 | 2.041 | 8.283 |
| 310.0 | 1.43 | 2.250 | 1.990 | 11.547 | 2.265 | 0.661 | 2.315 | 2.889 | 2.135 | 5.127 | 2.061 | 8.406 |
| 320.0 | 1.47 | 2.274 | 2.009 | 11.653 | 2.291 | 0.764 | 2.341 | 2.964 | 2.156 | 5.191 | 2.081 | 8.501 |
| 330.0 | 1.52 | 2.299 | 2.028 | 11.808 | 2.318 | 0.805 | 2.367 | 2.975 | 2.177 | 5.309 | 2.100 | 8.648 |
| 340.0 | 1.56 | 2.324 | 2.046 | 11.973 | 2.343 | 0.829 | 2.393 | 2.969 | 2.198 | 5.437 | 2.119 | 8.805 |
| 350.0 | 1.61 | 2.347 | 2.064 | 12.071 | 2.369 | 0.925 | 2.418 | 3.035 | 2.218 | 5.496 | 2.138 | 8.895 |
| 360.0 | 1.66 | 2.371 | 2.081 | 12.215 | 2.394 | 0.961 | 2.443 | 3.041 | 2.238 | 5.604 | 2.157 | 9.033 |
| 370.0 | 1.70 | 2.394 | 2.099 | 12.330 | 2.419 | 1.026 | 2.468 | 3.076 | 2.258 | 5.683 | 2.175 | 9.142 |
| 380.0 | 1.75 | 2.417 | 2.116 | 12.453 | 2.443 | 1.076 | 2.492 | 3.097 | 2.278 | 5.771 | 2.193 | 9.260 |
| 390.0 | 1.79 | 2.438 | 2.133 | 12.512 | 2.467 | 1.196 | 2.516 | 3.190 | 2.297 | 5.790 | 2.211 | 9.312 |
| 400.0 | 1.84 | 2.462 | 2.150 | 12.686 | 2.491 | 1.179 | 2.539 | 3.142 | 2.316 | 5.934 | 2.229 | 9.483 |

**Table 3c.** Key properties of the pair correlation function resulting from Langevin dynamics simulations and five integral theory approaches: the hypernetted-chain approximation (HNC), isomorph-based empirically modified hypernetted-chain approximation (IEMHNC), variational modified hypernetted-chain approximation (VMHNC), Rogers-Young approximation (RY) and Ballone-Pastore-Galli-Gazzillo approximation (BPGG). The absolute relative deviation $\epsilon_{\mathrm{r}}$ between the theoretical and the simulation results is also reported. **Results for the position of the first maximum in the case of $\boldsymbol{\kappa} = \mathbf{2}$**. The LD results are adopted from Table 6 of *T. Ott and M. Bonitz, Contrib. Plasma Phys.* **55**, *243 (2015)*. Here $x = r/d$, where $d$ is the Wigner-Seitz radius.

| $\Gamma$ | $\Gamma/\Gamma_{\mathrm{m}}$ | $x_{\mathrm{max1}}^{\mathrm{LD}}$ | $x_{\mathrm{max1}}^{\mathrm{HNC}}$ | $\epsilon_{\mathrm{HNC}}(\%)$ | $x_{\mathrm{max1}}^{\mathrm{IEMHNC}}$ | $\epsilon_{\mathrm{IEMHNC}}(\%)$ | $x_{\mathrm{max1}}^{\mathrm{VMHNC}}$ | $\epsilon_{\mathrm{VMHNC}}(\%)$ | $x_{\mathrm{max1}}^{\mathrm{RY}}$ | $\epsilon_{\mathrm{RY}}(\%)$ | $x_{\mathrm{max1}}^{\mathrm{BPGG}}$ | $\epsilon_{\mathrm{BPGG}}(\%)$ |
|---|---|---|---|---|---|---|---|---|---|---|---|---|
| 30.0 | 0.14 | 1.598 | 1.581 | 1.064 | 1.599 | 0.063 | 1.580 | 1.126 | 1.584 | 0.876 | 1.595 | 0.188 |
| 40.0 | 0.18 | 1.609 | 1.587 | 1.367 | 1.611 | 0.124 | 1.592 | 1.057 | 1.595 | 0.870 | 1.604 | 0.311 |
| 50.0 | 0.23 | 1.619 | 1.594 | 1.544 | 1.619 | 0.000 | 1.603 | 0.988 | 1.604 | 0.926 | 1.611 | 0.494 |
| 60.0 | 0.28 | 1.627 | 1.600 | 1.659 | 1.625 | 0.123 | 1.613 | 0.860 | 1.612 | 0.922 | 1.618 | 0.553 |
| 70.0 | 0.32 | 1.633 | 1.605 | 1.715 | 1.631 | 0.122 | 1.621 | 0.735 | 1.619 | 0.857 | 1.624 | 0.551 |
| 80.0 | 0.37 | 1.640 | 1.610 | 1.829 | 1.636 | 0.244 | 1.629 | 0.671 | 1.626 | 0.854 | 1.629 | 0.671 |
| 90.0 | 0.41 | 1.646 | 1.615 | 1.883 | 1.640 | 0.365 | 1.636 | 0.608 | 1.631 | 0.911 | 1.634 | 0.729 |
| 100.0 | 0.46 | 1.651 | 1.619 | 1.938 | 1.645 | 0.363 | 1.642 | 0.545 | 1.636 | 0.909 | 1.639 | 0.727 |
| 110.0 | 0.51 | 1.656 | 1.623 | 1.993 | 1.649 | 0.423 | 1.647 | 0.543 | 1.640 | 0.966 | 1.642 | 0.845 |
| 120.0 | 0.55 | 1.660 | 1.627 | 1.988 | 1.653 | 0.422 | 1.653 | 0.422 | 1.644 | 0.964 | 1.646 | 0.843 |
| 130.0 | 0.60 | 1.664 | 1.630 | 2.043 | 1.656 | 0.481 | 1.657 | 0.421 | 1.648 | 0.962 | 1.649 | 0.901 |
| 140.0 | 0.64 | 1.668 | 1.633 | 2.098 | 1.659 | 0.540 | 1.662 | 0.360 | 1.651 | 1.019 | 1.652 | 0.959 |
| 150.0 | 0.69 | 1.671 | 1.636 | 2.095 | 1.662 | 0.539 | 1.666 | 0.299 | 1.654 | 1.017 | 1.655 | 0.958 |
| 160.0 | 0.74 | 1.674 | 1.639 | 2.091 | 1.665 | 0.538 | 1.670 | 0.239 | 1.657 | 1.016 | 1.658 | 0.956 |
| 170.0 | 0.78 | 1.677 | 1.642 | 2.087 | 1.668 | 0.537 | 1.673 | 0.239 | 1.659 | 1.073 | 1.661 | 0.954 |
| 180.0 | 0.83 | 1.680 | 1.644 | 2.143 | 1.671 | 0.536 | 1.676 | 0.238 | 1.662 | 1.071 | 1.663 | 1.012 |
| 190.0 | 0.87 | 1.683 | 1.647 | 2.139 | 1.674 | 0.535 | 1.680 | 0.178 | 1.664 | 1.129 | 1.665 | 1.070 |
| 200.0 | 0.92 | 1.685 | 1.649 | 2.136 | 1.676 | 0.534 | 1.682 | 0.178 | 1.666 | 1.128 | 1.667 | 1.068 |
| 210.0 | 0.97 | 1.687 | 1.651 | 2.134 | 1.678 | 0.533 | 1.685 | 0.119 | 1.668 | 1.126 | 1.669 | 1.067 |
| 220.0 | 1.01 | 1.690 | 1.653 | 2.189 | 1.681 | 0.533 | 1.688 | 0.118 | 1.670 | 1.183 | 1.671 | 1.124 |
| 230.0 | 1.06 | 1.691 | 1.655 | 2.129 | 1.683 | 0.473 | 1.691 | 0.000 | 1.672 | 1.124 | 1.673 | 1.064 |
| 240.0 | 1.10 | 1.693 | 1.657 | 2.126 | 1.685 | 0.473 | 1.693 | 0.000 | 1.674 | 1.122 | 1.675 | 1.063 |
| 250.0 | 1.15 | 1.696 | 1.659 | 2.182 | 1.687 | 0.531 | 1.695 | 0.059 | 1.675 | 1.238 | 1.676 | 1.179 |
| 260.0 | 1.20 | 1.698 | 1.660 | 2.238 | 1.689 | 0.530 | 1.697 | 0.059 | 1.677 | 1.237 | 1.678 | 1.178 |
| 270.0 | 1.24 | 1.699 | 1.662 | 2.178 | 1.691 | 0.471 | 1.700 | 0.059 | 1.679 | 1.177 | 1.680 | 1.118 |
| 280.0 | 1.29 | 1.701 | 1.664 | 2.175 | 1.693 | 0.470 | 1.702 | 0.059 | 1.680 | 1.235 | 1.681 | 1.176 |
| 290.0 | 1.33 | 1.703 | 1.665 | 2.231 | 1.694 | 0.528 | 1.704 | 0.059 | 1.682 | 1.233 | 1.682 | 1.233 |
| 300.0 | 1.38 | 1.704 | 1.667 | 2.171 | 1.696 | 0.469 | 1.705 | 0.059 | 1.683 | 1.232 | 1.684 | 1.174 |
| 310.0 | 1.43 | 1.706 | 1.668 | 2.227 | 1.698 | 0.469 | 1.707 | 0.059 | 1.684 | 1.290 | 1.685 | 1.231 |
| 320.0 | 1.47 | 1.708 | 1.670 | 2.225 | 1.699 | 0.527 | 1.709 | 0.059 | 1.686 | 1.288 | 1.686 | 1.288 |
| 330.0 | 1.52 | 1.709 | 1.671 | 2.224 | 1.701 | 0.468 | 1.711 | 0.117 | 1.687 | 1.287 | 1.688 | 1.229 |
| 340.0 | 1.56 | 1.711 | 1.672 | 2.279 | 1.702 | 0.526 | 1.712 | 0.058 | 1.688 | 1.344 | 1.689 | 1.286 |
| 350.0 | 1.61 | 1.712 | 1.674 | 2.220 | 1.704 | 0.467 | 1.714 | 0.117 | 1.689 | 1.343 | 1.690 | 1.285 |
| 360.0 | 1.66 | 1.713 | 1.675 | 2.218 | 1.705 | 0.467 | 1.715 | 0.117 | 1.690 | 1.343 | 1.691 | 1.284 |
| 370.0 | 1.70 | 1.715 | 1.676 | 2.274 | 1.707 | 0.466 | 1.717 | 0.117 | 1.692 | 1.341 | 1.692 | 1.341 |
| 380.0 | 1.75 | 1.716 | 1.677 | 2.273 | 1.708 | 0.466 | 1.718 | 0.117 | 1.693 | 1.340 | 1.693 | 1.340 |
| 390.0 | 1.79 | 1.717 | 1.678 | 2.271 | 1.709 | 0.466 | 1.720 | 0.175 | 1.694 | 1.340 | 1.694 | 1.340 |
| 400.0 | 1.84 | 1.718 | 1.679 | 2.270 | 1.711 | 0.407 | 1.721 | 0.175 | 1.695 | 1.339 | 1.695 | 1.339 |

**Table 3d.** Key properties of the pair correlation function resulting from Langevin dynamics simulations and five integral theory approaches: the hypernetted-chain approximation (HNC), isomorph-based empirically modified hypernetted-chain approximation (IEMHNC), variational modified hypernetted-chain approximation (VMHNC), Rogers-Young approximation (RY) and Ballone-Pastore-Galli-Gazzillo approximation (BPGG). The absolute relative deviation $\epsilon_{\mathrm{r}}$ between the theoretical and the simulation results is also reported. **Results for the magnitude of the first minimum in the case of $\boldsymbol{\kappa = 2}$**. The LD results are adopted from Table 6 of *T. Ott and M. Bonitz, Contrib. Plasma Phys.* **55**, *243 (2015)*.

| $\Gamma$ | $\Gamma/\Gamma_{\mathrm{m}}$ | $g_{\mathrm{min1}}^{\mathrm{LD}}$ | $g_{\mathrm{min1}}^{\mathrm{HNC}}$ | $\epsilon_{\mathrm{HNC}}(\%)$ | $g_{\mathrm{min1}}^{\mathrm{IEMHNC}}$ | $\epsilon_{\mathrm{IEMHNC}}(\%)$ | $g_{\mathrm{min1}}^{\mathrm{VMHNC}}$ | $\epsilon_{\mathrm{VMHNC}}(\%)$ | $g_{\mathrm{min1}}^{\mathrm{RY}}$ | $\epsilon_{\mathrm{RY}}(\%)$ | $g_{\mathrm{min1}}^{\mathrm{BPGG}}$ | $\epsilon_{\mathrm{BPGG}}(\%)$ |
|---|---|---|---|---|---|---|---|---|---|---|---|---|
| 30.0 | 0.14 | 0.963 | 0.974 | 1.108 | 0.968 | 0.546 | 0.965 | 0.253 | 0.965 | 0.191 | 0.968 | 0.534 |
| 40.0 | 0.18 | 0.941 | 0.959 | 1.867 | 0.949 | 0.853 | 0.944 | 0.364 | 0.945 | 0.451 | 0.950 | 0.986 |
| 50.0 | 0.23 | 0.920 | 0.944 | 2.577 | 0.930 | 1.035 | 0.924 | 0.399 | 0.926 | 0.692 | 0.933 | 1.399 |
| 60.0 | 0.28 | 0.900 | 0.929 | 3.277 | 0.911 | 1.171 | 0.904 | 0.431 | 0.909 | 0.962 | 0.916 | 1.817 |
| 70.0 | 0.32 | 0.881 | 0.916 | 3.980 | 0.893 | 1.311 | 0.885 | 0.484 | 0.892 | 1.274 | 0.901 | 2.254 |
| 80.0 | 0.37 | 0.863 | 0.903 | 4.684 | 0.876 | 1.471 | 0.868 | 0.557 | 0.877 | 1.621 | 0.886 | 2.710 |
| 90.0 | 0.41 | 0.846 | 0.892 | 5.383 | 0.860 | 1.648 | 0.851 | 0.642 | 0.863 | 1.994 | 0.873 | 3.175 |
| 100.0 | 0.46 | 0.831 | 0.880 | 5.940 | 0.845 | 1.710 | 0.836 | 0.607 | 0.850 | 2.255 | 0.860 | 3.514 |
| 110.0 | 0.51 | 0.816 | 0.870 | 6.596 | 0.831 | 1.887 | 0.822 | 0.679 | 0.837 | 2.634 | 0.848 | 3.964 |
| 120.0 | 0.55 | 0.802 | 0.860 | 7.216 | 0.818 | 2.046 | 0.808 | 0.727 | 0.826 | 2.998 | 0.837 | 4.390 |
| 130.0 | 0.60 | 0.789 | 0.850 | 7.789 | 0.806 | 2.173 | 0.795 | 0.738 | 0.815 | 3.333 | 0.827 | 4.780 |
| 140.0 | 0.64 | 0.776 | 0.842 | 8.444 | 0.795 | 2.387 | 0.782 | 0.830 | 0.805 | 3.761 | 0.817 | 5.258 |
| 150.0 | 0.69 | 0.764 | 0.833 | 9.035 | 0.783 | 2.549 | 0.771 | 0.868 | 0.796 | 4.141 | 0.807 | 5.683 |
| 160.0 | 0.74 | 0.753 | 0.825 | 9.552 | 0.773 | 2.647 | 0.759 | 0.840 | 0.787 | 4.461 | 0.799 | 6.043 |
| 170.0 | 0.78 | 0.742 | 0.817 | 10.134 | 0.763 | 2.811 | 0.748 | 0.873 | 0.778 | 4.852 | 0.790 | 6.473 |
| 180.0 | 0.83 | 0.732 | 0.810 | 10.627 | 0.753 | 2.896 | 0.738 | 0.826 | 0.770 | 5.168 | 0.782 | 6.823 |
| 190.0 | 0.87 | 0.721 | 0.803 | 11.331 | 0.744 | 3.179 | 0.728 | 0.971 | 0.762 | 5.691 | 0.774 | 7.380 |
| 200.0 | 0.92 | 0.712 | 0.796 | 11.781 | 0.735 | 3.228 | 0.718 | 0.884 | 0.755 | 5.980 | 0.767 | 7.698 |
| 210.0 | 0.97 | 0.702 | 0.789 | 12.440 | 0.726 | 3.470 | 0.709 | 0.986 | 0.747 | 6.473 | 0.760 | 8.221 |
| 220.0 | 1.01 | 0.693 | 0.783 | 12.988 | 0.718 | 3.611 | 0.700 | 0.986 | 0.741 | 6.868 | 0.753 | 8.643 |
| 230.0 | 1.06 | 0.684 | 0.777 | 13.584 | 0.710 | 3.796 | 0.691 | 1.027 | 0.734 | 7.312 | 0.746 | 9.113 |
| 240.0 | 1.10 | 0.676 | 0.771 | 14.057 | 0.702 | 3.868 | 0.682 | 0.956 | 0.728 | 7.645 | 0.740 | 9.468 |
| 250.0 | 1.15 | 0.667 | 0.765 | 14.741 | 0.695 | 4.132 | 0.674 | 1.071 | 0.722 | 8.182 | 0.734 | 10.030 |
| 260.0 | 1.20 | 0.659 | 0.760 | 15.297 | 0.687 | 4.278 | 0.666 | 1.069 | 0.716 | 8.601 | 0.728 | 10.470 |
| 270.0 | 1.24 | 0.651 | 0.754 | 15.892 | 0.680 | 4.458 | 0.658 | 1.098 | 0.710 | 9.060 | 0.722 | 10.951 |
| 280.0 | 1.29 | 0.644 | 0.749 | 16.345 | 0.673 | 4.510 | 0.650 | 1.001 | 0.704 | 9.390 | 0.717 | 11.298 |
| 290.0 | 1.33 | 0.636 | 0.744 | 17.015 | 0.666 | 4.756 | 0.643 | 1.089 | 0.699 | 9.926 | 0.711 | 11.856 |
| 300.0 | 1.38 | 0.628 | 0.739 | 17.724 | 0.660 | 5.034 | 0.636 | 1.207 | 0.694 | 10.502 | 0.706 | 12.452 |
| 310.0 | 1.43 | 0.622 | 0.735 | 18.093 | 0.653 | 5.007 | 0.628 | 1.029 | 0.689 | 10.760 | 0.701 | 12.724 |
| 320.0 | 1.47 | 0.614 | 0.730 | 18.874 | 0.647 | 5.346 | 0.621 | 1.199 | 0.684 | 11.408 | 0.696 | 13.393 |
| 330.0 | 1.52 | 0.608 | 0.725 | 19.301 | 0.641 | 5.370 | 0.614 | 1.065 | 0.679 | 11.726 | 0.691 | 13.727 |
| 340.0 | 1.56 | 0.602 | 0.721 | 19.757 | 0.635 | 5.417 | 0.608 | 0.950 | 0.675 | 12.072 | 0.687 | 14.087 |
| 350.0 | 1.61 | 0.595 | 0.717 | 20.440 | 0.629 | 5.664 | 0.601 | 1.025 | 0.670 | 12.633 | 0.682 | 14.667 |
| 360.0 | 1.66 | 0.588 | 0.712 | 21.158 | 0.623 | 5.937 | 0.595 | 1.122 | 0.666 | 13.228 | 0.678 | 15.280 |
| 370.0 | 1.70 | 0.583 | 0.708 | 21.491 | 0.617 | 5.874 | 0.588 | 0.896 | 0.661 | 13.464 | 0.674 | 15.529 |
| 380.0 | 1.75 | 0.577 | 0.704 | 22.057 | 0.612 | 6.012 | 0.582 | 0.858 | 0.657 | 13.920 | 0.669 | 16.000 |
| 390.0 | 1.79 | 0.571 | 0.700 | 22.650 | 0.606 | 6.172 | 0.576 | 0.839 | 0.653 | 14.401 | 0.665 | 16.498 |
| 400.0 | 1.84 | 0.565 | 0.696 | 23.271 | 0.601 | 6.353 | 0.570 | 0.837 | 0.649 | 14.909 | 0.661 | 17.024 |

**Table 3e.** Key properties of the pair correlation function resulting from Langevin dynamics simulations and five integral theory approaches: the hypernetted-chain approximation (HNC), isomorph-based empirically modified hypernetted-chain approximation (IEMHNC), variational modified hypernetted-chain approximation (VMHNC), Rogers-Young approximation (RY) and Ballone-Pastore-Galli-Gazzillo approximation (BPGG). The absolute relative deviation $\epsilon_{\mathrm{r}}$ between the theoretical and the simulation results is also reported. **Results for the position of the first minimum in the case of $\boldsymbol{\kappa = 2}$.** The LD results are adopted from Table 6 of *T. Ott and M. Bonitz, Contrib. Plasma Phys.* **55**, *243 (2015)*. Here $x = r/d$, where $d$ is the Wigner-Seitz radius.

| $\Gamma$ | $\Gamma/\Gamma_{\mathrm{m}}$ | $x_{\mathrm{min1}}^{\mathrm{LD}}$ | $x_{\mathrm{min1}}^{\mathrm{HNC}}$ | $\epsilon_{\mathrm{HNC}}(\%)$ | $x_{\mathrm{min1}}^{\mathrm{IEMHNC}}$ | $\epsilon_{\mathrm{IEMHNC}}(\%)$ | $x_{\mathrm{min1}}^{\mathrm{VMHNC}}$ | $\epsilon_{\mathrm{VMHNC}}(\%)$ | $x_{\mathrm{min1}}^{\mathrm{RY}}$ | $\epsilon_{\mathrm{RY}}(\%)$ | $x_{\mathrm{min1}}^{\mathrm{BPGG}}$ | $\epsilon_{\mathrm{BPGG}}(\%)$ |
|---|---|---|---|---|---|---|---|---|---|---|---|---|
| 30.0 | 0.14 | 2.409 | 2.415 | 0.249 | 2.438 | 1.204 | 2.381 | 1.162 | 2.406 | 0.125 | 2.430 | 0.872 |
| 40.0 | 0.18 | 2.408 | 2.413 | 0.208 | 2.441 | 1.370 | 2.380 | 1.163 | 2.410 | 0.083 | 2.431 | 0.955 |
| 50.0 | 0.23 | 2.414 | 2.415 | 0.041 | 2.439 | 1.036 | 2.385 | 1.201 | 2.416 | 0.083 | 2.434 | 0.829 |
| 60.0 | 0.28 | 2.419 | 2.419 | 0.000 | 2.438 | 0.785 | 2.391 | 1.158 | 2.423 | 0.165 | 2.439 | 0.827 |
| 70.0 | 0.32 | 2.422 | 2.423 | 0.041 | 2.438 | 0.661 | 2.395 | 1.115 | 2.428 | 0.248 | 2.443 | 0.867 |
| 80.0 | 0.37 | 2.427 | 2.427 | 0.000 | 2.439 | 0.494 | 2.399 | 1.154 | 2.433 | 0.247 | 2.447 | 0.824 |
| 90.0 | 0.41 | 2.428 | 2.431 | 0.124 | 2.439 | 0.453 | 2.402 | 1.071 | 2.437 | 0.371 | 2.450 | 0.906 |
| 100.0 | 0.46 | 2.431 | 2.434 | 0.123 | 2.440 | 0.370 | 2.403 | 1.152 | 2.440 | 0.370 | 2.452 | 0.864 |
| 110.0 | 0.51 | 2.432 | 2.436 | 0.164 | 2.440 | 0.329 | 2.404 | 1.151 | 2.443 | 0.452 | 2.455 | 0.946 |
| 120.0 | 0.55 | 2.434 | 2.438 | 0.164 | 2.440 | 0.247 | 2.405 | 1.191 | 2.445 | 0.452 | 2.456 | 0.904 |
| 130.0 | 0.60 | 2.433 | 2.440 | 0.288 | 2.440 | 0.288 | 2.404 | 1.192 | 2.446 | 0.534 | 2.458 | 1.028 |
| 140.0 | 0.64 | 2.434 | 2.442 | 0.329 | 2.440 | 0.247 | 2.404 | 1.233 | 2.448 | 0.575 | 2.459 | 1.027 |
| 150.0 | 0.69 | 2.434 | 2.443 | 0.370 | 2.440 | 0.247 | 2.403 | 1.274 | 2.449 | 0.616 | 2.460 | 1.068 |
| 160.0 | 0.74 | 2.433 | 2.444 | 0.452 | 2.439 | 0.247 | 2.402 | 1.274 | 2.449 | 0.658 | 2.460 | 1.110 |
| 170.0 | 0.78 | 2.435 | 2.445 | 0.411 | 2.438 | 0.123 | 2.400 | 1.437 | 2.450 | 0.616 | 2.461 | 1.068 |
| 180.0 | 0.83 | 2.433 | 2.445 | 0.493 | 2.437 | 0.164 | 2.399 | 1.397 | 2.450 | 0.699 | 2.461 | 1.151 |
| 190.0 | 0.87 | 2.432 | 2.446 | 0.576 | 2.436 | 0.164 | 2.397 | 1.439 | 2.450 | 0.740 | 2.461 | 1.192 |
| 200.0 | 0.92 | 2.433 | 2.446 | 0.534 | 2.435 | 0.082 | 2.395 | 1.562 | 2.450 | 0.699 | 2.461 | 1.151 |
| 210.0 | 0.97 | 2.432 | 2.446 | 0.576 | 2.434 | 0.082 | 2.394 | 1.562 | 2.450 | 0.740 | 2.460 | 1.151 |
| 220.0 | 1.01 | 2.430 | 2.446 | 0.658 | 2.433 | 0.123 | 2.392 | 1.564 | 2.450 | 0.823 | 2.460 | 1.235 |
| 230.0 | 1.06 | 2.429 | 2.446 | 0.700 | 2.432 | 0.124 | 2.390 | 1.606 | 2.449 | 0.823 | 2.460 | 1.276 |
| 240.0 | 1.10 | 2.429 | 2.446 | 0.700 | 2.431 | 0.082 | 2.388 | 1.688 | 2.449 | 0.823 | 2.459 | 1.235 |
| 250.0 | 1.15 | 2.429 | 2.445 | 0.659 | 2.429 | 0.000 | 2.386 | 1.770 | 2.448 | 0.782 | 2.459 | 1.235 |
| 260.0 | 1.20 | 2.426 | 2.445 | 0.783 | 2.428 | 0.082 | 2.384 | 1.731 | 2.448 | 0.907 | 2.458 | 1.319 |
| 270.0 | 1.24 | 2.427 | 2.445 | 0.742 | 2.427 | 0.000 | 2.382 | 1.854 | 2.447 | 0.824 | 2.457 | 1.236 |
| 280.0 | 1.29 | 2.426 | 2.444 | 0.742 | 2.426 | 0.000 | 2.380 | 1.896 | 2.447 | 0.866 | 2.456 | 1.237 |
| 290.0 | 1.33 | 2.423 | 2.444 | 0.867 | 2.424 | 0.041 | 2.378 | 1.857 | 2.446 | 0.949 | 2.456 | 1.362 |
| 300.0 | 1.38 | 2.424 | 2.443 | 0.784 | 2.423 | 0.041 | 2.376 | 1.980 | 2.445 | 0.866 | 2.455 | 1.279 |
| 310.0 | 1.43 | 2.424 | 2.443 | 0.784 | 2.422 | 0.083 | 2.375 | 2.021 | 2.445 | 0.866 | 2.454 | 1.238 |
| 320.0 | 1.47 | 2.421 | 2.442 | 0.867 | 2.421 | 0.000 | 2.373 | 1.983 | 2.444 | 0.950 | 2.453 | 1.322 |
| 330.0 | 1.52 | 2.421 | 2.441 | 0.826 | 2.420 | 0.041 | 2.371 | 2.065 | 2.443 | 0.909 | 2.453 | 1.322 |
| 340.0 | 1.56 | 2.421 | 2.441 | 0.826 | 2.418 | 0.124 | 2.369 | 2.148 | 2.442 | 0.867 | 2.452 | 1.280 |
| 350.0 | 1.61 | 2.419 | 2.440 | 0.868 | 2.417 | 0.083 | 2.367 | 2.150 | 2.441 | 0.909 | 2.451 | 1.323 |
| 360.0 | 1.66 | 2.418 | 2.439 | 0.868 | 2.416 | 0.083 | 2.365 | 2.192 | 2.440 | 0.910 | 2.450 | 1.323 |
| 370.0 | 1.70 | 2.417 | 2.439 | 0.910 | 2.415 | 0.083 | 2.364 | 2.193 | 2.440 | 0.952 | 2.449 | 1.324 |
| 380.0 | 1.75 | 2.417 | 2.438 | 0.869 | 2.414 | 0.124 | 2.362 | 2.276 | 2.439 | 0.910 | 2.448 | 1.283 |
| 390.0 | 1.79 | 2.416 | 2.437 | 0.869 | 2.413 | 0.124 | 2.360 | 2.318 | 2.438 | 0.911 | 2.447 | 1.283 |
| 400.0 | 1.84 | 2.415 | 2.437 | 0.911 | 2.412 | 0.124 | 2.358 | 2.360 | 2.437 | 0.911 | 2.447 | 1.325 |

**Table 3f.** Key properties of the pair correlation function resulting from Langevin dynamics simulations and five integral theory approaches: the hypernetted-chain approximation (HNC), isomorph-based empirically modified hypernetted-chain approximation (IEMHNC), variational modified hypernetted-chain approximation (VMHNC), Rogers-Young approximation (RY) and Ballone-Pastore-Galli-Gazzillo approximation (BPGG). The absolute relative deviation $\epsilon_{\mathrm{r}}$ between the theoretical and the simulation results is also reported. **Results for the magnitude of the second maximum in the case of $\boldsymbol{\kappa = 2}$**. The LD results are adopted from Table 6 of *T. Ott and M. Bonitz, Contrib. Plasma Phys.* **55**, *243 (2015).*

| $\Gamma$ | $\Gamma/\Gamma_{\mathrm{m}}$ | $g_{\max 2}^{\mathrm{LD}}$ | $g_{\max 2}^{\mathrm{HNC}}$ | $\epsilon_{\mathrm{HNC}}(\%)$ | $g_{\max 2}^{\mathrm{IEMHNC}}$ | $\epsilon_{\mathrm{IEMHNC}}(\%)$ | $g_{\max 2}^{\mathrm{VMHNC}}$ | $\epsilon_{\mathrm{VMHNC}}(\%)$ | $g_{\max 2}^{\mathrm{RY}}$ | $\epsilon_{\mathrm{RY}}(\%)$ | $g_{\max 2}^{\mathrm{BPGG}}$ | $\epsilon_{\mathrm{BPGG}}(\%)$ |
|---|---|---|---|---|---|---|---|---|---|---|---|---|
| 30.0 | 0.14 | 1.008 | 1.005 | 0.304 | 1.007 | 0.126 | 1.007 | 0.056 | 1.008 | 0.045 | 1.007 | 0.136 |
| 40.0 | 0.18 | 1.016 | 1.009 | 0.642 | 1.013 | 0.270 | 1.015 | 0.132 | 1.014 | 0.164 | 1.013 | 0.338 |
| 50.0 | 0.23 | 1.025 | 1.015 | 0.994 | 1.021 | 0.381 | 1.023 | 0.172 | 1.022 | 0.278 | 1.019 | 0.542 |
| 60.0 | 0.28 | 1.034 | 1.021 | 1.292 | 1.030 | 0.399 | 1.033 | 0.130 | 1.031 | 0.335 | 1.027 | 0.689 |
| 70.0 | 0.32 | 1.044 | 1.027 | 1.650 | 1.039 | 0.456 | 1.043 | 0.136 | 1.039 | 0.458 | 1.035 | 0.898 |
| 80.0 | 0.37 | 1.054 | 1.033 | 1.983 | 1.049 | 0.480 | 1.053 | 0.116 | 1.048 | 0.566 | 1.043 | 1.088 |
| 90.0 | 0.41 | 1.064 | 1.040 | 2.300 | 1.059 | 0.487 | 1.063 | 0.085 | 1.057 | 0.671 | 1.051 | 1.267 |
| 100.0 | 0.46 | 1.074 | 1.046 | 2.606 | 1.069 | 0.486 | 1.073 | 0.052 | 1.066 | 0.778 | 1.059 | 1.442 |
| 110.0 | 0.51 | 1.084 | 1.053 | 2.904 | 1.079 | 0.483 | 1.084 | 0.026 | 1.074 | 0.891 | 1.066 | 1.618 |
| 120.0 | 0.55 | 1.093 | 1.059 | 3.110 | 1.089 | 0.391 | 1.094 | 0.082 | 1.083 | 0.922 | 1.074 | 1.706 |
| 130.0 | 0.60 | 1.103 | 1.065 | 3.403 | 1.099 | 0.396 | 1.104 | 0.084 | 1.091 | 1.054 | 1.082 | 1.890 |
| 140.0 | 0.64 | 1.113 | 1.072 | 3.694 | 1.108 | 0.407 | 1.114 | 0.070 | 1.100 | 1.197 | 1.090 | 2.079 |
| 150.0 | 0.69 | 1.122 | 1.078 | 3.899 | 1.118 | 0.338 | 1.123 | 0.130 | 1.108 | 1.262 | 1.097 | 2.187 |
| 160.0 | 0.74 | 1.131 | 1.085 | 4.106 | 1.128 | 0.278 | 1.133 | 0.169 | 1.116 | 1.338 | 1.105 | 2.303 |
| 170.0 | 0.78 | 1.140 | 1.091 | 4.315 | 1.137 | 0.229 | 1.142 | 0.190 | 1.124 | 1.427 | 1.112 | 2.428 |
| 180.0 | 0.83 | 1.149 | 1.097 | 4.527 | 1.147 | 0.191 | 1.151 | 0.192 | 1.131 | 1.526 | 1.120 | 2.561 |
| 190.0 | 0.87 | 1.158 | 1.103 | 4.742 | 1.156 | 0.164 | 1.160 | 0.176 | 1.139 | 1.636 | 1.127 | 2.702 |
| 200.0 | 0.92 | 1.165 | 1.109 | 4.797 | 1.165 | 0.024 | 1.169 | 0.312 | 1.147 | 1.588 | 1.134 | 2.684 |
| 210.0 | 0.97 | 1.173 | 1.115 | 4.938 | 1.174 | 0.113 | 1.177 | 0.344 | 1.154 | 1.635 | 1.141 | 2.760 |
| 220.0 | 1.01 | 1.181 | 1.121 | 5.084 | 1.183 | 0.191 | 1.185 | 0.357 | 1.161 | 1.694 | 1.147 | 2.844 |
| 230.0 | 1.06 | 1.189 | 1.127 | 5.234 | 1.192 | 0.256 | 1.193 | 0.351 | 1.168 | 1.762 | 1.154 | 2.936 |
| 240.0 | 1.10 | 1.196 | 1.133 | 5.309 | 1.201 | 0.394 | 1.201 | 0.414 | 1.175 | 1.758 | 1.161 | 2.955 |
| 250.0 | 1.15 | 1.204 | 1.138 | 5.468 | 1.209 | 0.436 | 1.209 | 0.374 | 1.182 | 1.845 | 1.167 | 3.064 |
| 260.0 | 1.20 | 1.210 | 1.144 | 5.475 | 1.218 | 0.633 | 1.216 | 0.485 | 1.188 | 1.779 | 1.173 | 3.020 |
| 270.0 | 1.24 | 1.217 | 1.149 | 5.565 | 1.226 | 0.734 | 1.223 | 0.496 | 1.195 | 1.804 | 1.180 | 3.065 |
| 280.0 | 1.29 | 1.224 | 1.155 | 5.661 | 1.234 | 0.825 | 1.230 | 0.492 | 1.202 | 1.838 | 1.186 | 3.118 |
| 290.0 | 1.33 | 1.230 | 1.160 | 5.684 | 1.242 | 0.985 | 1.237 | 0.554 | 1.208 | 1.801 | 1.192 | 3.100 |
| 300.0 | 1.38 | 1.236 | 1.165 | 5.713 | 1.250 | 1.134 | 1.243 | 0.601 | 1.214 | 1.773 | 1.198 | 3.090 |
| 310.0 | 1.43 | 1.243 | 1.171 | 5.823 | 1.258 | 1.189 | 1.250 | 0.553 | 1.220 | 1.832 | 1.204 | 3.166 |
| 320.0 | 1.47 | 1.248 | 1.176 | 5.786 | 1.265 | 1.396 | 1.256 | 0.653 | 1.226 | 1.741 | 1.209 | 3.093 |
| 330.0 | 1.52 | 1.254 | 1.181 | 5.830 | 1.273 | 1.511 | 1.262 | 0.658 | 1.232 | 1.738 | 1.215 | 3.105 |
| 340.0 | 1.56 | 1.259 | 1.186 | 5.805 | 1.280 | 1.695 | 1.268 | 0.731 | 1.238 | 1.664 | 1.221 | 3.048 |
| 350.0 | 1.61 | 1.264 | 1.191 | 5.784 | 1.288 | 1.868 | 1.274 | 0.790 | 1.244 | 1.597 | 1.226 | 2.998 |
| 360.0 | 1.66 | 1.270 | 1.196 | 5.844 | 1.295 | 1.950 | 1.280 | 0.758 | 1.249 | 1.617 | 1.231 | 3.032 |
| 370.0 | 1.70 | 1.275 | 1.201 | 5.833 | 1.302 | 2.102 | 1.285 | 0.794 | 1.255 | 1.566 | 1.237 | 2.996 |
| 380.0 | 1.75 | 1.279 | 1.205 | 5.754 | 1.309 | 2.323 | 1.290 | 0.896 | 1.261 | 1.446 | 1.242 | 2.891 |
| 390.0 | 1.79 | 1.283 | 1.210 | 5.680 | 1.315 | 2.533 | 1.296 | 0.987 | 1.266 | 1.333 | 1.247 | 2.793 |
| 400.0 | 1.84 | 1.288 | 1.215 | 5.685 | 1.322 | 2.653 | 1.301 | 0.989 | 1.271 | 1.303 | 1.252 | 2.777 |

**Table 3g.** Key properties of the pair correlation function resulting from Langevin dynamics simulations and five integral theory approaches: the hypernetted-chain approximation (HNC), isomorph-based empirically modified hypernetted-chain approximation (IEMHNC), variational modified hypernetted-chain approximation (VMHNC), Rogers-Young approximation (RY) and Ballone-Pastore-Galli-Gazzillo approximation (BPGG). The absolute relative deviation $\epsilon_{\mathrm{r}}$ between the theoretical and the simulation results is also reported. **Results for the position of the second maximum in the case of $\boldsymbol{\kappa = 2}$**. The LD results are adopted from Table 6 of *T. Ott and M. Bonitz, Contrib. Plasma Phys.* **55**, *243 (2015)*. Here $x = r/d$, where $d$ is the Wigner-Seitz radius.

| $\Gamma$ | $\Gamma/\Gamma_{\mathrm{m}}$ | $x_{\mathrm{max2}}^{\mathrm{LD}}$ | $x_{\mathrm{max2}}^{\mathrm{HNC}}$ | $\epsilon_{\mathrm{HNC}}(\%)$ | $x_{\mathrm{max2}}^{\mathrm{IEMHNC}}$ | $\epsilon_{\mathrm{IEMHNC}}(\%)$ | $x_{\mathrm{max2}}^{\mathrm{VMHNC}}$ | $\epsilon_{\mathrm{VMHNC}}(\%)$ | $x_{\mathrm{max2}}^{\mathrm{RY}}$ | $\epsilon_{\mathrm{RY}}(\%)$ | $x_{\mathrm{max2}}^{\mathrm{BPGG}}$ | $\epsilon_{\mathrm{BPGG}}(\%)$ |
|---|---|---|---|---|---|---|---|---|---|---|---|---|
| 30.0 | 0.14 | 3.213 | 3.230 | 0.529 | 3.255 | 1.307 | 3.180 | 1.027 | 3.208 | 0.156 | 3.246 | 1.027 |
| 40.0 | 0.18 | 3.199 | 3.212 | 0.406 | 3.245 | 1.438 | 3.170 | 0.907 | 3.198 | 0.031 | 3.231 | 1.000 |
| 50.0 | 0.23 | 3.193 | 3.204 | 0.345 | 3.231 | 1.190 | 3.169 | 0.752 | 3.196 | 0.094 | 3.225 | 1.002 |
| 60.0 | 0.28 | 3.192 | 3.200 | 0.251 | 3.220 | 0.877 | 3.172 | 0.627 | 3.196 | 0.125 | 3.223 | 0.971 |
| 70.0 | 0.32 | 3.196 | 3.199 | 0.094 | 3.214 | 0.563 | 3.175 | 0.657 | 3.198 | 0.063 | 3.222 | 0.814 |
| 80.0 | 0.37 | 3.193 | 3.198 | 0.157 | 3.210 | 0.532 | 3.180 | 0.407 | 3.200 | 0.219 | 3.221 | 0.877 |
| 90.0 | 0.41 | 3.194 | 3.198 | 0.125 | 3.208 | 0.438 | 3.184 | 0.313 | 3.202 | 0.250 | 3.222 | 0.877 |
| 100.0 | 0.46 | 3.194 | 3.198 | 0.125 | 3.207 | 0.407 | 3.188 | 0.188 | 3.204 | 0.313 | 3.222 | 0.877 |
| 110.0 | 0.51 | 3.198 | 3.199 | 0.031 | 3.206 | 0.250 | 3.193 | 0.156 | 3.206 | 0.250 | 3.223 | 0.782 |
| 120.0 | 0.55 | 3.198 | 3.200 | 0.063 | 3.206 | 0.250 | 3.197 | 0.031 | 3.208 | 0.313 | 3.223 | 0.782 |
| 130.0 | 0.60 | 3.200 | 3.201 | 0.031 | 3.207 | 0.219 | 3.201 | 0.031 | 3.209 | 0.281 | 3.224 | 0.750 |
| 140.0 | 0.64 | 3.201 | 3.201 | 0.000 | 3.208 | 0.219 | 3.205 | 0.125 | 3.211 | 0.312 | 3.225 | 0.750 |
| 150.0 | 0.69 | 3.201 | 3.202 | 0.031 | 3.209 | 0.250 | 3.208 | 0.219 | 3.213 | 0.375 | 3.226 | 0.781 |
| 160.0 | 0.74 | 3.205 | 3.203 | 0.062 | 3.210 | 0.156 | 3.212 | 0.218 | 3.214 | 0.281 | 3.226 | 0.655 |
| 170.0 | 0.78 | 3.203 | 3.204 | 0.031 | 3.211 | 0.250 | 3.216 | 0.406 | 3.216 | 0.406 | 3.227 | 0.749 |
| 180.0 | 0.83 | 3.207 | 3.205 | 0.062 | 3.213 | 0.187 | 3.219 | 0.374 | 3.217 | 0.312 | 3.228 | 0.655 |
| 190.0 | 0.87 | 3.206 | 3.206 | 0.000 | 3.214 | 0.250 | 3.222 | 0.499 | 3.219 | 0.405 | 3.229 | 0.717 |
| 200.0 | 0.92 | 3.207 | 3.207 | 0.000 | 3.215 | 0.249 | 3.226 | 0.592 | 3.220 | 0.405 | 3.230 | 0.717 |
| 210.0 | 0.97 | 3.209 | 3.209 | 0.000 | 3.217 | 0.249 | 3.229 | 0.623 | 3.221 | 0.374 | 3.231 | 0.686 |
| 220.0 | 1.01 | 3.210 | 3.210 | 0.000 | 3.218 | 0.249 | 3.232 | 0.685 | 3.223 | 0.405 | 3.232 | 0.685 |
| 230.0 | 1.06 | 3.211 | 3.211 | 0.000 | 3.220 | 0.280 | 3.235 | 0.747 | 3.224 | 0.405 | 3.232 | 0.654 |
| 240.0 | 1.10 | 3.211 | 3.212 | 0.031 | 3.221 | 0.311 | 3.237 | 0.810 | 3.225 | 0.436 | 3.233 | 0.685 |
| 250.0 | 1.15 | 3.212 | 3.213 | 0.031 | 3.223 | 0.342 | 3.240 | 0.872 | 3.226 | 0.436 | 3.234 | 0.685 |
| 260.0 | 1.20 | 3.212 | 3.214 | 0.062 | 3.224 | 0.374 | 3.243 | 0.965 | 3.227 | 0.467 | 3.235 | 0.716 |
| 270.0 | 1.24 | 3.213 | 3.215 | 0.062 | 3.226 | 0.405 | 3.245 | 0.996 | 3.228 | 0.467 | 3.236 | 0.716 |
| 280.0 | 1.29 | 3.214 | 3.216 | 0.062 | 3.227 | 0.404 | 3.248 | 1.058 | 3.229 | 0.467 | 3.237 | 0.716 |
| 290.0 | 1.33 | 3.214 | 3.217 | 0.093 | 3.228 | 0.436 | 3.250 | 1.120 | 3.231 | 0.529 | 3.237 | 0.716 |
| 300.0 | 1.38 | 3.216 | 3.218 | 0.062 | 3.230 | 0.435 | 3.253 | 1.150 | 3.232 | 0.498 | 3.238 | 0.684 |
| 310.0 | 1.43 | 3.216 | 3.218 | 0.062 | 3.231 | 0.466 | 3.255 | 1.213 | 3.233 | 0.529 | 3.239 | 0.715 |
| 320.0 | 1.47 | 3.216 | 3.219 | 0.093 | 3.233 | 0.529 | 3.257 | 1.275 | 3.234 | 0.560 | 3.240 | 0.746 |
| 330.0 | 1.52 | 3.218 | 3.220 | 0.062 | 3.234 | 0.497 | 3.260 | 1.305 | 3.235 | 0.528 | 3.240 | 0.684 |
| 340.0 | 1.56 | 3.218 | 3.221 | 0.093 | 3.235 | 0.528 | 3.262 | 1.367 | 3.236 | 0.559 | 3.241 | 0.715 |
| 350.0 | 1.61 | 3.218 | 3.222 | 0.124 | 3.237 | 0.590 | 3.264 | 1.429 | 3.236 | 0.559 | 3.242 | 0.746 |
| 360.0 | 1.66 | 3.220 | 3.223 | 0.093 | 3.238 | 0.559 | 3.266 | 1.429 | 3.237 | 0.528 | 3.243 | 0.714 |
| 370.0 | 1.70 | 3.219 | 3.224 | 0.155 | 3.239 | 0.621 | 3.268 | 1.522 | 3.238 | 0.590 | 3.243 | 0.746 |
| 380.0 | 1.75 | 3.221 | 3.225 | 0.124 | 3.240 | 0.590 | 3.270 | 1.521 | 3.239 | 0.559 | 3.244 | 0.714 |
| 390.0 | 1.79 | 3.221 | 3.226 | 0.155 | 3.242 | 0.652 | 3.272 | 1.583 | 3.240 | 0.590 | 3.245 | 0.745 |
| 400.0 | 1.84 | 3.221 | 3.227 | 0.186 | 3.243 | 0.683 | 3.274 | 1.645 | 3.241 | 0.621 | 3.246 | 0.776 |

**Table 4a.** The reduced excess internal energy due to particle-particle interactions $u_{\mathrm{ex}}^{\mathrm{pp}}$ resulting from molecular dynamics simulations and five integral theory approaches: the hypernetted-chain approximation (HNC), isomorph-based empirically modified hypernetted-chain approximation (IEMHNC), variational modified hypernetted-chain approximation (VMHNC), Rogers-Young approximation (RY) and Ballone-Pastore-Galli-Gazzillo approximation (BPGG). The absolute relative deviation $\epsilon_{\mathrm{r}}$ between the theoretical and the simulation results is also reported. **Results for very low screening parameters**, *i.e.* $\kappa = \{0.0, 0.2, 0.4, 0.6\}$. The MD results are adopted from Table II of *R. T. Farouki and S. Hamaguchi, J. Chem. Phys.* **101**, *9885 (1994)*. Owing to the well-known divergence, the reduced excess internal energy for the OCP includes interaction with the neutralizing background.

| $\Gamma$ | $\Gamma/\Gamma_{\mathrm{m}}$ | $u_{\mathrm{ex}}^{\mathrm{pp,MD}}$ | $u_{\mathrm{ex}}^{\mathrm{pp,HNC}}$ | $\epsilon_{\mathrm{r}}^{\mathrm{HNC}}(\%)$ | $u_{\mathrm{ex}}^{\mathrm{pp,IEMHNC}}$ | $\epsilon_{\mathrm{r}}^{\mathrm{IEMHNC}}(\%)$ | $u_{\mathrm{ex}}^{\mathrm{pp,VMHNC}}$ | $\epsilon_{\mathrm{r}}^{\mathrm{VMHNC}}(\%)$ | $u_{\mathrm{ex}}^{\mathrm{pp,RY}}$ | $\epsilon_{\mathrm{r}}^{\mathrm{RY}}(\%)$ | $u_{\mathrm{ex}}^{\mathrm{pp,BPGG}}$ | $\epsilon_{\mathrm{r}}^{\mathrm{BPGG}}(\%)$ |
|---|---|---|---|---|---|---|---|---|---|---|---|---|
| | | | | | | $\kappa = 0.0$ | | | | | | |
| 10.0 | 0.06 | -7.995 | -7.935 | 0.745 | -7.963 | 0.395 | -7.989 | 0.080 | -7.993 | 0.027 | -7.939 | 0.706 |
| 20.0 | 0.12 | -16.668 | -16.538 | 0.782 | -16.639 | 0.177 | -16.662 | 0.036 | -16.640 | 0.167 | -16.554 | 0.685 |
| 40.0 | 0.23 | -34.259 | -33.999 | 0.758 | -34.221 | 0.110 | -34.251 | 0.023 | -34.168 | 0.267 | -34.083 | 0.513 |
| 60.0 | 0.35 | -51.957 | -51.597 | 0.692 | -51.925 | 0.061 | -51.960 | 0.006 | -51.817 | 0.269 | -51.815 | 0.274 |
| 80.0 | 0.47 | -69.725 | -69.264 | 0.661 | -69.690 | 0.051 | -69.724 | 0.001 | -69.528 | 0.283 | -69.689 | 0.051 |
| 100.0 | 0.58 | -87.519 | -86.974 | 0.623 | -87.486 | 0.038 | -87.515 | 0.004 | -87.276 | 0.277 | -87.688 | 0.193 |
| 120.0 | 0.70 | -105.343 | -104.715 | 0.596 | -105.284 | 0.056 | -105.310 | 0.032 | -105.049 | 0.279 | -105.802 | 0.436 |
| 140.0 | 0.81 | -123.175 | -122.478 | 0.566 | -123.046 | 0.105 | -123.087 | 0.072 | -122.834 | 0.277 | -124.028 | 0.693 |
| 160.0 | 0.93 | -141.698 | -140.256 | 1.017 | -140.727 | 0.685 | -140.831 | 0.612 | -140.616 | 0.764 | -142.362 | 0.469 |
| | | | | | | $\kappa = 0.2$ | | | | | | |
| 10.0 | 0.06 | 367.955 | 368.018 | 0.017 | 367.990 | 0.010 | 367.965 | 0.003 | 367.962 | 0.002 | 368.015 | 0.016 |
| 20.0 | 0.12 | 735.243 | 735.373 | 0.018 | 735.272 | 0.004 | 735.250 | 0.001 | 735.272 | 0.004 | 735.368 | 0.017 |
| 40.0 | 0.23 | 1469.574 | 1469.827 | 0.017 | 1469.605 | 0.002 | 1469.578 | 0.000 | 1469.660 | 0.006 | 1469.820 | 0.017 |
| 60.0 | 0.35 | 2203.783 | 2204.145 | 0.016 | 2203.818 | 0.002 | 2203.786 | 0.000 | 2203.927 | 0.007 | 2204.138 | 0.016 |
| 80.0 | 0.46 | 2937.938 | 2938.395 | 0.016 | 2937.970 | 0.001 | 2937.937 | 0.000 | 2938.133 | 0.007 | 2938.387 | 0.015 |
| 100.0 | 0.58 | 3672.056 | 3672.602 | 0.015 | 3672.084 | 0.001 | 3672.055 | 0.000 | 3672.302 | 0.007 | 3672.594 | 0.015 |
| 120.0 | 0.69 | 4406.160 | 4406.779 | 0.014 | 4406.171 | 0.000 | 4406.149 | 0.000 | 4406.444 | 0.006 | 4406.771 | 0.014 |
| 140.0 | 0.81 | 5140.234 | 5140.934 | 0.014 | 5140.238 | 0.000 | 5140.226 | 0.000 | 5140.567 | 0.006 | 5140.925 | 0.013 |
| 160.0 | 0.92 | 5873.712 | 5875.071 | 0.023 | 5874.292 | 0.010 | 5874.291 | 0.010 | 5874.674 | 0.016 | 5875.062 | 0.023 |
| | | | | | | $\kappa = 0.4$ | | | | | | |
| 10.0 | 0.06 | 87.571 | 87.628 | 0.065 | 87.602 | 0.035 | 87.578 | 0.008 | 87.574 | 0.003 | 87.620 | 0.056 |
| 20.0 | 0.11 | 174.480 | 174.606 | 0.072 | 174.508 | 0.016 | 174.487 | 0.004 | 174.507 | 0.015 | 174.593 | 0.065 |
| 40.0 | 0.22 | 348.064 | 348.308 | 0.070 | 348.091 | 0.008 | 348.066 | 0.001 | 348.144 | 0.023 | 348.290 | 0.065 |
| 60.0 | 0.34 | 521.526 | 521.876 | 0.067 | 521.555 | 0.005 | 521.526 | 0.000 | 521.661 | 0.026 | 521.855 | 0.063 |
| 80.0 | 0.45 | 694.927 | 695.377 | 0.065 | 694.959 | 0.005 | 694.930 | 0.000 | 695.118 | 0.027 | 695.353 | 0.061 |
| 100.0 | 0.56 | 868.304 | 868.835 | 0.061 | 868.325 | 0.002 | 868.300 | 0.000 | 868.538 | 0.027 | 868.810 | 0.058 |
| 120.0 | 0.67 | 1041.667 | 1042.264 | 0.057 | 1041.665 | 0.000 | 1041.647 | 0.002 | 1041.932 | 0.025 | 1042.238 | 0.055 |
| 140.0 | 0.78 | 1214.982 | 1215.670 | 0.057 | 1214.985 | 0.000 | 1214.976 | 0.000 | 1215.306 | 0.027 | 1215.644 | 0.054 |
| 160.0 | 0.90 | 1387.654 | 1389.059 | 0.101 | 1388.289 | 0.046 | 1388.292 | 0.046 | 1388.665 | 0.073 | 1389.032 | 0.099 |
| | | | | | | $\kappa = 0.6$ | | | | | | |
| 10.0 | 0.05 | 36.262 | 36.314 | 0.143 | 36.292 | 0.082 | 36.268 | 0.016 | 36.262 | 0.001 | 36.302 | 0.111 |
| 20.0 | 0.11 | 71.877 | 71.998 | 0.168 | 71.906 | 0.040 | 71.887 | 0.014 | 71.902 | 0.035 | 71.977 | 0.139 |
| 40.0 | 0.21 | 142.878 | 143.118 | 0.168 | 142.910 | 0.022 | 142.889 | 0.007 | 142.958 | 0.056 | 143.086 | 0.146 |
| 60.0 | 0.32 | 213.769 | 214.107 | 0.158 | 213.798 | 0.013 | 213.773 | 0.002 | 213.896 | 0.059 | 214.068 | 0.140 |
| 80.0 | 0.43 | 284.608 | 285.029 | 0.148 | 284.627 | 0.007 | 284.601 | 0.002 | 284.775 | 0.059 | 284.985 | 0.133 |
| 100.0 | 0.53 | 355.406 | 355.910 | 0.142 | 355.420 | 0.004 | 355.396 | 0.003 | 355.617 | 0.059 | 355.863 | 0.128 |
| 120.0 | 0.64 | 426.172 | 426.761 | 0.138 | 426.186 | 0.003 | 426.168 | 0.001 | 426.434 | 0.062 | 426.712 | 0.127 |
| 140.0 | 0.75 | 496.928 | 497.591 | 0.133 | 496.932 | 0.001 | 496.923 | 0.001 | 497.232 | 0.061 | 497.539 | 0.123 |
| 160.0 | 0.86 | 567.668 | 568.404 | 0.130 | 567.663 | 0.001 | 567.665 | 0.001 | 568.015 | 0.061 | 568.350 | 0.120 |
| 180.0 | 0.96 | 637.721 | 639.202 | 0.232 | 638.382 | 0.104 | 638.396 | 0.106 | 638.787 | 0.167 | 639.147 | 0.224 |

**Table 4b.** The reduced excess internal energy due to particle-particle interactions $u_{\mathrm{ex}}^{\mathrm{pp}}$ resulting from molecular dynamics simulations and five integral theory approaches: the hypernetted-chain approximation (HNC), isomorph-based empirically modified hypernetted-chain approximation (IEMHNC), variational modified hypernetted-chain approximation (VMHNC), Rogers-Young approximation (RY) and Ballone-Pastore-Galli-Gazzillo approximation (BPGG). The absolute relative deviation $\epsilon_{\mathrm{r}}$ between the theoretical and the simulation results is also reported. **Results for low screening parameters**, *i.e.* $\kappa = \{0.8, 1.0, 1.2\}$. The MD results are adopted from Table II of *R. T. Farouki and S. Hamaguchi, J. Chem. Phys.* **101**, *9885 (1994)* and from Table II of *S. Hamaguchi, R. T. Farouki and D. H. E. Dubin, J. Chem. Phys.* **105**, *7641 (1996)*.

| $\Gamma$ | $\Gamma/\Gamma_{\mathrm{m}}$ | $u_{\mathrm{ex}}^{\mathrm{pp,MD}}$ | $u_{\mathrm{ex}}^{\mathrm{pp,HNC}}$ | $\epsilon_{\mathrm{r}}^{\mathrm{HNC}}(\%)$ | $u_{\mathrm{ex}}^{\mathrm{pp,IEMHNC}}$ | $\epsilon_{\mathrm{r}}^{\mathrm{IEMHNC}}(\%)$ | $u_{\mathrm{ex}}^{\mathrm{pp,VMHNC}}$ | $\epsilon_{\mathrm{r}}^{\mathrm{VMHNC}}(\%)$ | $u_{\mathrm{ex}}^{\mathrm{pp,RY}}$ | $\epsilon_{\mathrm{r}}^{\mathrm{RY}}(\%)$ | $u_{\mathrm{ex}}^{\mathrm{pp,BPGG}}$ | $\epsilon_{\mathrm{r}}^{\mathrm{BPGG}}(\%)$ |
|---|---|---|---|---|---|---|---|---|---|---|---|---|
| $\kappa = 0.8$ | | | | | | | | | | | | |
| 10.0 | 0.05 | 18.718 | 18.767 | 0.261 | 18.751 | 0.174 | 18.726 | 0.041 | 18.719 | 0.007 | 18.752 | 0.180 |
| 20.0 | 0.10 | 36.821 | 36.932 | 0.301 | 36.848 | 0.073 | 36.830 | 0.025 | 36.840 | 0.052 | 36.903 | 0.223 |
| 40.0 | 0.20 | 72.801 | 73.020 | 0.301 | 72.826 | 0.034 | 72.806 | 0.007 | 72.864 | 0.087 | 72.973 | 0.237 |
| 60.0 | 0.30 | 108.666 | 108.979 | 0.288 | 108.690 | 0.022 | 108.667 | 0.001 | 108.774 | 0.099 | 108.922 | 0.235 |
| 80.0 | 0.40 | 144.482 | 144.875 | 0.272 | 144.497 | 0.011 | 144.472 | 0.007 | 144.627 | 0.100 | 144.809 | 0.226 |
| 100.0 | 0.50 | 180.249 | 180.730 | 0.267 | 180.269 | 0.011 | 180.245 | 0.002 | 180.444 | 0.108 | 180.657 | 0.226 |
| 120.0 | 0.60 | 216.011 | 216.557 | 0.253 | 216.015 | 0.002 | 215.995 | 0.007 | 216.237 | 0.104 | 216.478 | 0.216 |
| 140.0 | 0.70 | 251.747 | 252.362 | 0.244 | 251.742 | 0.002 | 251.729 | 0.007 | 252.011 | 0.105 | 252.279 | 0.211 |
| 160.0 | 0.80 | 287.472 | 288.151 | 0.236 | 287.454 | 0.006 | 287.449 | 0.008 | 287.770 | 0.104 | 288.064 | 0.206 |
| 180.0 | 0.90 | 322.564 | 323.926 | 0.422 | 323.154 | 0.183 | 323.159 | 0.185 | 323.518 | 0.296 | 323.836 | 0.394 |
| $\kappa = 1.0$ | | | | | | | | | | | | |
| 10.0 | 0.05 | 10.890 | 10.930 | 0.363 | 10.920 | 0.275 | 10.894 | 0.035 | 10.887 | 0.031 | 10.912 | 0.206 |
| 20.0 | 0.09 | 21.194 | 21.290 | 0.455 | 21.217 | 0.110 | 21.200 | 0.027 | 21.204 | 0.048 | 21.256 | 0.291 |
| 40.0 | 0.18 | 41.575 | 41.779 | 0.490 | 41.602 | 0.065 | 41.584 | 0.023 | 41.629 | 0.129 | 41.720 | 0.348 |
| 60.0 | 0.28 | 61.854 | 62.143 | 0.467 | 61.877 | 0.037 | 61.856 | 0.003 | 61.944 | 0.146 | 62.067 | 0.344 |
| 80.0 | 0.37 | 82.074 | 82.445 | 0.453 | 82.098 | 0.029 | 82.073 | 0.001 | 82.205 | 0.160 | 82.357 | 0.344 |
| 100.0 | 0.46 | 102.265 | 102.709 | 0.434 | 102.284 | 0.019 | 102.259 | 0.006 | 102.432 | 0.163 | 102.610 | 0.337 |
| 120.0 | 0.55 | 122.429 | 122.945 | 0.421 | 122.446 | 0.014 | 122.422 | 0.005 | 122.634 | 0.168 | 122.837 | 0.334 |
| 140.0 | 0.64 | 142.582 | 143.161 | 0.406 | 142.589 | 0.005 | 142.570 | 0.009 | 142.819 | 0.166 | 143.046 | 0.325 |
| 160.0 | 0.74 | 162.715 | 163.360 | 0.396 | 162.717 | 0.001 | 162.704 | 0.007 | 162.990 | 0.169 | 163.239 | 0.322 |
| 180.0 | 0.83 | 182.839 | 183.546 | 0.387 | 182.834 | 0.003 | 182.829 | 0.006 | 183.149 | 0.170 | 183.419 | 0.317 |
| 200.0 | 0.92 | 202.358 | 203.722 | 0.674 | 202.941 | 0.288 | 202.945 | 0.290 | 203.299 | 0.465 | 203.590 | 0.609 |
| $\kappa = 1.2$ | | | | | | | | | | | | |
| 10.0 | 0.04 | 6.831 | 6.870 | 0.575 | 6.867 | 0.523 | 6.840 | 0.134 | 6.833 | 0.025 | 6.852 | 0.314 |
| 20.0 | 0.08 | 13.124 | 13.209 | 0.651 | 13.149 | 0.189 | 13.131 | 0.050 | 13.130 | 0.045 | 13.171 | 0.359 |
| 40.0 | 0.16 | 25.485 | 25.665 | 0.705 | 25.508 | 0.091 | 25.491 | 0.025 | 25.522 | 0.145 | 25.596 | 0.434 |
| 60.0 | 0.25 | 37.734 | 38.001 | 0.707 | 37.762 | 0.074 | 37.742 | 0.021 | 37.810 | 0.202 | 37.910 | 0.466 |
| 80.0 | 0.33 | 49.942 | 50.278 | 0.673 | 49.964 | 0.044 | 49.940 | 0.003 | 50.047 | 0.210 | 50.169 | 0.455 |
| 100.0 | 0.41 | 62.098 | 62.518 | 0.676 | 62.133 | 0.057 | 62.107 | 0.015 | 62.251 | 0.246 | 62.395 | 0.478 |
| 120.0 | 0.49 | 74.273 | 74.731 | 0.617 | 74.279 | 0.008 | 74.253 | 0.027 | 74.432 | 0.214 | 74.596 | 0.435 |
| 140.0 | 0.58 | 86.398 | 86.925 | 0.610 | 86.407 | 0.010 | 86.383 | 0.018 | 86.596 | 0.229 | 86.780 | 0.442 |
| 160.0 | 0.66 | 98.520 | 99.104 | 0.593 | 98.521 | 0.001 | 98.500 | 0.020 | 98.747 | 0.230 | 98.949 | 0.435 |
| 180.0 | 0.74 | 110.606 | 111.270 | 0.600 | 110.624 | 0.016 | 110.608 | 0.002 | 110.886 | 0.253 | 111.107 | 0.453 |
| 200.0 | 0.82 | 122.732 | 123.426 | 0.565 | 122.718 | 0.012 | 122.708 | 0.020 | 123.017 | 0.232 | 123.254 | 0.426 |

**Table 4c.** The reduced excess internal energy due to particle-particle interactions $u_{\mathrm{ex}}^{\mathrm{pp}}$ resulting from molecular dynamics simulations and five integral theory approaches: the hypernetted-chain approximation (HNC), isomorph-based empirically modified hypernetted-chain approximation (IEMHNC), variational modified hypernetted-chain approximation (VMHNC), Rogers-Young approximation (RY) and Ballone-Pastore-Galli-Gazzillo approximation (BPGG). The absolute relative deviation $\epsilon_{\mathrm{r}}$ between the theoretical and the simulation results is also reported. **Results for intermediate screening parameters**, *i.e.* $\kappa = \{1.4, 2.0, 2.6, 3.0\}$. The MD results are adopted from Table III of *S. Hamaguchi, R. T. Farouki and D. H. E. Dubin* ,Phys. Rev. E **56**, 4671 (1997) and from Table II of *S. Hamaguchi, R. T. Farouki and D. H. E. Dubin, J. Chem. Phys.* **105**, *7641 (1996).*

| $\Gamma$ | $\Gamma/\Gamma_{\mathrm{m}}$ | $u_{\mathrm{ex}}^{\mathrm{pp,MD}}$ | $u_{\mathrm{ex}}^{\mathrm{pp,HNC}}$ | $\epsilon_{\mathrm{r}}^{\mathrm{HNC}}(\%)$ | $u_{\mathrm{ex}}^{\mathrm{pp,IEMHNC}}$ | $\epsilon_{\mathrm{r}}^{\mathrm{IEMHNC}}(\%)$ | $u_{\mathrm{ex}}^{\mathrm{pp,VMHNC}}$ | $\epsilon_{\mathrm{r}}^{\mathrm{VMHNC}}(\%)$ | $u_{\mathrm{ex}}^{\mathrm{pp,RY}}$ | $\epsilon_{\mathrm{r}}^{\mathrm{RY}}(\%)$ | $u_{\mathrm{ex}}^{\mathrm{pp,BPGG}}$ | $\epsilon_{\mathrm{r}}^{\mathrm{BPGG}}(\%)$ |
|---|---|---|---|---|---|---|---|---|---|---|---|---|
| | | | | | | $\kappa = 1.4$ | | | | | | |
| 10.0 | 0.04 | 4.533 | 4.561 | 0.620 | 4.561 | 0.614 | 4.536 | 0.076 | 4.529 | 0.082 | 4.544 | 0.242 |
| 20.0 | 0.07 | 8.564 | 8.632 | 0.790 | 8.585 | 0.241 | 8.565 | 0.009 | 8.560 | 0.043 | 8.593 | 0.334 |
| 40.0 | 0.15 | 16.406 | 16.561 | 0.946 | 16.427 | 0.125 | 16.410 | 0.026 | 16.428 | 0.133 | 16.487 | 0.493 |
| 60.0 | 0.22 | 24.153 | 24.378 | 0.932 | 24.168 | 0.062 | 24.149 | 0.015 | 24.197 | 0.182 | 24.277 | 0.512 |
| 80.0 | 0.30 | 31.853 | 32.138 | 0.896 | 31.860 | 0.022 | 31.838 | 0.048 | 31.918 | 0.203 | 32.015 | 0.510 |
| 100.0 | 0.37 | 39.498 | 39.864 | 0.926 | 39.521 | 0.059 | 39.496 | 0.005 | 39.608 | 0.279 | 39.722 | 0.567 |
| 120.0 | 0.45 | 47.135 | 47.564 | 0.910 | 47.160 | 0.054 | 47.133 | 0.004 | 47.277 | 0.302 | 47.407 | 0.576 |
| 140.0 | 0.52 | 54.771 | 55.246 | 0.866 | 54.783 | 0.022 | 54.755 | 0.028 | 54.930 | 0.290 | 55.074 | 0.554 |
| 160.0 | 0.60 | 62.374 | 62.913 | 0.863 | 62.392 | 0.029 | 62.366 | 0.013 | 62.570 | 0.315 | 62.729 | 0.569 |
| 180.0 | 0.67 | 69.991 | 70.568 | 0.824 | 69.991 | 0.000 | 69.967 | 0.035 | 70.200 | 0.299 | 70.373 | 0.545 |
| 200.0 | 0.74 | 77.564 | 78.213 | 0.837 | 77.580 | 0.021 | 77.560 | 0.005 | 77.821 | 0.332 | 78.007 | 0.572 |
| 240.0 | 0.89 | 92.744 | 93.479 | 0.793 | 92.738 | 0.006 | 92.728 | 0.018 | 93.043 | 0.322 | 93.255 | 0.551 |
| | | | | | | $\kappa = 2.0$ | | | | | | |
| 20.0 | 0.09 | 2.944 | 2.983 | 1.324 | 2.976 | 1.091 | 2.947 | 0.113 | 2.940 | 0.136 | 2.954 | 0.324 |
| 40.0 | 0.18 | 5.343 | 5.430 | 1.627 | 5.361 | 0.333 | 5.342 | 0.025 | 5.336 | 0.130 | 5.364 | 0.401 |
| 60.0 | 0.28 | 7.630 | 7.785 | 2.037 | 7.662 | 0.421 | 7.645 | 0.201 | 7.648 | 0.234 | 7.688 | 0.758 |
| 80.0 | 0.37 | 9.903 | 10.095 | 1.938 | 9.923 | 0.198 | 9.905 | 0.022 | 9.920 | 0.170 | 9.969 | 0.666 |
| 100.0 | 0.46 | 12.133 | 12.376 | 2.000 | 12.158 | 0.204 | 12.138 | 0.045 | 12.168 | 0.284 | 12.224 | 0.752 |
| 200.0 | 0.92 | 23.107 | 23.554 | 1.935 | 23.137 | 0.130 | 23.107 | 0.000 | 23.221 | 0.492 | 23.303 | 0.848 |
| | | | | | | $\kappa = 2.6$ | | | | | | |
| 40.0 | 0.05 | 2.165 | 2.216 | 2.339 | 2.202 | 1.696 | 2.172 | 0.303 | 2.164 | 0.053 | 2.176 | 0.486 |
| 60.0 | 0.08 | 2.986 | 3.062 | 2.533 | 3.012 | 0.873 | 2.988 | 0.078 | 2.979 | 0.221 | 2.998 | 0.385 |
| 80.0 | 0.11 | 3.772 | 3.873 | 2.676 | 3.791 | 0.501 | 3.770 | 0.041 | 3.762 | 0.264 | 3.786 | 0.366 |
| 100.0 | 0.13 | 4.528 | 4.662 | 2.967 | 4.550 | 0.486 | 4.531 | 0.072 | 4.525 | 0.072 | 4.553 | 0.561 |
| 200.0 | 0.26 | 8.181 | 8.438 | 3.143 | 8.194 | 0.157 | 8.173 | 0.092 | 8.190 | 0.106 | 8.234 | 0.652 |
| 400.0 | 0.53 | 15.147 | 15.630 | 3.192 | 15.167 | 0.130 | 15.138 | 0.060 | 15.227 | 0.527 | 15.282 | 0.892 |
| 700.0 | 0.92 | 25.319 | 26.080 | 3.006 | 25.322 | 0.011 | 25.304 | 0.059 | 25.518 | 0.788 | 25.574 | 1.006 |
| | | | | | | $\kappa = 3.0$ | | | | | | |
| 40.0 | 0.03 | 1.322 | 1.345 | 1.766 | 1.345 | 1.766 | 1.319 | 0.211 | 1.314 | 0.624 | 1.320 | 0.171 |
| 60.0 | 0.05 | 1.769 | 1.810 | 2.319 | 1.798 | 1.613 | 1.765 | 0.207 | 1.758 | 0.636 | 1.768 | 0.083 |
| 80.0 | 0.07 | 2.189 | 2.247 | 2.644 | 2.211 | 1.012 | 2.183 | 0.262 | 2.174 | 0.675 | 2.188 | 0.062 |
| 100.0 | 0.08 | 2.582 | 2.666 | 3.261 | 2.608 | 1.021 | 2.584 | 0.064 | 2.574 | 0.319 | 2.591 | 0.332 |
| 200.0 | 0.17 | 4.456 | 4.625 | 3.790 | 4.470 | 0.312 | 4.451 | 0.110 | 4.444 | 0.267 | 4.474 | 0.403 |
| 400.0 | 0.34 | 7.928 | 8.253 | 4.095 | 7.938 | 0.120 | 7.916 | 0.157 | 7.935 | 0.083 | 7.977 | 0.616 |
| 700.0 | 0.59 | 12.869 | 13.420 | 4.282 | 12.897 | 0.214 | 12.873 | 0.031 | 12.952 | 0.644 | 12.996 | 0.986 |

**Table 4d.** The reduced excess internal energy due to particle-particle interactions $u_{\rm ex}^{\rm pp}$ resulting from molecular dynamics simulations and five integral theory approaches: the hypernetted-chain approximation (HNC), isomorph-based empirically modified hypernetted-chain approximation (IEMHNC), variational modified hypernetted-chain approximation (VMHNC), Rogers-Young approximation (RY) and Ballone-Pastore-Galli-Gazzillo approximation (BPGG). The absolute relative deviation $\epsilon_{\rm r}$ between the theoretical and the simulation results is also reported. **Results for high screening parameters**, *i.e.* $\kappa = \{3.6, 4.0, 4.6, 5.0\}$. The MD results are adopted from Table III of *S. Hamaguchi, R. T. Farouki and D. H. E. Dubin ,Phys. Rev. E* **56**, *4671 (1997)*.

| $\Gamma$ | $\Gamma/\Gamma_{\rm m}$ | $u_{\rm ex}^{\rm pp,MD}$ | $u_{\rm ex}^{\rm pp,HNC}$ | $\epsilon_{\rm r}^{\rm HNC}(\%)$ | $u_{\rm ex}^{\rm pp,IEMHNC}$ | $\epsilon_{\rm r}^{\rm IEMHNC}(\%)$ | $u_{\rm ex}^{\rm pp,VMHNC}$ | $\epsilon_{\rm r}^{\rm VMHNC}(\%)$ | $u_{\rm ex}^{\rm pp,RY}$ | $\epsilon_{\rm r}^{\rm RY}(\%)$ | $u_{\rm ex}^{\rm pp,BPGG}$ | $\epsilon_{\rm r}^{\rm BPGG}(\%)$ |
|---|---|---|---|---|---|---|---|---|---|---|---|---|
| $\kappa = 3.6$ | | | | | | | | | | | | |
| 80.0 | 0.03 | 1.092 | 1.126 | 3.135 | 1.126 | 3.135 | 1.097 | 0.443 | 1.092 | 0.038 | 1.097 | 0.432 |
| 100.0 | 0.04 | 1.272 | 1.308 | 2.809 | 1.304 | 2.540 | 1.269 | 0.238 | 1.263 | 0.744 | 1.269 | 0.218 |
| 200.0 | 0.08 | 2.035 | 2.119 | 4.145 | 2.062 | 1.304 | 2.034 | 0.070 | 2.023 | 0.590 | 2.037 | 0.092 |
| 400.0 | 0.17 | 3.378 | 3.541 | 4.830 | 3.386 | 0.248 | 3.366 | 0.350 | 3.354 | 0.711 | 3.379 | 0.022 |
| 700.0 | 0.29 | 5.200 | 5.483 | 5.445 | 5.205 | 0.090 | 5.187 | 0.254 | 5.183 | 0.335 | 5.216 | 0.316 |
| 1000.0 | 0.42 | 6.934 | 7.320 | 5.564 | 6.930 | 0.053 | 6.914 | 0.295 | 6.925 | 0.135 | 6.962 | 0.402 |
| 2000.0 | 0.84 | 12.399 | 13.108 | 5.719 | 12.382 | 0.139 | 12.387 | 0.094 | 12.476 | 0.621 | 12.503 | 0.840 |
| $\kappa = 4.0$ | | | | | | | | | | | | |
| 200.0 | 0.05 | 1.305 | 1.360 | 4.223 | 1.345 | 3.027 | 1.308 | 0.230 | 1.300 | 0.347 | 1.308 | 0.241 |
| 400.0 | 0.10 | 2.066 | 2.173 | 5.163 | 2.091 | 1.223 | 2.064 | 0.106 | 2.052 | 0.692 | 2.067 | 0.039 |
| 700.0 | 0.18 | 3.054 | 3.245 | 6.240 | 3.077 | 0.744 | 3.056 | 0.077 | 3.042 | 0.391 | 3.066 | 0.377 |
| 1000.0 | 0.26 | 3.971 | 4.236 | 6.664 | 3.991 | 0.497 | 3.974 | 0.071 | 3.961 | 0.248 | 3.990 | 0.485 |
| 2000.0 | 0.52 | 6.824 | 7.282 | 6.710 | 6.810 | 0.209 | 6.804 | 0.295 | 6.812 | 0.171 | 6.848 | 0.345 |
| $\kappa = 4.6$ | | | | | | | | | | | | |
| 400.0 | 0.05 | 1.114 | 1.161 | 4.205 | 1.148 | 3.089 | 1.109 | 0.486 | 1.102 | 1.110 | 1.108 | 0.534 |
| 700.0 | 0.08 | 1.553 | 1.645 | 5.896 | 1.586 | 2.113 | 1.552 | 0.038 | 1.542 | 0.731 | 1.553 | 0.019 |
| 1000.0 | 0.12 | 1.947 | 2.075 | 6.553 | 1.973 | 1.325 | 1.945 | 0.121 | 1.931 | 0.814 | 1.946 | 0.039 |
| 2000.0 | 0.23 | 3.119 | 3.338 | 7.035 | 3.110 | 0.292 | 3.094 | 0.810 | 3.076 | 1.370 | 3.101 | 0.573 |
| 3000.0 | 0.35 | 4.126 | 4.477 | 8.508 | 4.136 | 0.249 | 4.130 | 0.088 | 4.113 | 0.304 | 4.144 | 0.433 |
| 4000.0 | 0.46 | 5.118 | 5.551 | 8.457 | 5.104 | 0.265 | 5.109 | 0.176 | 5.098 | 0.398 | 5.131 | 0.245 |
| 5000.0 | 0.58 | 6.047 | 6.583 | 8.867 | 6.035 | 0.199 | 6.053 | 0.100 | 6.049 | 0.039 | 6.082 | 0.585 |
| 6000.0 | 0.70 | 6.969 | 7.586 | 8.855 | 6.939 | 0.432 | 6.973 | 0.051 | 6.979 | 0.142 | 7.010 | 0.591 |
| $\kappa = 5.0$ | | | | | | | | | | | | |
| 700.0 | 0.05 | 1.067 | 1.117 | 4.656 | 1.101 | 3.191 | 1.060 | 0.683 | 1.053 | 1.342 | 1.059 | 0.753 |
| 1000.0 | 0.07 | 1.295 | 1.379 | 6.501 | 1.336 | 3.175 | 1.298 | 0.269 | 1.289 | 0.455 | 1.298 | 0.229 |
| 2000.0 | 0.13 | 1.978 | 2.126 | 7.487 | 1.999 | 1.073 | 1.972 | 0.280 | 1.957 | 1.037 | 1.974 | 0.226 |
| 3000.0 | 0.20 | 2.568 | 2.779 | 8.219 | 2.577 | 0.360 | 2.559 | 0.344 | 2.541 | 1.053 | 2.562 | 0.217 |
| 4000.0 | 0.27 | 3.108 | 3.384 | 8.866 | 3.112 | 0.141 | 3.102 | 0.192 | 3.082 | 0.830 | 3.108 | 0.006 |
| 5000.0 | 0.33 | 3.625 | 3.957 | 9.160 | 3.620 | 0.140 | 3.617 | 0.207 | 3.597 | 0.764 | 3.626 | 0.026 |
| 6000.0 | 0.40 | 4.140 | 4.509 | 8.902 | 4.108 | 0.783 | 4.114 | 0.634 | 4.094 | 1.104 | 4.125 | 0.362 |
| 8000.0 | 0.53 | 5.072 | 5.565 | 9.717 | 5.041 | 0.620 | 5.066 | 0.109 | 5.051 | 0.414 | 5.084 | 0.229 |
| 10000.0 | 0.66 | 5.900 | 6.577 | 11.481 | 5.934 | 0.571 | 5.982 | 1.395 | 5.974 | 1.252 | 6.006 | 1.794 |

**Table 5a.** Test of the thermodynamic consistency of the isomorph-based empirically modified hypernetted-chain approximation (IEMHNC) and the variational modified hypernetted-chain approximation (VMHNC); the reduced excess inverse isothermal compressibility due to the particle presence resulting from the statistical route $\mu^{\mathrm{p}}_{\mathrm{stat}}$ and the virial route $\mu^{\mathrm{p}}_{\mathrm{vir}}$. The absolute relative deviation between the two thermodynamic paths is also reported. **Results for $\boldsymbol{\kappa = 0.0}$.**

| $\Gamma$ | $\Gamma/\Gamma_{\mathrm{m}}$ | $\mu^{\mathrm{p,IEMHNC}}_{\mathrm{stat}}$ | $\mu^{\mathrm{p,IEMHNC}}_{\mathrm{vir}}$ | deviation (%) | $\mu^{\mathrm{p,VMHNC}}_{\mathrm{stat}}$ | $\mu^{\mathrm{p,VMHNC}}_{\mathrm{vir}}$ | deviation (%) |
|---|---|---|---|---|---|---|---|
| 10.0 | 0.06 | -4.047 | -3.609 | 12.112 | -3.890 | -3.616 | 7.583 |
| 20.0 | 0.12 | -7.289 | -7.488 | 2.660 | -7.920 | -7.495 | 5.666 |
| 30.0 | 0.17 | -10.850 | -11.402 | 4.843 | -11.911 | -11.411 | 4.383 |
| 40.0 | 0.23 | -14.804 | -15.333 | 3.449 | -15.883 | -15.343 | 3.520 |
| 50.0 | 0.29 | -19.018 | -19.275 | 1.333 | -19.851 | -19.286 | 2.930 |
| 60.0 | 0.35 | -23.407 | -23.224 | 0.789 | -23.820 | -23.234 | 2.523 |
| 70.0 | 0.41 | -27.924 | -27.179 | 2.743 | -27.797 | -27.187 | 2.241 |
| 80.0 | 0.47 | -32.540 | -31.137 | 4.505 | -31.782 | -31.144 | 2.048 |
| 90.0 | 0.52 | -37.235 | -35.098 | 6.089 | -35.776 | -35.101 | 1.922 |
| 100.0 | 0.58 | -41.995 | -39.057 | 7.523 | -39.780 | -39.058 | 1.848 |
| 110.0 | 0.64 | -46.811 | -43.011 | 8.835 | -43.792 | -43.012 | 1.814 |
| 120.0 | 0.70 | -51.675 | -46.957 | 10.047 | -47.813 | -46.962 | 1.812 |
| 130.0 | 0.76 | -56.582 | -50.892 | 11.182 | -51.841 | -50.906 | 1.837 |
| 140.0 | 0.81 | -61.527 | -54.810 | 12.256 | -55.876 | -54.844 | 1.882 |
| 150.0 | 0.87 | -66.506 | -58.709 | 13.282 | -59.916 | -58.774 | 1.942 |
| 160.0 | 0.93 | -71.516 | -62.585 | 14.271 | -63.961 | -62.698 | 2.015 |

**Table 5b.** Test of the thermodynamic consistency of the isomorph-based empirically modified hypernetted-chain approximation (IEMHNC) and the variational modified hypernetted-chain approximation (VMHNC); the reduced excess inverse isothermal compressibility due to the particle presence resulting from the statistical route $\mu^{\mathrm{p}}_{\mathrm{stat}}$ and the virial route $\mu^{\mathrm{p}}_{\mathrm{vir}}$. The absolute relative deviation between the two thermodynamic paths is also reported. **Results for $\boldsymbol{\kappa = 1.0}$.**

| $\Gamma$ | $\Gamma/\Gamma_{\mathrm{m}}$ | $\mu^{\mathrm{p,IEMHNC}}_{\mathrm{stat}}$ | $\mu^{\mathrm{p,IEMHNC}}_{\mathrm{vir}}$ | deviation (%) | $\mu^{\mathrm{p,VMHNC}}_{\mathrm{stat}}$ | $\mu^{\mathrm{p,VMHNC}}_{\mathrm{vir}}$ | deviation (%) |
|---|---|---|---|---|---|---|---|
| 20.0 | 0.09 | -6.938 | -6.912 | 0.375 | -7.303 | -6.915 | 5.613 |
| 30.0 | 0.14 | -10.141 | -10.582 | 4.168 | -11.105 | -10.587 | 4.894 |
| 40.0 | 0.18 | -13.637 | -14.274 | 4.461 | -14.896 | -14.280 | 4.313 |
| 50.0 | 0.23 | -17.368 | -17.977 | 3.387 | -18.680 | -17.985 | 3.862 |
| 60.0 | 0.28 | -21.268 | -21.690 | 1.944 | -22.461 | -21.699 | 3.513 |
| 70.0 | 0.32 | -25.292 | -25.410 | 0.464 | -26.242 | -25.418 | 3.242 |
| 80.0 | 0.37 | -29.409 | -29.134 | 0.944 | -30.025 | -29.142 | 3.031 |
| 90.0 | 0.41 | -33.602 | -32.864 | 2.247 | -33.812 | -32.869 | 2.867 |
| 100.0 | 0.46 | -37.856 | -36.597 | 3.441 | -37.602 | -36.600 | 2.738 |
| 110.0 | 0.51 | -42.162 | -40.333 | 4.536 | -41.397 | -40.332 | 2.641 |
| 120.0 | 0.55 | -46.513 | -44.071 | 5.539 | -45.197 | -44.068 | 2.562 |
| 130.0 | 0.60 | -50.902 | -47.813 | 6.461 | -49.002 | -47.806 | 2.501 |
| 140.0 | 0.64 | -55.326 | -51.556 | 7.313 | -52.810 | -51.545 | 2.456 |
| 150.0 | 0.69 | -59.780 | -55.300 | 8.101 | -56.673 | -55.284 | 2.512 |
| 160.0 | 0.74 | -64.263 | -59.047 | 8.834 | -60.440 | -59.024 | 2.398 |
| 170.0 | 0.78 | -68.771 | -62.795 | 9.517 | -64.260 | -62.767 | 2.378 |
| 180.0 | 0.83 | -73.302 | -66.544 | 10.156 | -68.083 | -66.511 | 2.363 |
| 190.0 | 0.87 | -77.854 | -70.294 | 10.755 | -71.909 | -70.258 | 2.349 |
| 200.0 | 0.92 | -82.426 | -74.045 | 11.319 | -75.737 | -74.005 | 2.342 |

**Table 5c.** Test of the thermodynamic consistency of the isomorph-based empirically modified hypernetted-chain approximation (IEMHNC) and the variational modified hypernetted-chain approximation (VMHNC); the reduced excess inverse isothermal compressibility due to the particle presence resulting from the statistical route $\mu^{\mathrm{p}}_{\mathrm{stat}}$ and the virial route $\mu^{\mathrm{p}}_{\mathrm{vir}}$. The absolute relative deviation between the two thermodynamic paths is also reported. **Results for $\boldsymbol{\kappa = 2.0}$**.

| $\Gamma$ | $\Gamma/\Gamma_{\mathrm{m}}$ | $\mu^{\mathrm{p,IEMHNC}}_{\mathrm{stat}}$ | $\mu^{\mathrm{p,IEMHNC}}_{\mathrm{vir}}$ | deviation (%) | $\mu^{\mathrm{p,VMHNC}}_{\mathrm{stat}}$ | $\mu^{\mathrm{p,VMHNC}}_{\mathrm{vir}}$ | deviation (%) |
|---|---|---|---|---|---|---|---|
| 40.0 | 0.09 | -11.489 | -11.384 | 0.914 | -11.781 | -11.378 | 3.549 |
| 60.0 | 0.14 | -17.175 | -17.473 | 1.702 | -18.073 | -17.473 | 3.433 |
| 80.0 | 0.18 | -23.165 | -23.602 | 1.851 | -24.387 | -23.610 | 3.289 |
| 100.0 | 0.23 | -29.405 | -29.756 | 1.178 | -30.711 | -29.772 | 3.154 |
| 120.0 | 0.27 | -35.826 | -35.928 | 0.283 | -37.041 | -35.948 | 3.039 |
| 140.0 | 0.32 | -42.380 | -42.113 | 0.633 | -43.377 | -42.136 | 2.943 |
| 160.0 | 0.36 | -49.036 | -48.310 | 1.502 | -49.717 | -48.333 | 2.864 |
| 180.0 | 0.41 | -55.773 | -54.516 | 2.306 | -56.063 | -54.537 | 2.797 |
| 200.0 | 0.45 | -62.576 | -60.729 | 3.042 | -62.412 | -60.749 | 2.738 |
| 220.0 | 0.50 | -69.436 | -66.948 | 3.716 | -68.767 | -66.964 | 2.693 |
| 240.0 | 0.55 | -76.343 | -73.173 | 4.333 | -75.125 | -73.182 | 2.655 |
| 260.0 | 0.59 | -83.293 | -79.402 | 4.900 | -81.488 | -79.404 | 2.624 |
| 280.0 | 0.64 | -90.280 | -85.636 | 5.423 | -87.854 | -85.629 | 2.598 |
| 300.0 | 0.68 | -97.300 | -91.865 | 5.917 | -94.223 | -91.858 | 2.575 |
| 320.0 | 0.73 | -104.350 | -98.112 | 6.358 | -100.595 | -98.087 | 2.557 |
| 340.0 | 0.77 | -111.427 | -104.355 | 6.777 | -106.970 | -104.320 | 2.541 |
| 360.0 | 0.82 | -118.529 | -110.600 | 7.169 | -113.347 | -110.555 | 2.525 |
| 380.0 | 0.86 | -125.653 | -116.846 | 7.537 | -119.726 | -116.791 | 2.513 |
| 400.0 | 0.91 | -132.799 | -123.095 | 7.883 | -126.107 | -123.030 | 2.501 |

**Table 5d.** Test of the thermodynamic consistency of the isomorph-based empirically modified hypernetted-chain approximation (IEMHNC) and the variational modified hypernetted-chain approximation (VMHNC); the reduced excess inverse isothermal compressibility due to the particle presence resulting from the statistical route $\mu^{\mathrm{p}}_{\mathrm{stat}}$ and the virial route $\mu^{\mathrm{p}}_{\mathrm{vir}}$. The absolute relative deviation between the two thermodynamic paths is also reported. **Results for $\boldsymbol{\kappa = 3.0}$**.

| $\Gamma$ | $\Gamma/\Gamma_{\mathrm{m}}$ | $\mu^{\mathrm{p,IEMHNC}}_{\mathrm{stat}}$ | $\mu^{\mathrm{p,IEMHNC}}_{\mathrm{vir}}$ | deviation (%) | $\mu^{\mathrm{p,VMHNC}}_{\mathrm{stat}}$ | $\mu^{\mathrm{p,VMHNC}}_{\mathrm{vir}}$ | deviation (%) |
|---|---|---|---|---|---|---|---|
| 40.0 | 0.03 | -8.297 | -7.889 | 5.173 | -8.096 | -7.972 | 1.559 |
| 60.0 | 0.05 | -12.855 | -12.385 | 3.797 | -12.590 | -12.382 | 1.676 |
| 80.0 | 0.07 | -17.255 | -16.875 | 2.248 | -17.144 | -16.851 | 1.739 |
| 100.0 | 0.08 | -21.606 | -21.380 | 1.058 | -21.735 | -21.356 | 1.775 |
| 200.0 | 0.17 | -43.831 | -44.150 | 0.723 | -44.949 | -44.146 | 1.818 |
| 400.0 | 0.34 | -90.856 | -90.204 | 0.723 | -91.830 | -90.244 | 1.757 |
| 700.0 | 0.59 | -163.998 | -159.799 | 2.628 | -162.515 | -159.803 | 1.697 |

**Table 5e.** Test of the thermodynamic consistency of the isomorph-based empirically modified hypernetted-chain approximation (IEMHNC) and the variational modified hypernetted-chain approximation (VMHNC); the reduced excess inverse isothermal compressibility due to the particle presence resulting from the statistical route $\mu^{\mathrm{p}}_{\mathrm{stat}}$ and the virial route $\mu^{\mathrm{p}}_{\mathrm{vir}}$. The absolute relative deviation between the two thermodynamic paths is also reported. **Results for $\boldsymbol{\kappa = 4.0}$**.

| $\Gamma$ | $\Gamma/\Gamma_{\mathrm{m}}$ | $\mu^{\mathrm{p,IEMHNC}}_{\mathrm{stat}}$ | $\mu^{\mathrm{p,IEMHNC}}_{\mathrm{vir}}$ | deviation (%) | $\mu^{\mathrm{p,VMHNC}}_{\mathrm{stat}}$ | $\mu^{\mathrm{p,VMHNC}}_{\mathrm{vir}}$ | deviation (%) |
|---|---|---|---|---|---|---|---|
| 200.0 | 0.05 | -30.831 | -30.295 | 1.767 | -30.509 | -30.285 | 0.740 |
| 400.0 | 0.10 | -62.370 | -62.317 | 0.086 | -62.770 | -62.274 | 0.796 |
| 700.0 | 0.18 | -110.465 | -110.779 | 0.284 | -111.652 | -110.750 | 0.815 |
| 1000.0 | 0.26 | -159.452 | -159.491 | 0.025 | -160.783 | -159.479 | 0.818 |
| 2000.0 | 0.52 | -325.562 | -322.726 | 0.879 | -325.271 | -322.650 | 0.812 |

**Table 5f.** Test of the thermodynamic consistency of the isomorph-based empirically modified hypernetted-chain approximation (IEMHNC) and the variational modified hypernetted-chain approximation (VMHNC); the reduced excess inverse isothermal compressibility due to the particle presence resulting from the statistical route $\mu^{\mathrm{p}}_{\mathrm{stat}}$ and the virial route $\mu^{\mathrm{p}}_{\mathrm{vir}}$. The absolute relative deviation between the two thermodynamic paths is also reported. **Results for $\boldsymbol{\kappa = 5.0}$.**

| $\Gamma$ | $\Gamma/\Gamma_{\mathrm{m}}$ | $\mu^{\mathrm{p,IEMHNC}}_{\mathrm{stat}}$ | $\mu^{\mathrm{p,IEMHNC}}_{\mathrm{vir}}$ | deviation (%) | $\mu^{\mathrm{p,VMHNC}}_{\mathrm{stat}}$ | $\mu^{\mathrm{p,VMHNC}}_{\mathrm{vir}}$ | deviation (%) |
|---|---|---|---|---|---|---|---|
| 700.0 | 0.05 | -77.425 | -76.788 | 0.829 | -77.017 | -76.786 | 0.300 |
| 1000.0 | 0.07 | -111.099 | -110.654 | 0.402 | -110.954 | -110.613 | 0.309 |
| 2000.0 | 0.13 | -223.832 | -224.104 | 0.121 | -224.720 | -224.008 | 0.318 |
| 3000.0 | 0.20 | -337.621 | -337.986 | 0.108 | -338.945 | -337.865 | 0.320 |
| 4000.0 | 0.27 | -452.043 | -452.111 | 0.015 | -453.398 | -451.945 | 0.322 |
| 5000.0 | 0.33 | -566.851 | -566.400 | 0.080 | -567.993 | -566.181 | 0.320 |
| 6000.0 | 0.40 | -681.927 | -680.808 | 0.164 | -682.686 | -680.509 | 0.320 |
| 8000.0 | 0.53 | -912.631 | -909.868 | 0.304 | -912.268 | -909.373 | 0.318 |
| 10000.0 | 0.66 | -1143.855 | -1139.142 | 0.414 | -1142.027 | -1138.415 | 0.317 |
